# Supplementary material for: Augmentations in Graph Contrastive Learning: Current Methodological Flaws & Towards Better Practices
Source: arXiv:2111.03220 source file (2022-03-11)
Supplement: Supplementary file 1 [file training_figures_nlp.tex]

\subsection{SimSiam}\label{app_text_simsiam}
In this section, we report our training setup for document classification using SimSiam (\cite{Chen20_SimSiam}), a positive-sample-only framework. We use the hyper-parameters discussed in Sec.\ref{sec:app_doc}. Further, in Figs. (\ref{fig:simsiam_nlp_ws2}, \ref{fig:simsiam_nlp_ws2_sub10_v_node10}, \ref{fig:simsiam_nlp_ws2_sub10_v_sub10}, \ref{fig:simsiam_nlp_ws4}, \ref{fig:simsiam_nlp_ws4_sub10_v_node10}, \ref{fig:simsiam_nlp_ws4_sub10_v_sub10}), we plot KNN accuracy and loss as well as the norm, standard deviation, and similarity of backbone, encoder, and projector representations throughout training. 
\begin{figure}[H]
    \centering
    \includegraphics[width=0.8\textwidth]{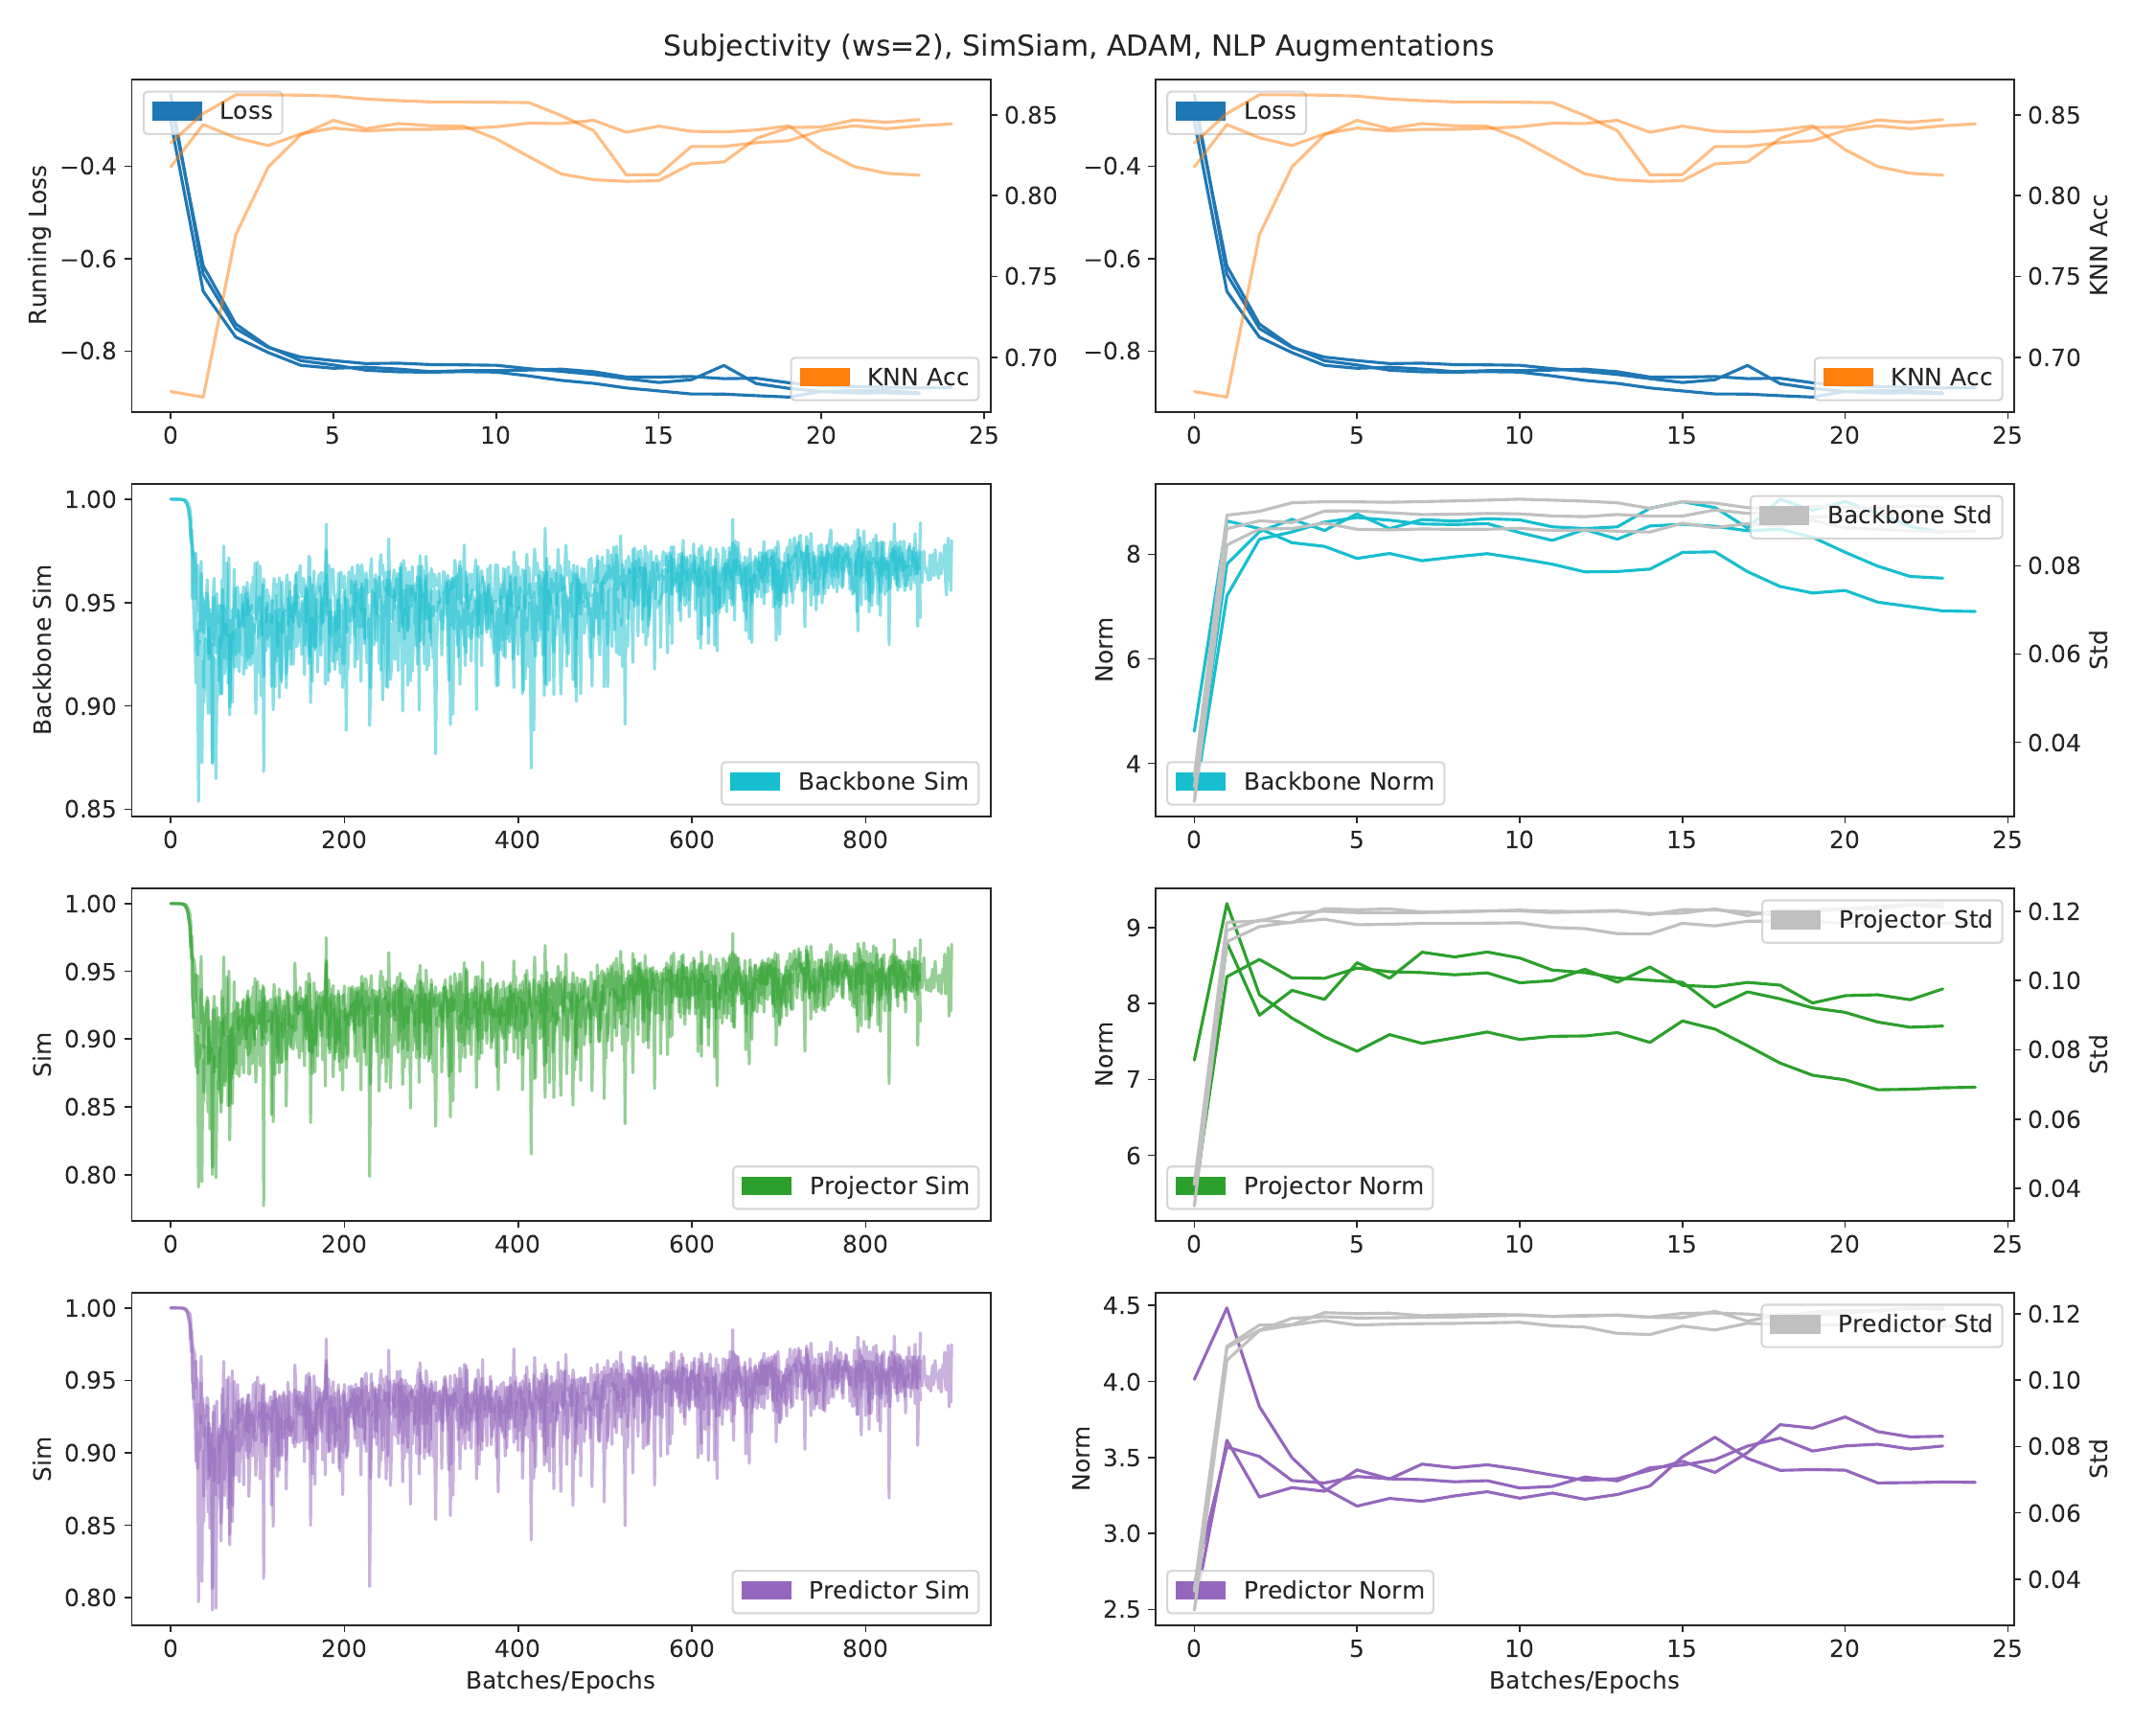}
    \caption{SimSiam, WS=2, NLP Augmentations}
    \label{fig:simsiam_nlp_ws2}
\end{figure}
\begin{figure}[H]
    \centering
    \includegraphics[width=0.8\textwidth]{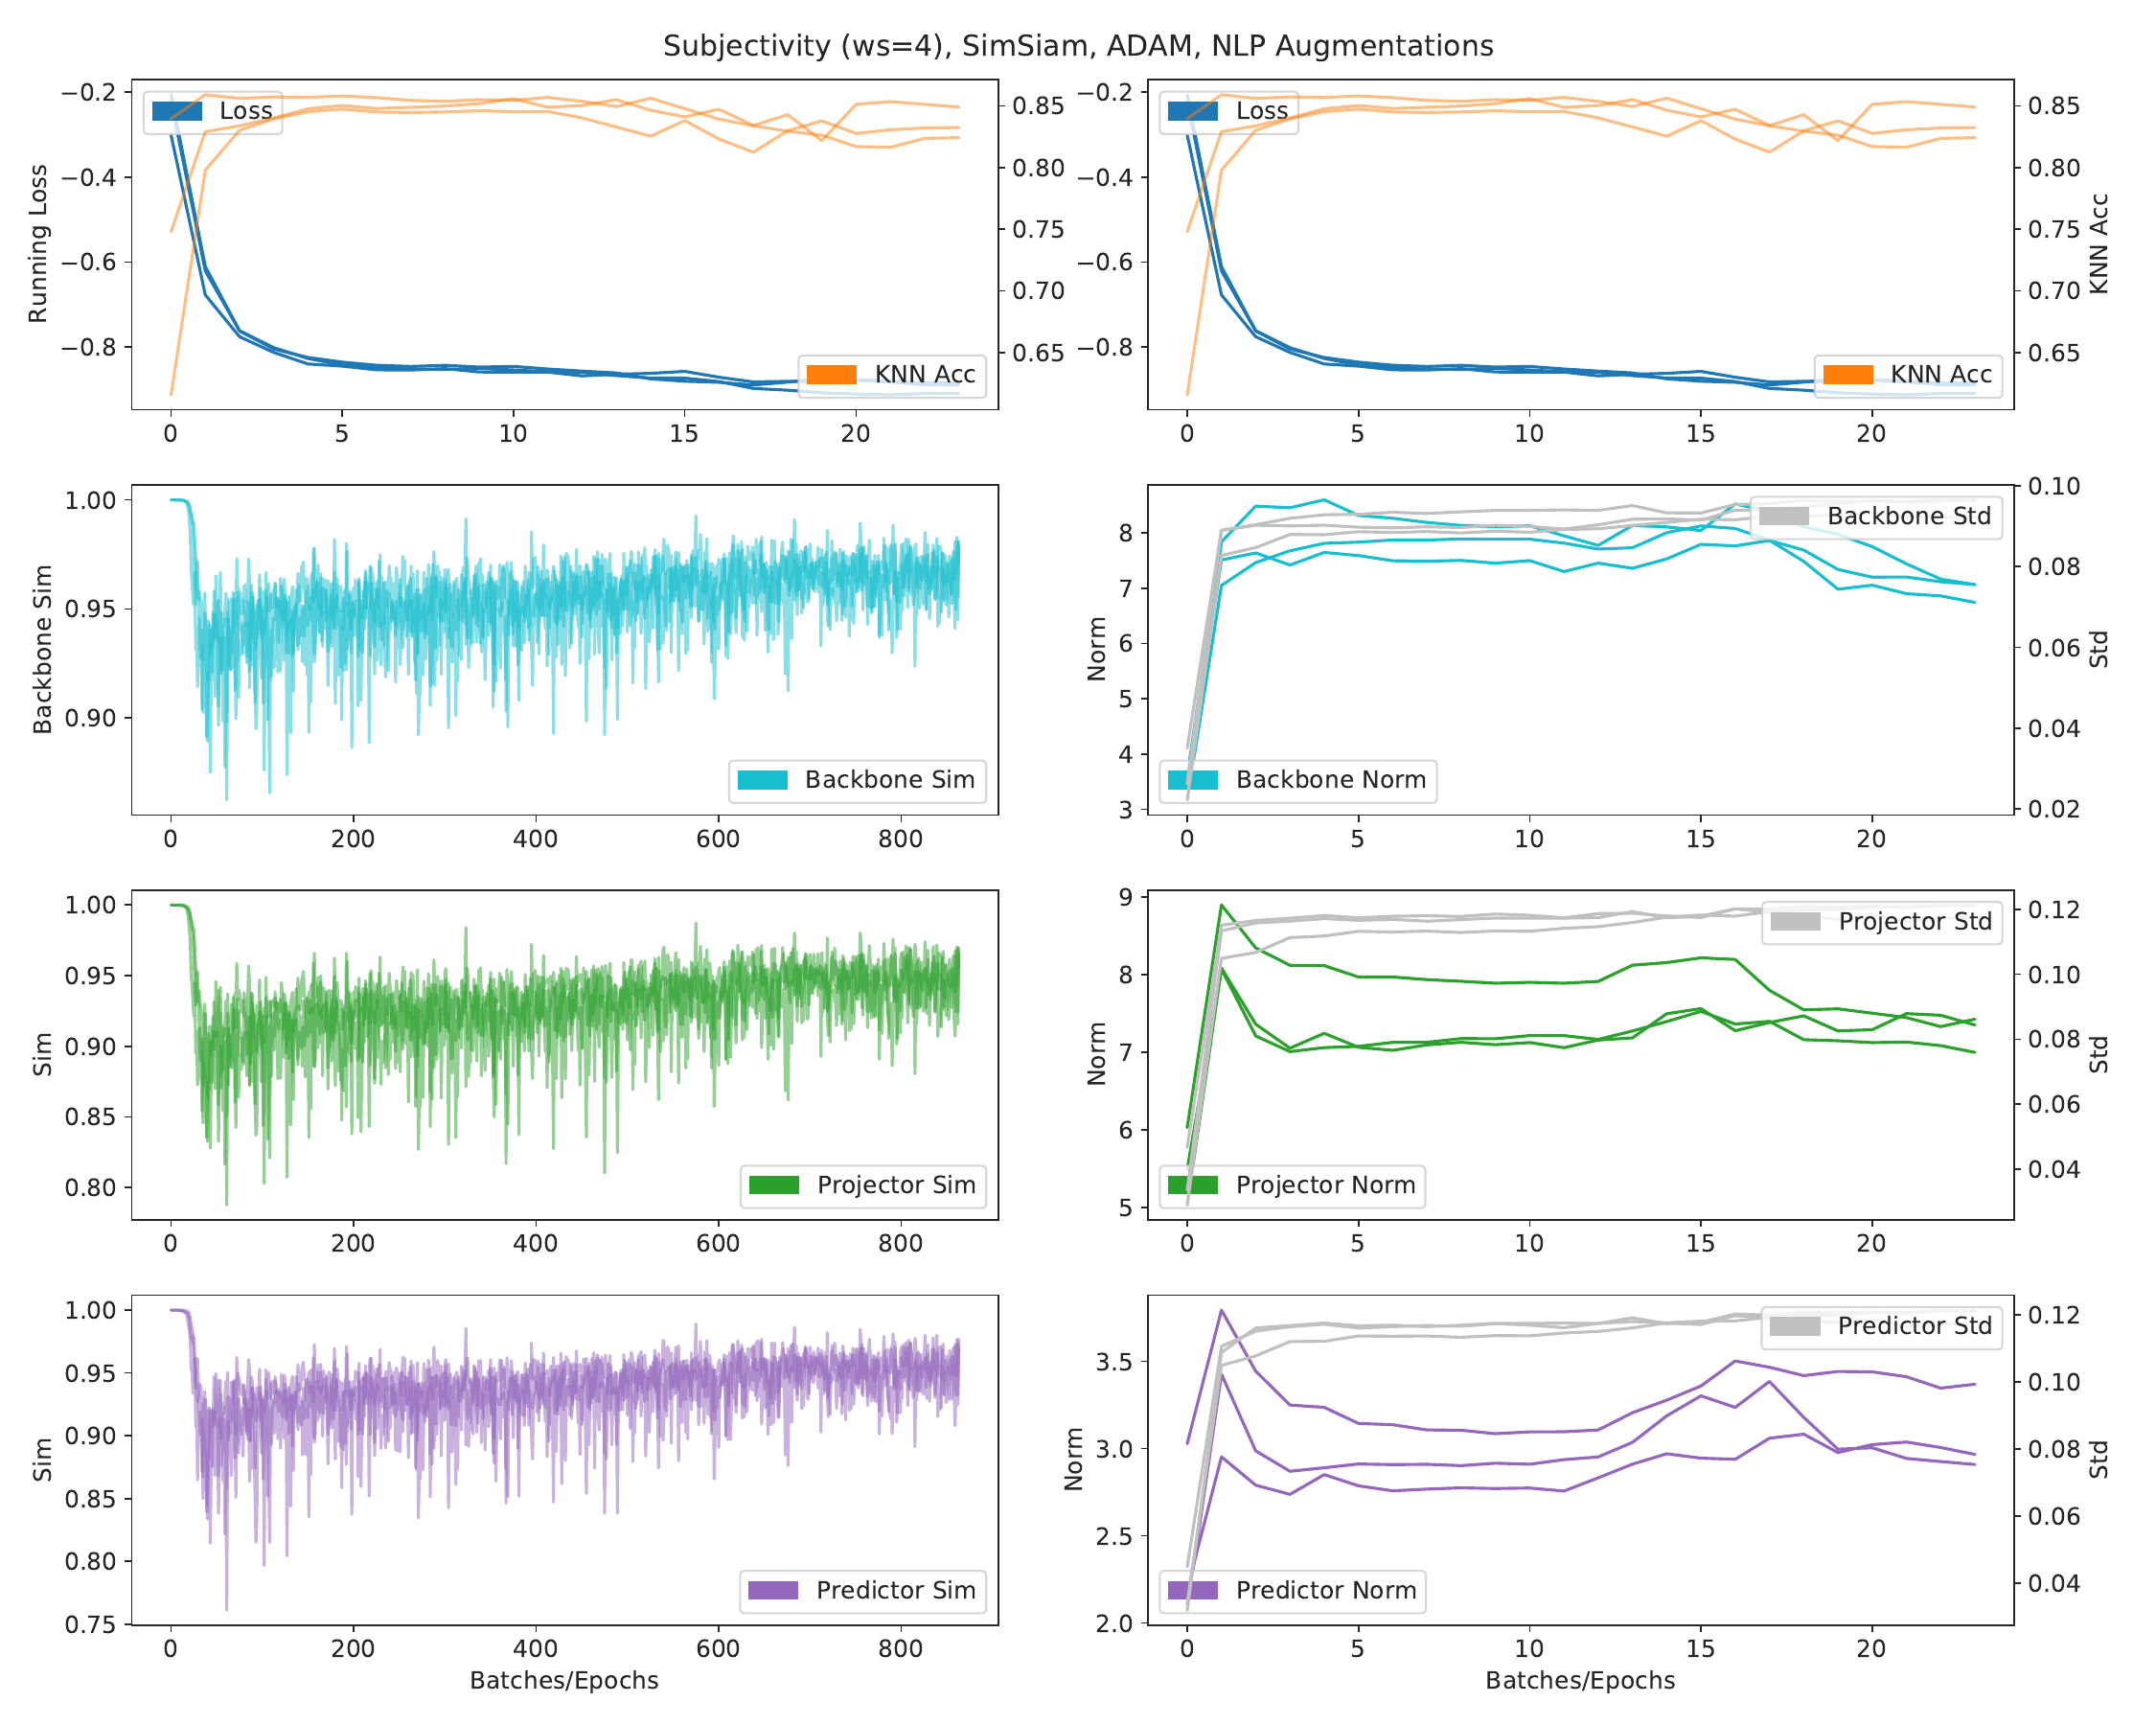}
    \caption{SimSiam, WS=4, NLP Augmentations}
    \label{fig:simsiam_nlp_ws4}
\end{figure}
\begin{figure}[H]
    \centering
    \includegraphics[width=0.8\textwidth]{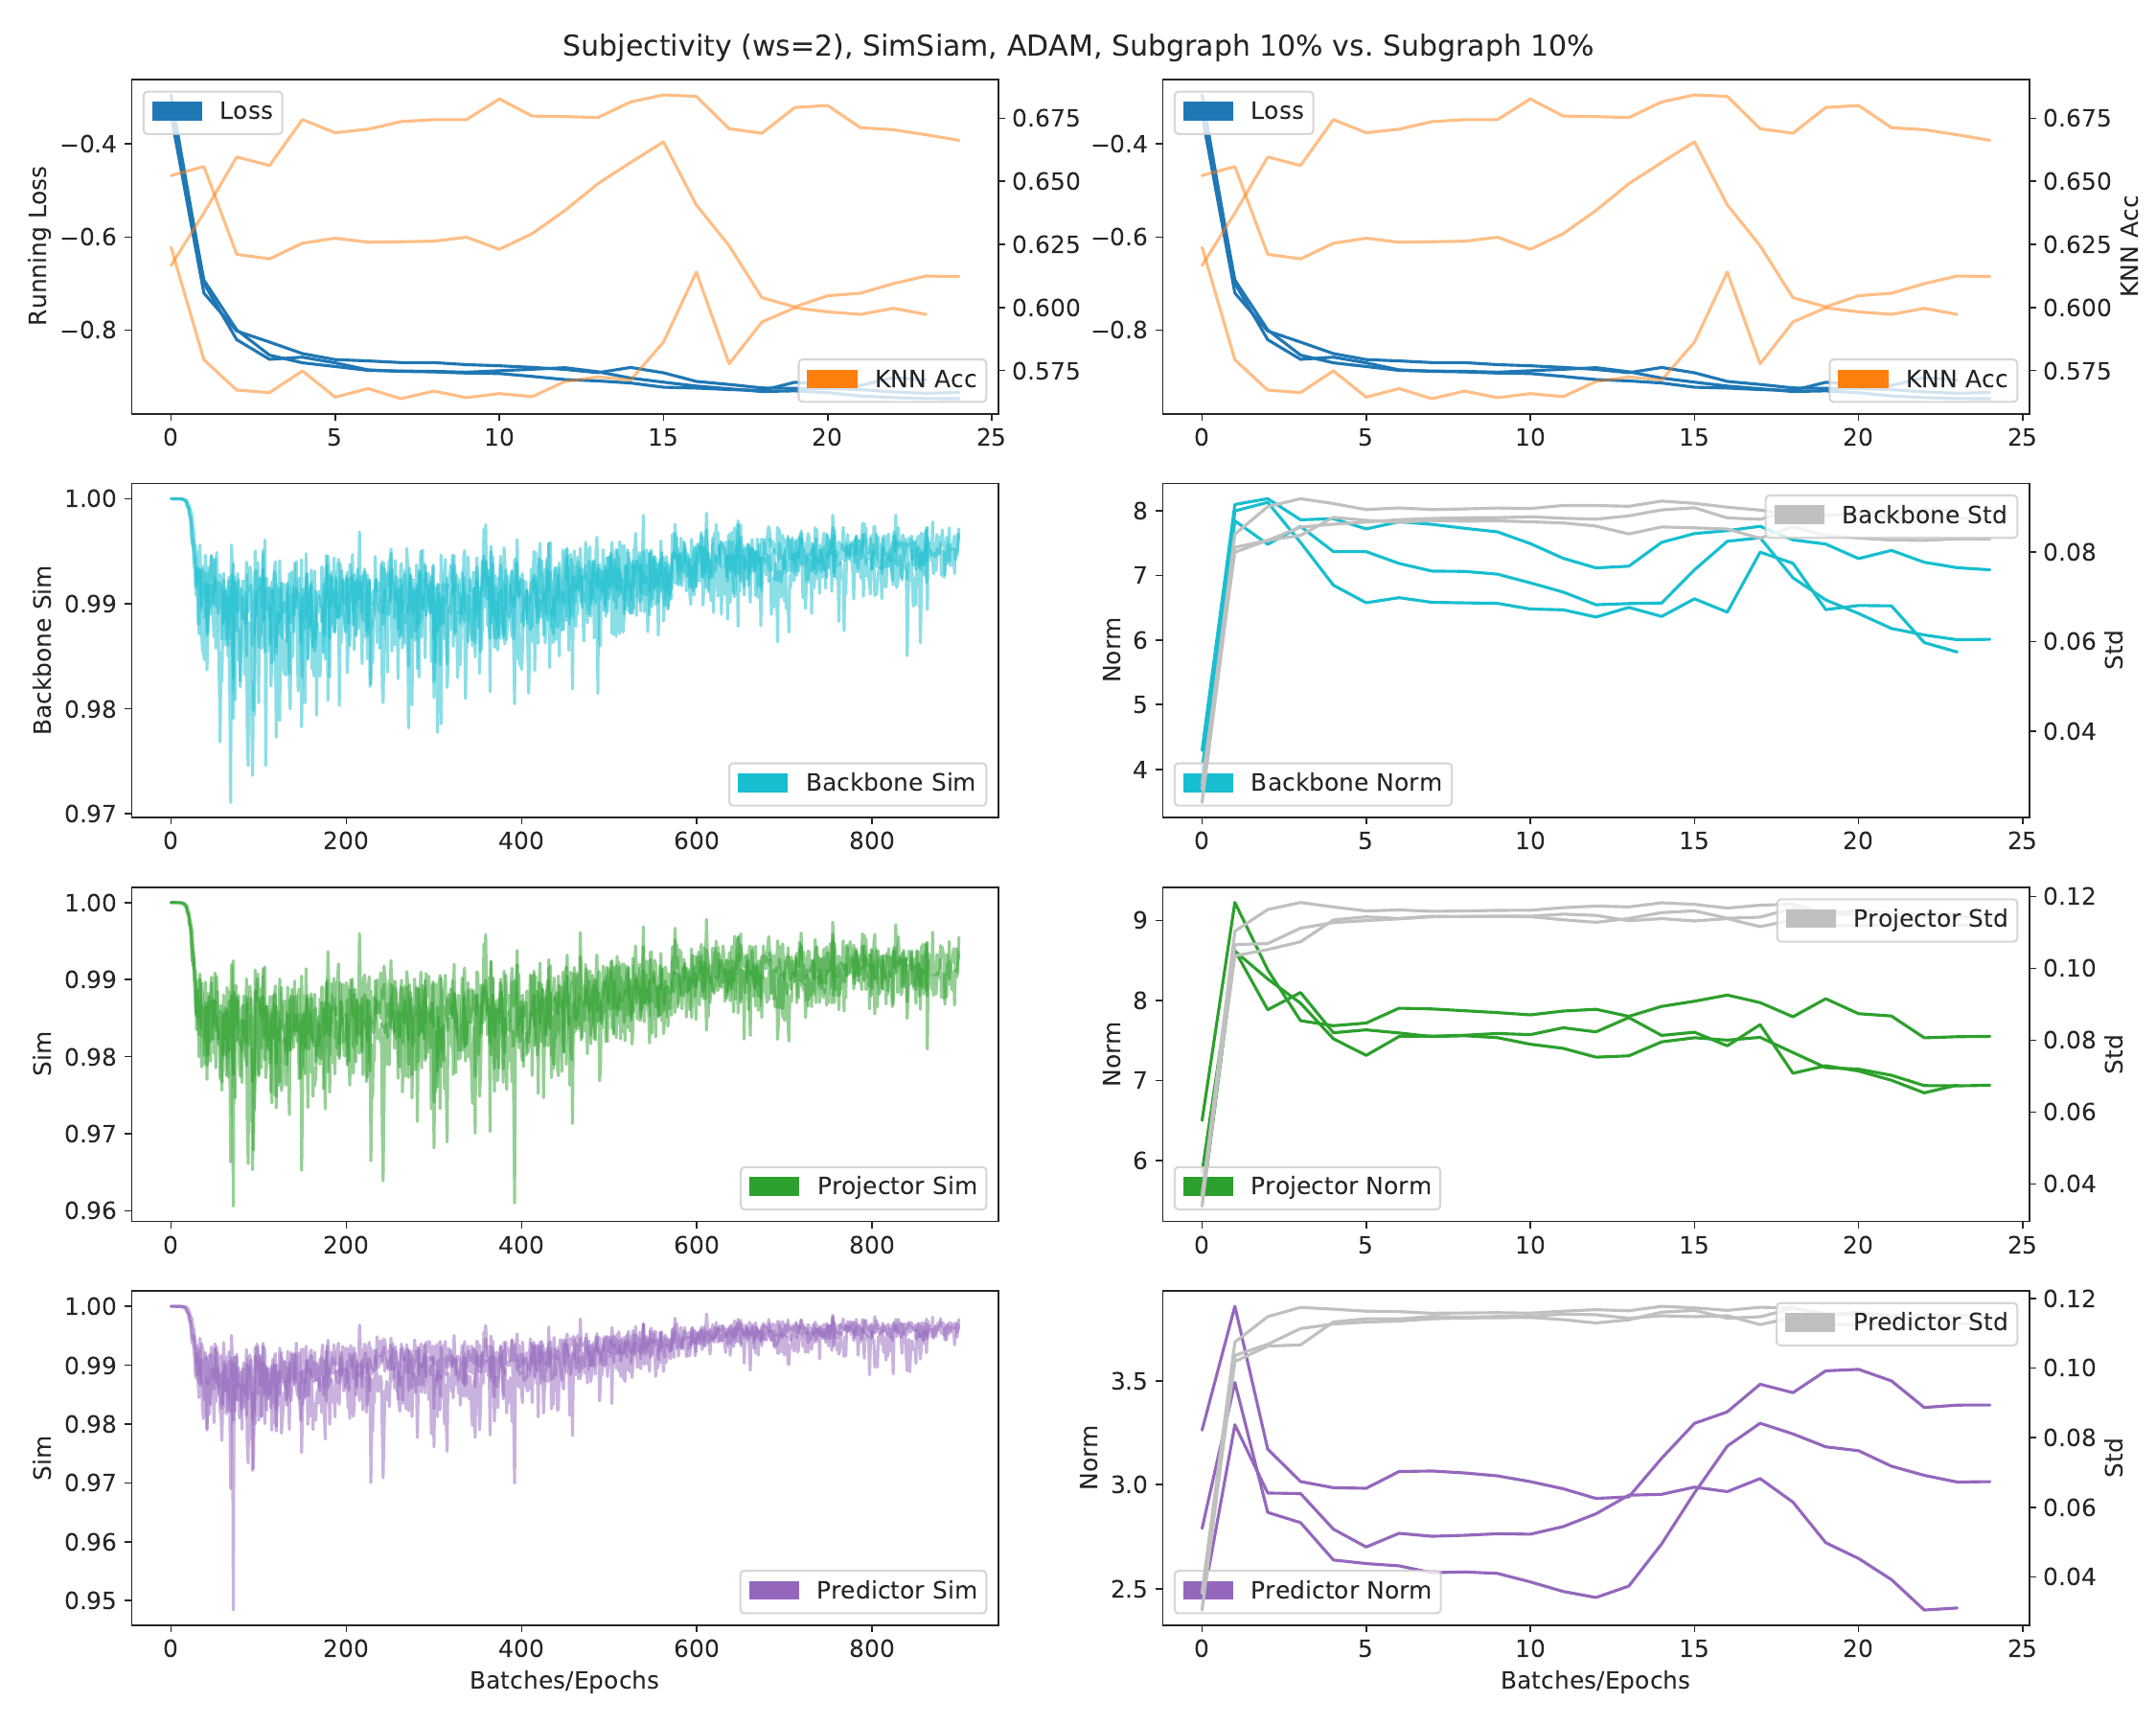}
    \caption{SimSiam, WS=2, Subgraph 10\% vs. Subgraph 10\%}
    \label{fig:simsiam_nlp_ws2_sub10_v_sub10}
\end{figure}
\begin{figure}[H]
    \centering
    \includegraphics[width=0.8\textwidth]{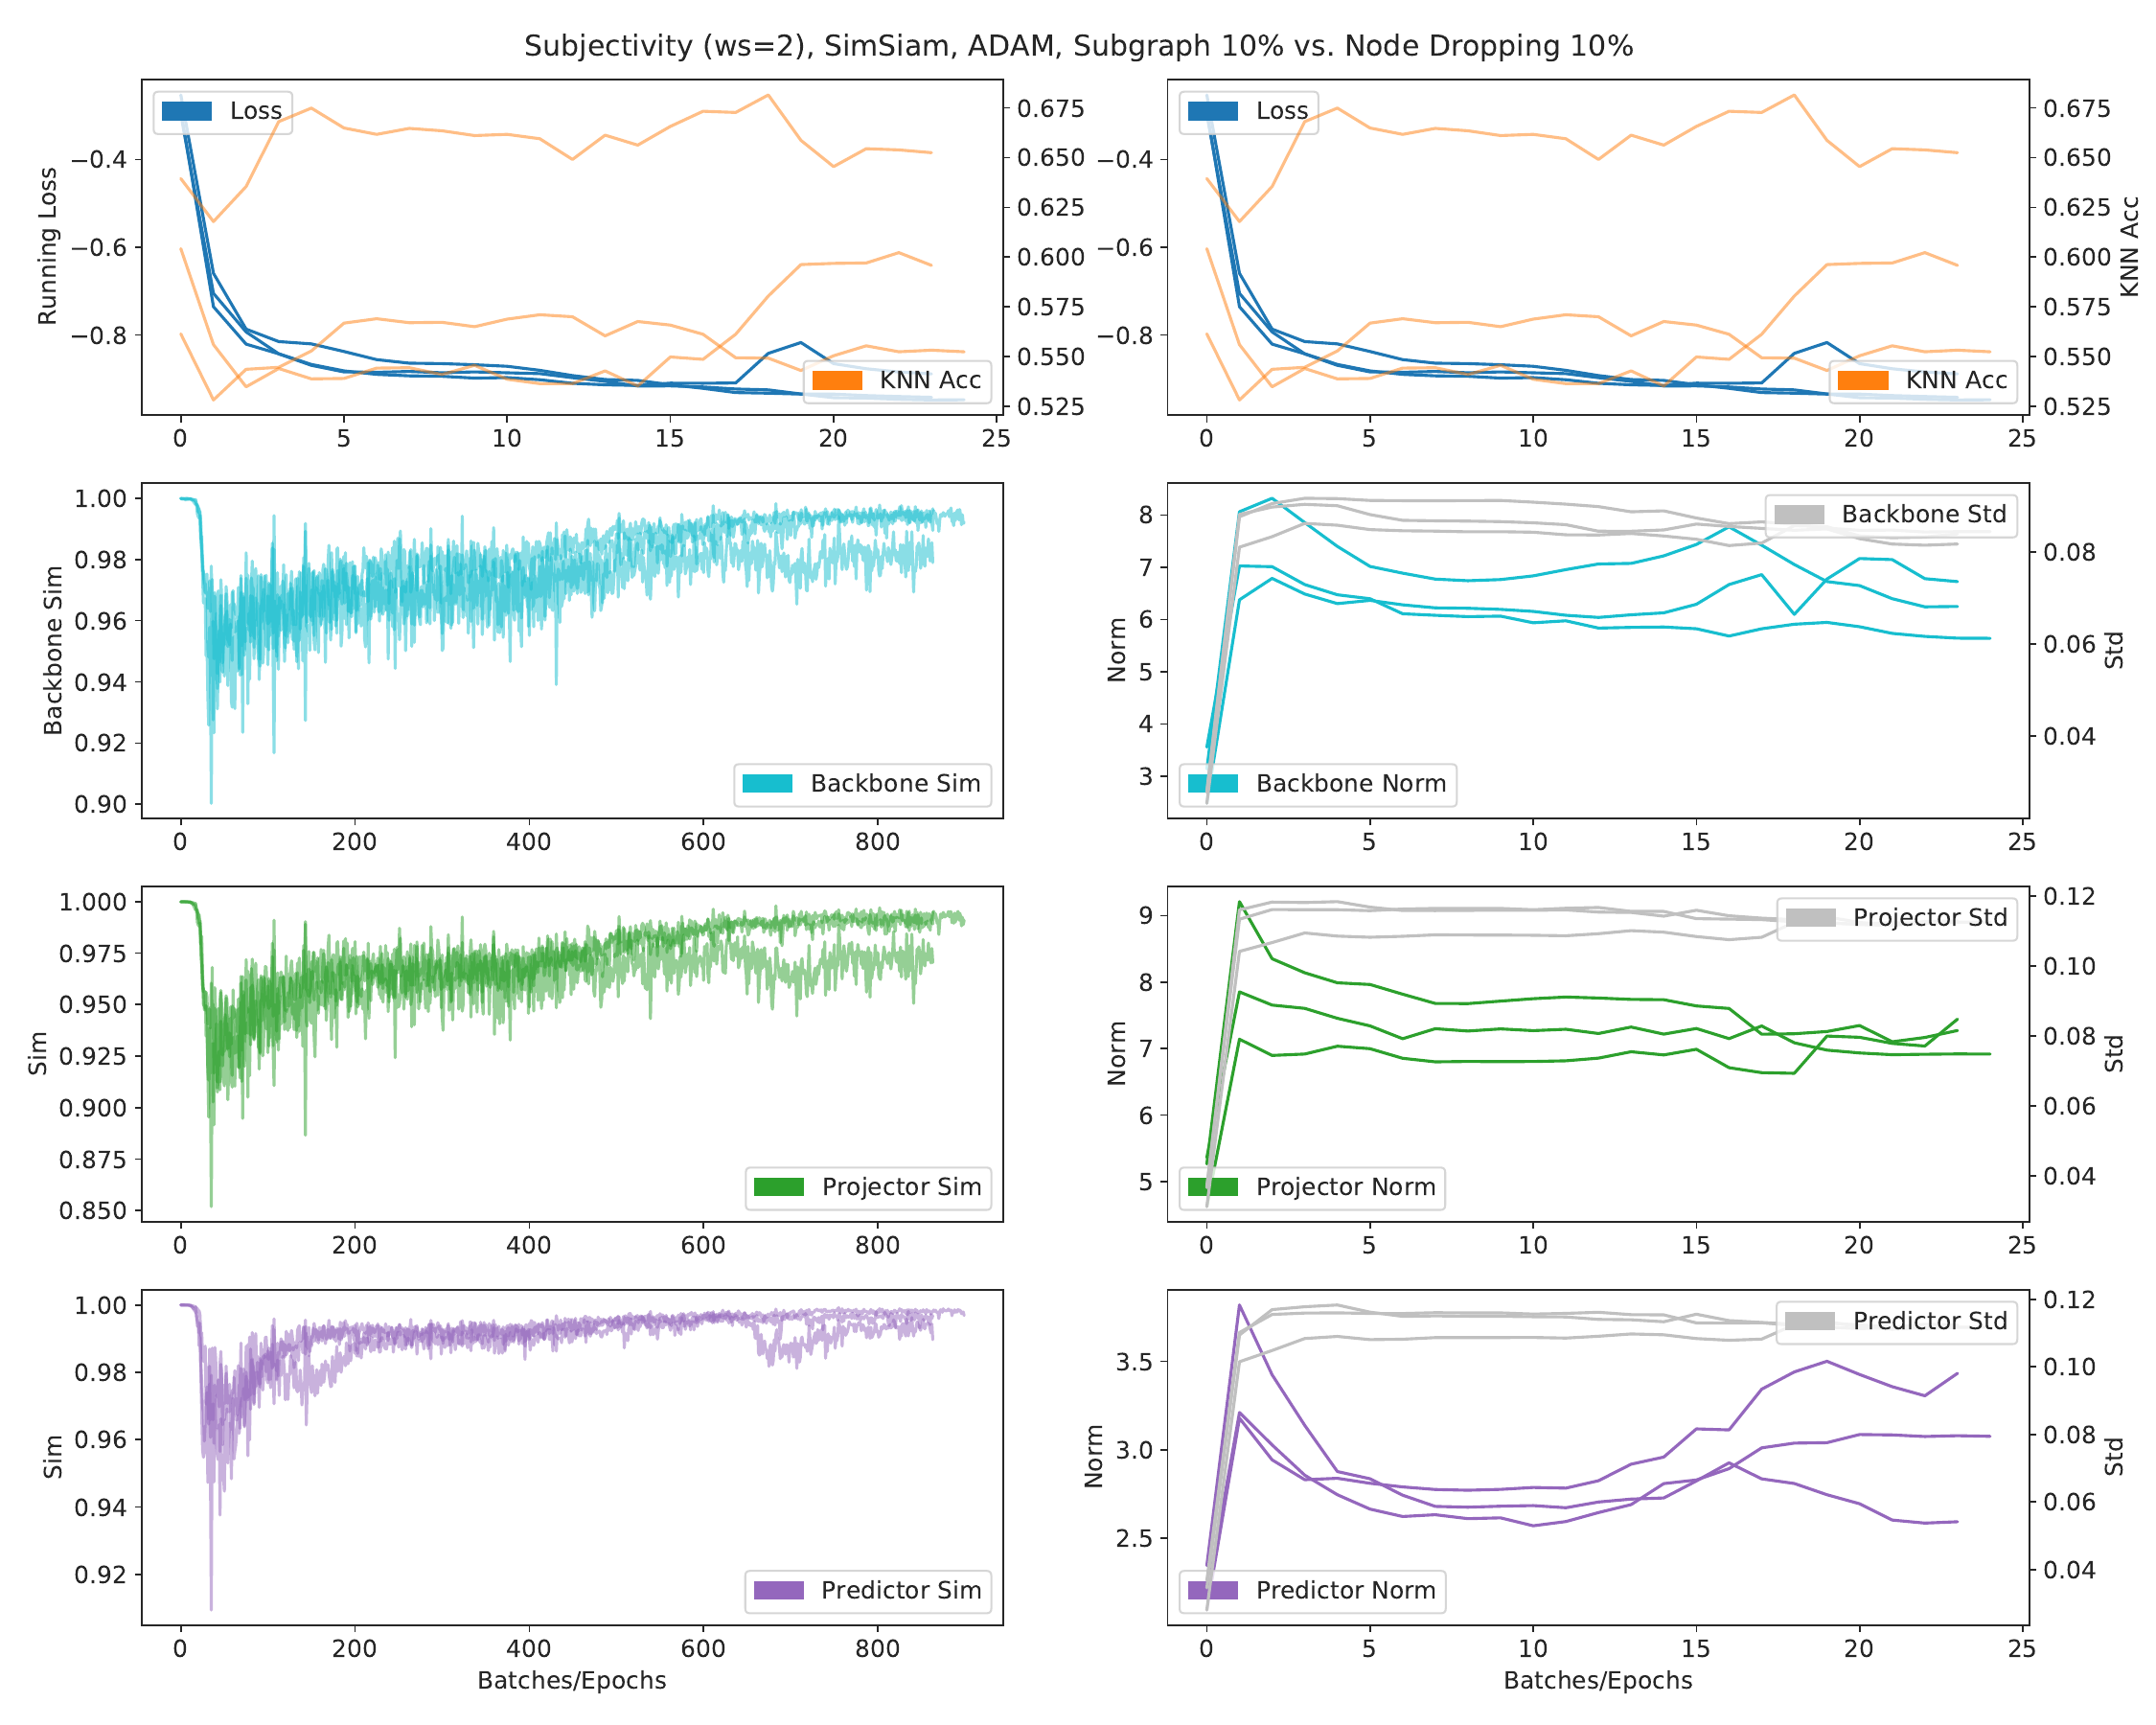}
    \caption{SimSiam, WS=2, Subgraph 10\% vs. Node Dropping 10\%}
    \label{fig:simsiam_nlp_ws2_sub10_v_node10}
\end{figure}
\begin{figure}[H]
    \centering
    \includegraphics[width=0.8\textwidth]{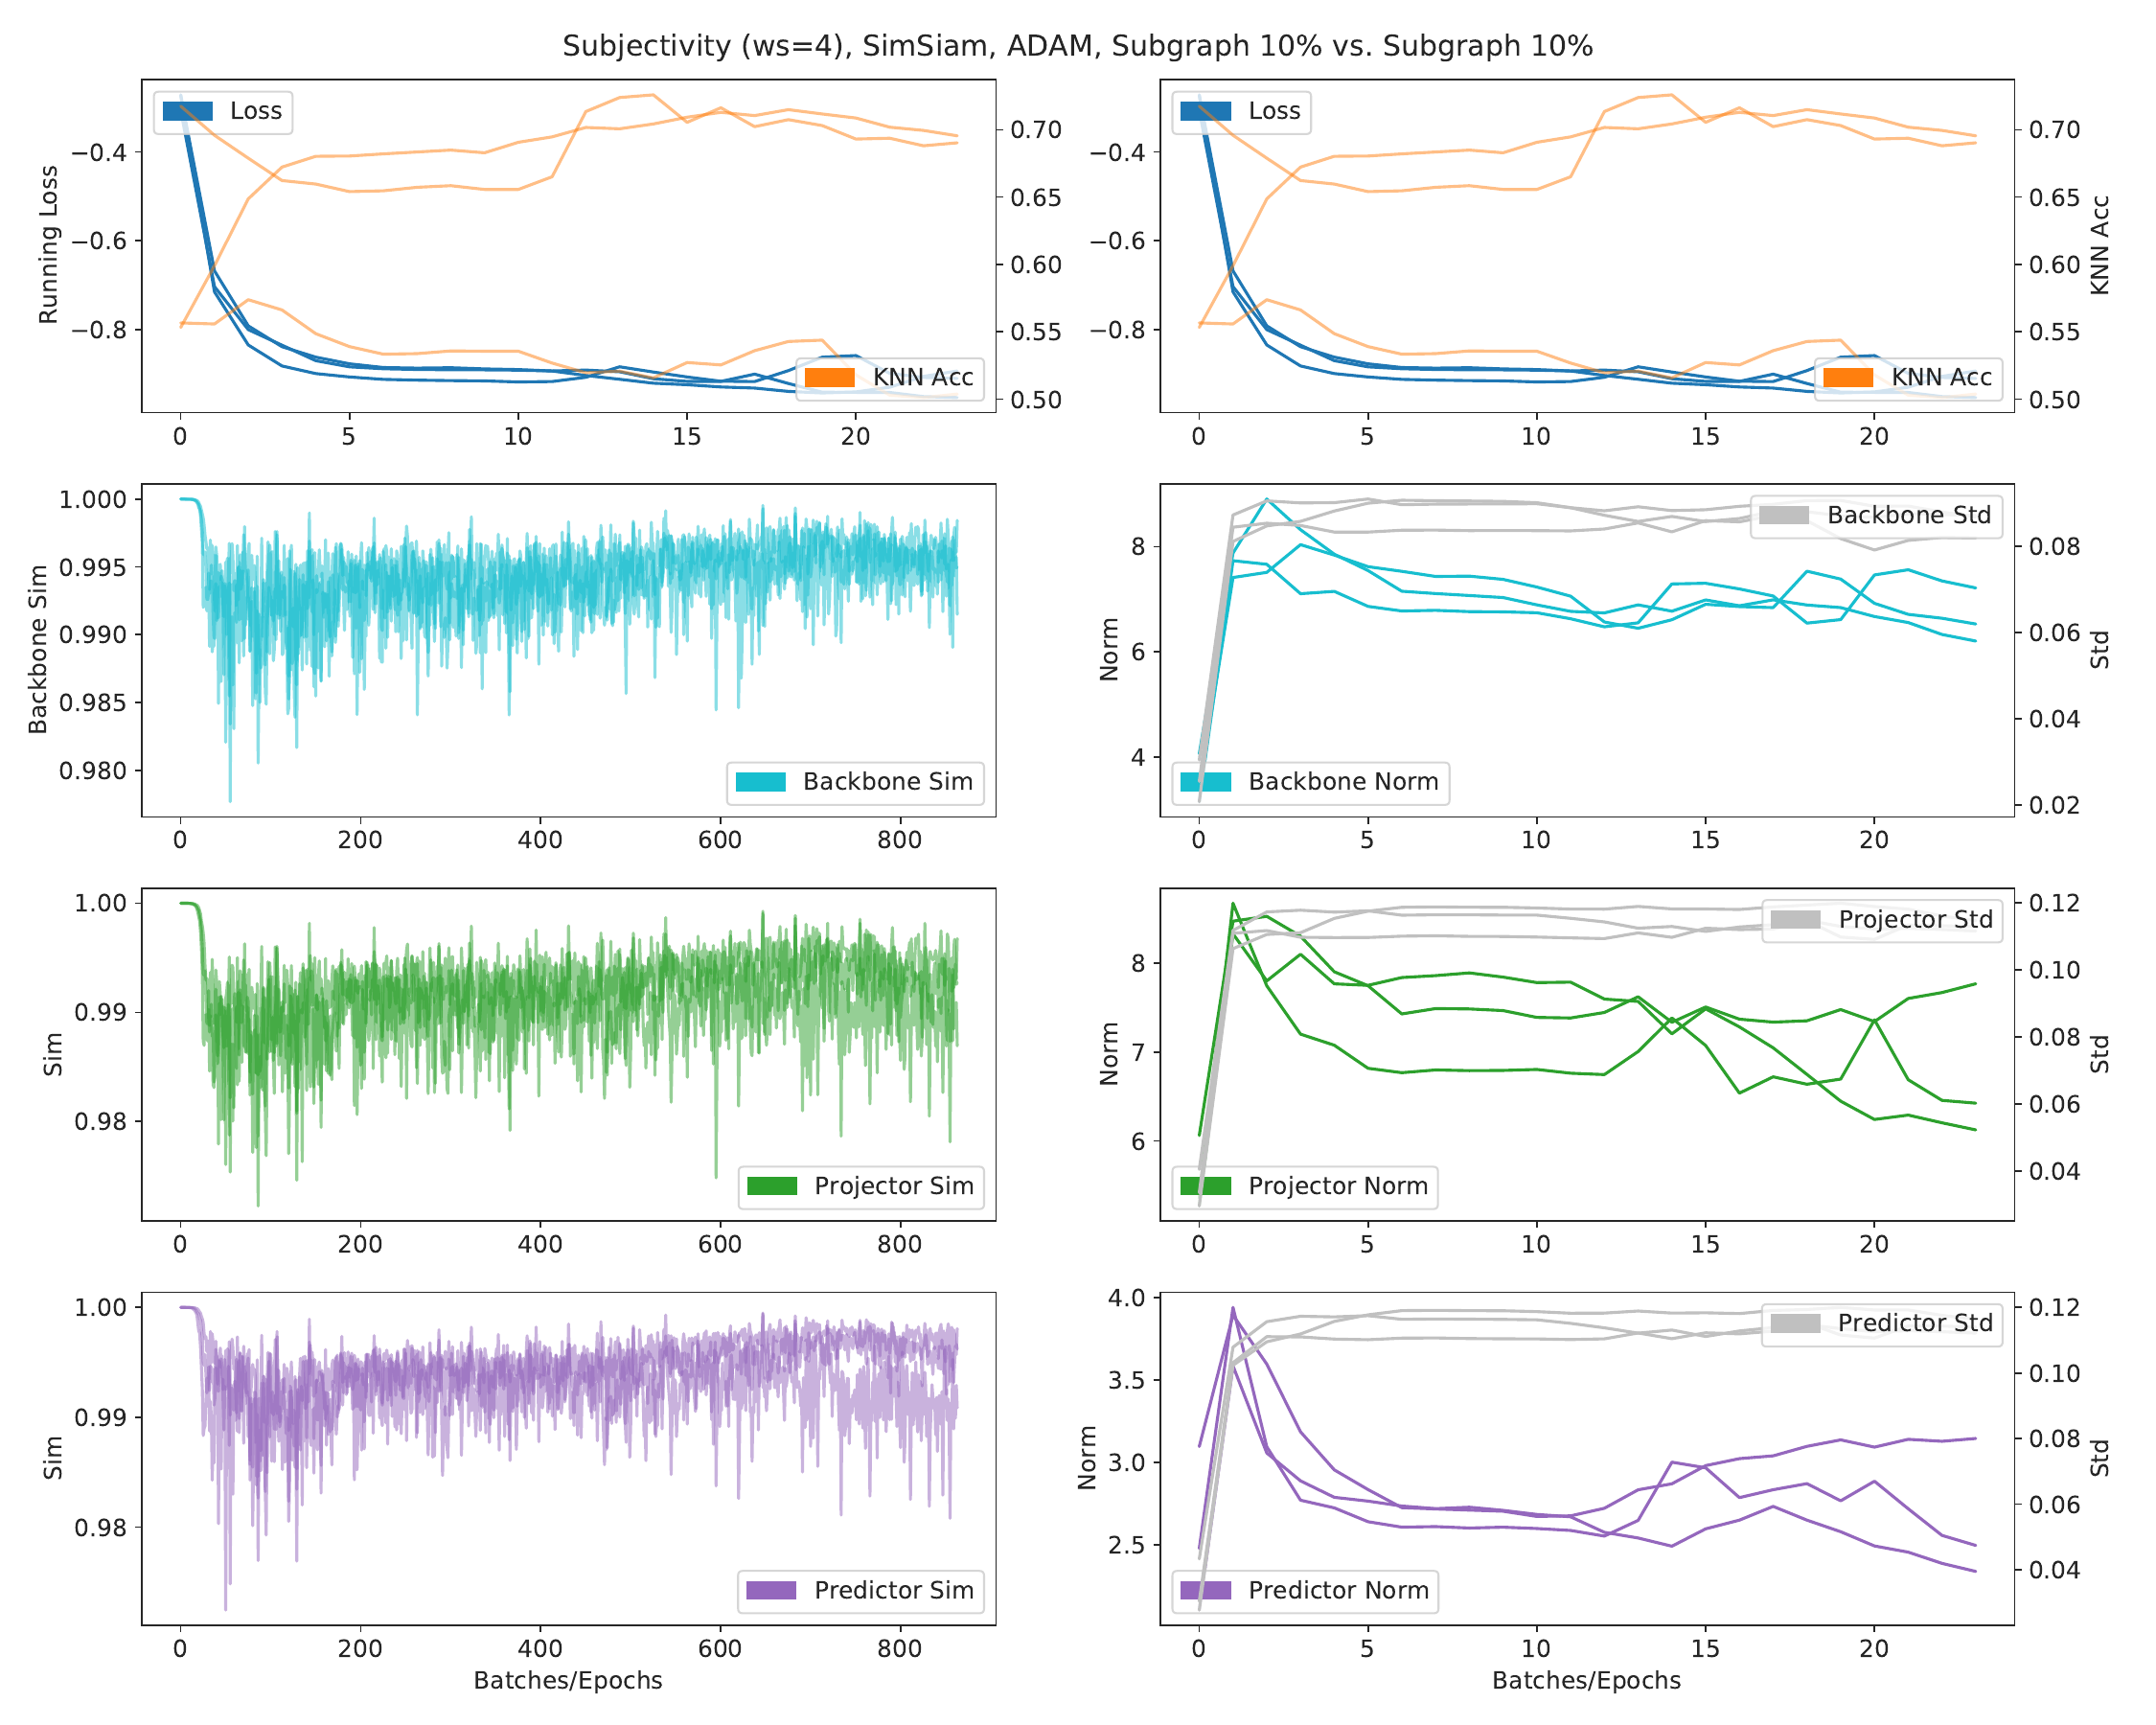}
    \caption{SimSiam, WS=4, Subgraph 10\% vs. Subgraph 10\%}
    \label{fig:simsiam_nlp_ws4_sub10_v_sub10}
\end{figure}
\begin{figure}[H]
    \centering
    \includegraphics[width=0.8\textwidth]{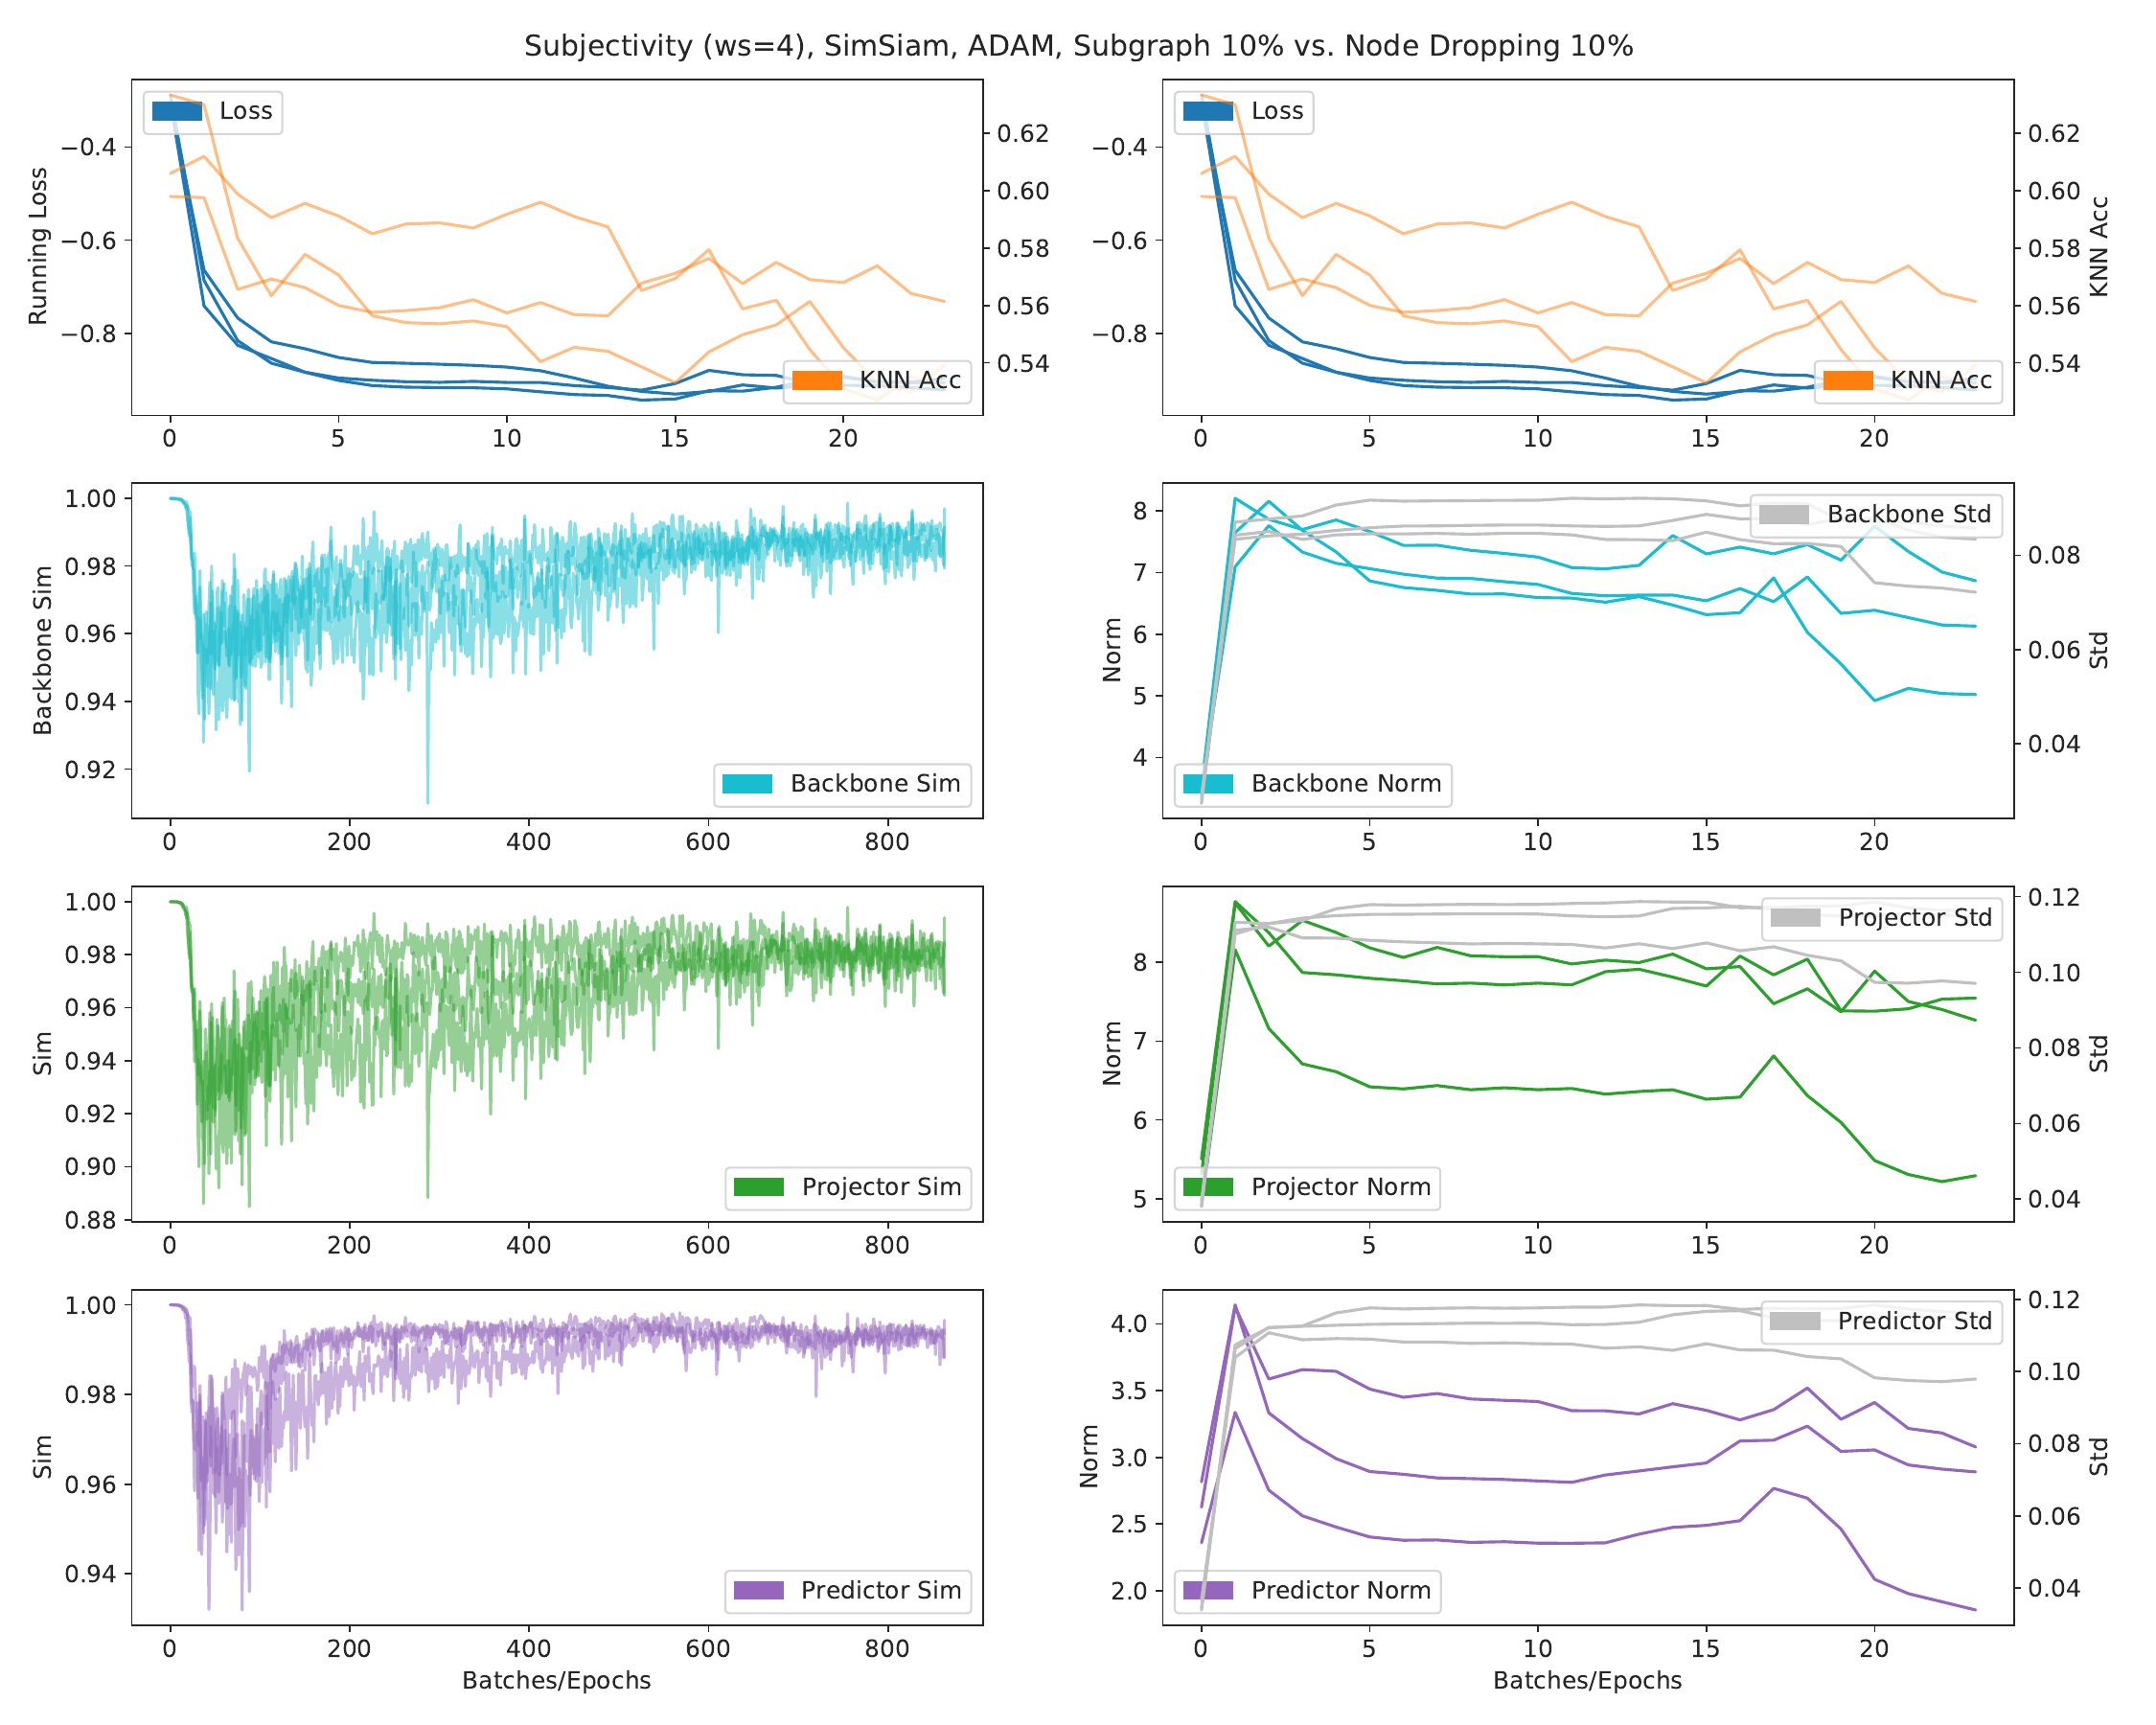}
    \caption{SimSiam, WS=4, Subgraph 10\% vs. Node Dropping 10\%}
    \label{fig:simsiam_nlp_ws4_sub10_v_node10}
\end{figure}

\subsection{BYOL}\label{app_text_byol}
In this section, we report our training setup for document classification using BYOL (\cite{Grill20_BYOL}), a positive-sample-only framework. We use the hyper-parameters discussed in Sec. \ref{sec:app_doc}. Further, in Figs. (\ref{fig:byol_nlp_ws2}, \ref{fig:byol_nlp_ws2_sub10_v_node10}, \ref{fig:byol_nlp_ws2_sub10_v_sub10}, \ref{fig:byol_nlp_ws4}, \ref{fig:byol_nlp_ws4_sub10_v_node10}, \ref{fig:byol_nlp_ws4_sub10_v_sub10}), we plot KNN accuracy and loss as well as the norm, standard deviation, and similarity of backbone, encoder, and projector representations throughout training. 
\begin{figure}[H]
    \centering
    \includegraphics[width=0.8\textwidth]{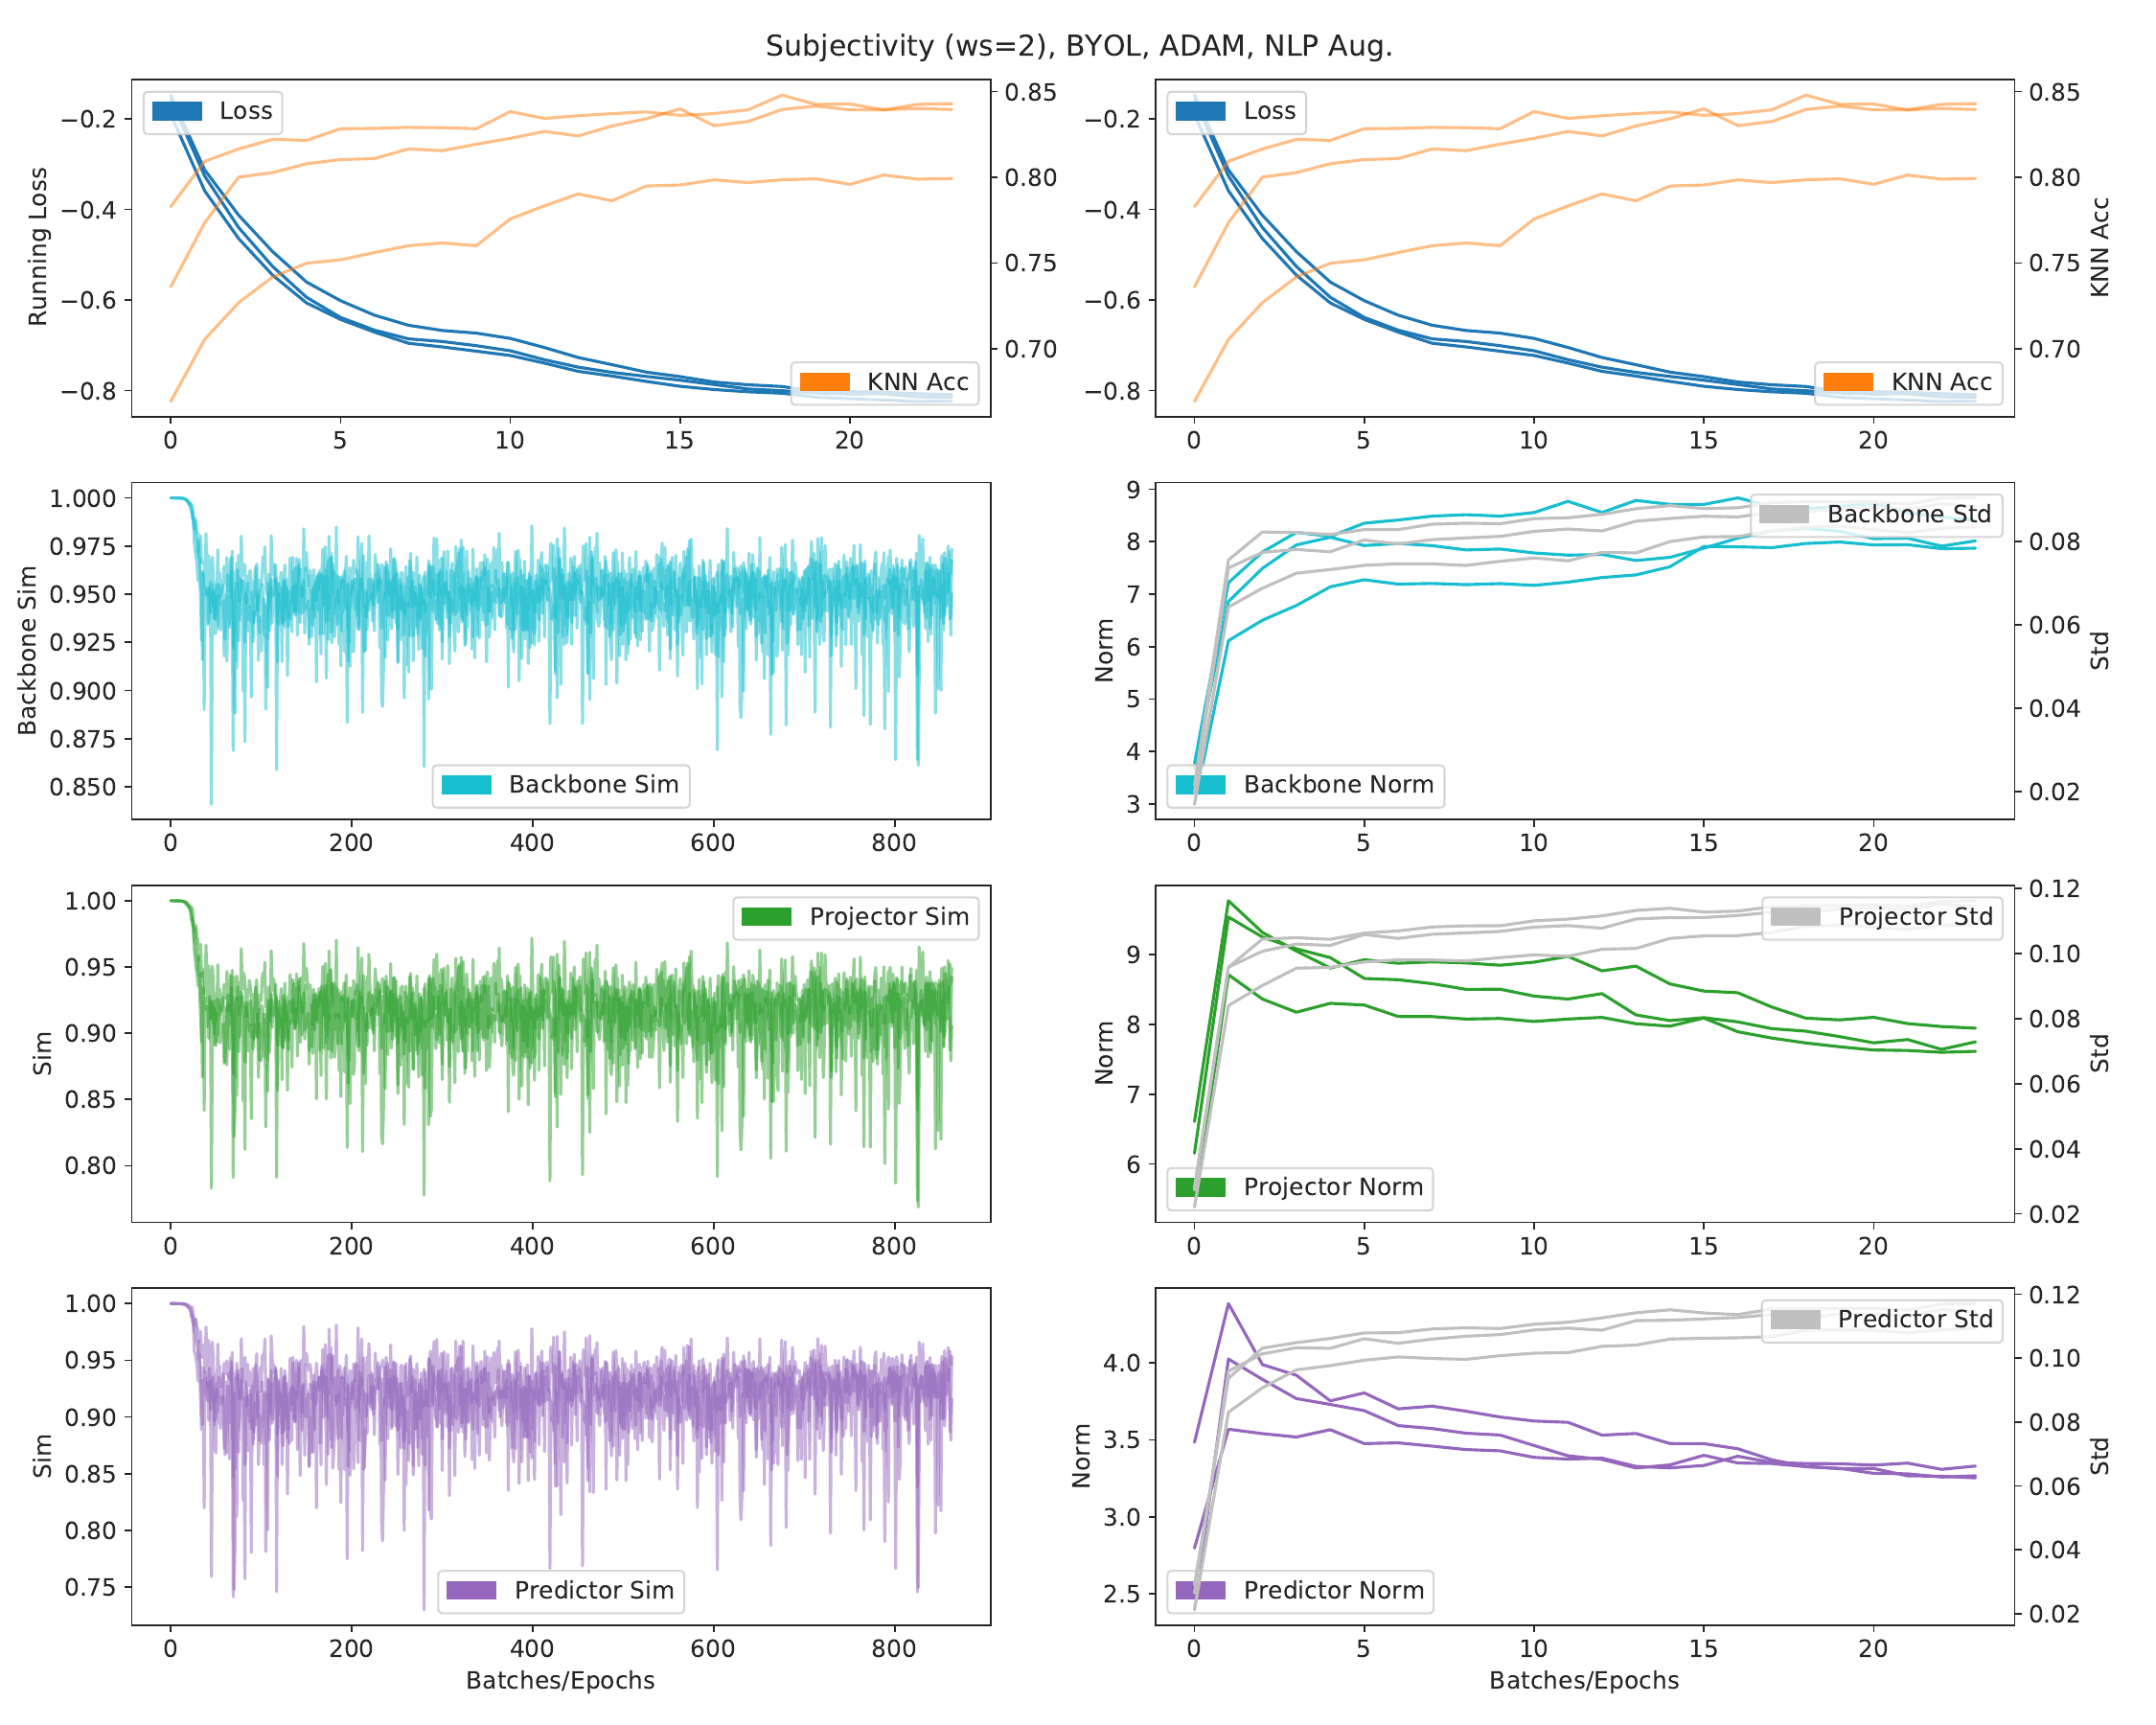}
    \caption{BYOL, WS=2, NLP Augmentations}
    \label{fig:byol_nlp_ws2}
\end{figure}
\begin{figure}[H]
    \centering
    \includegraphics[width=0.8\textwidth]{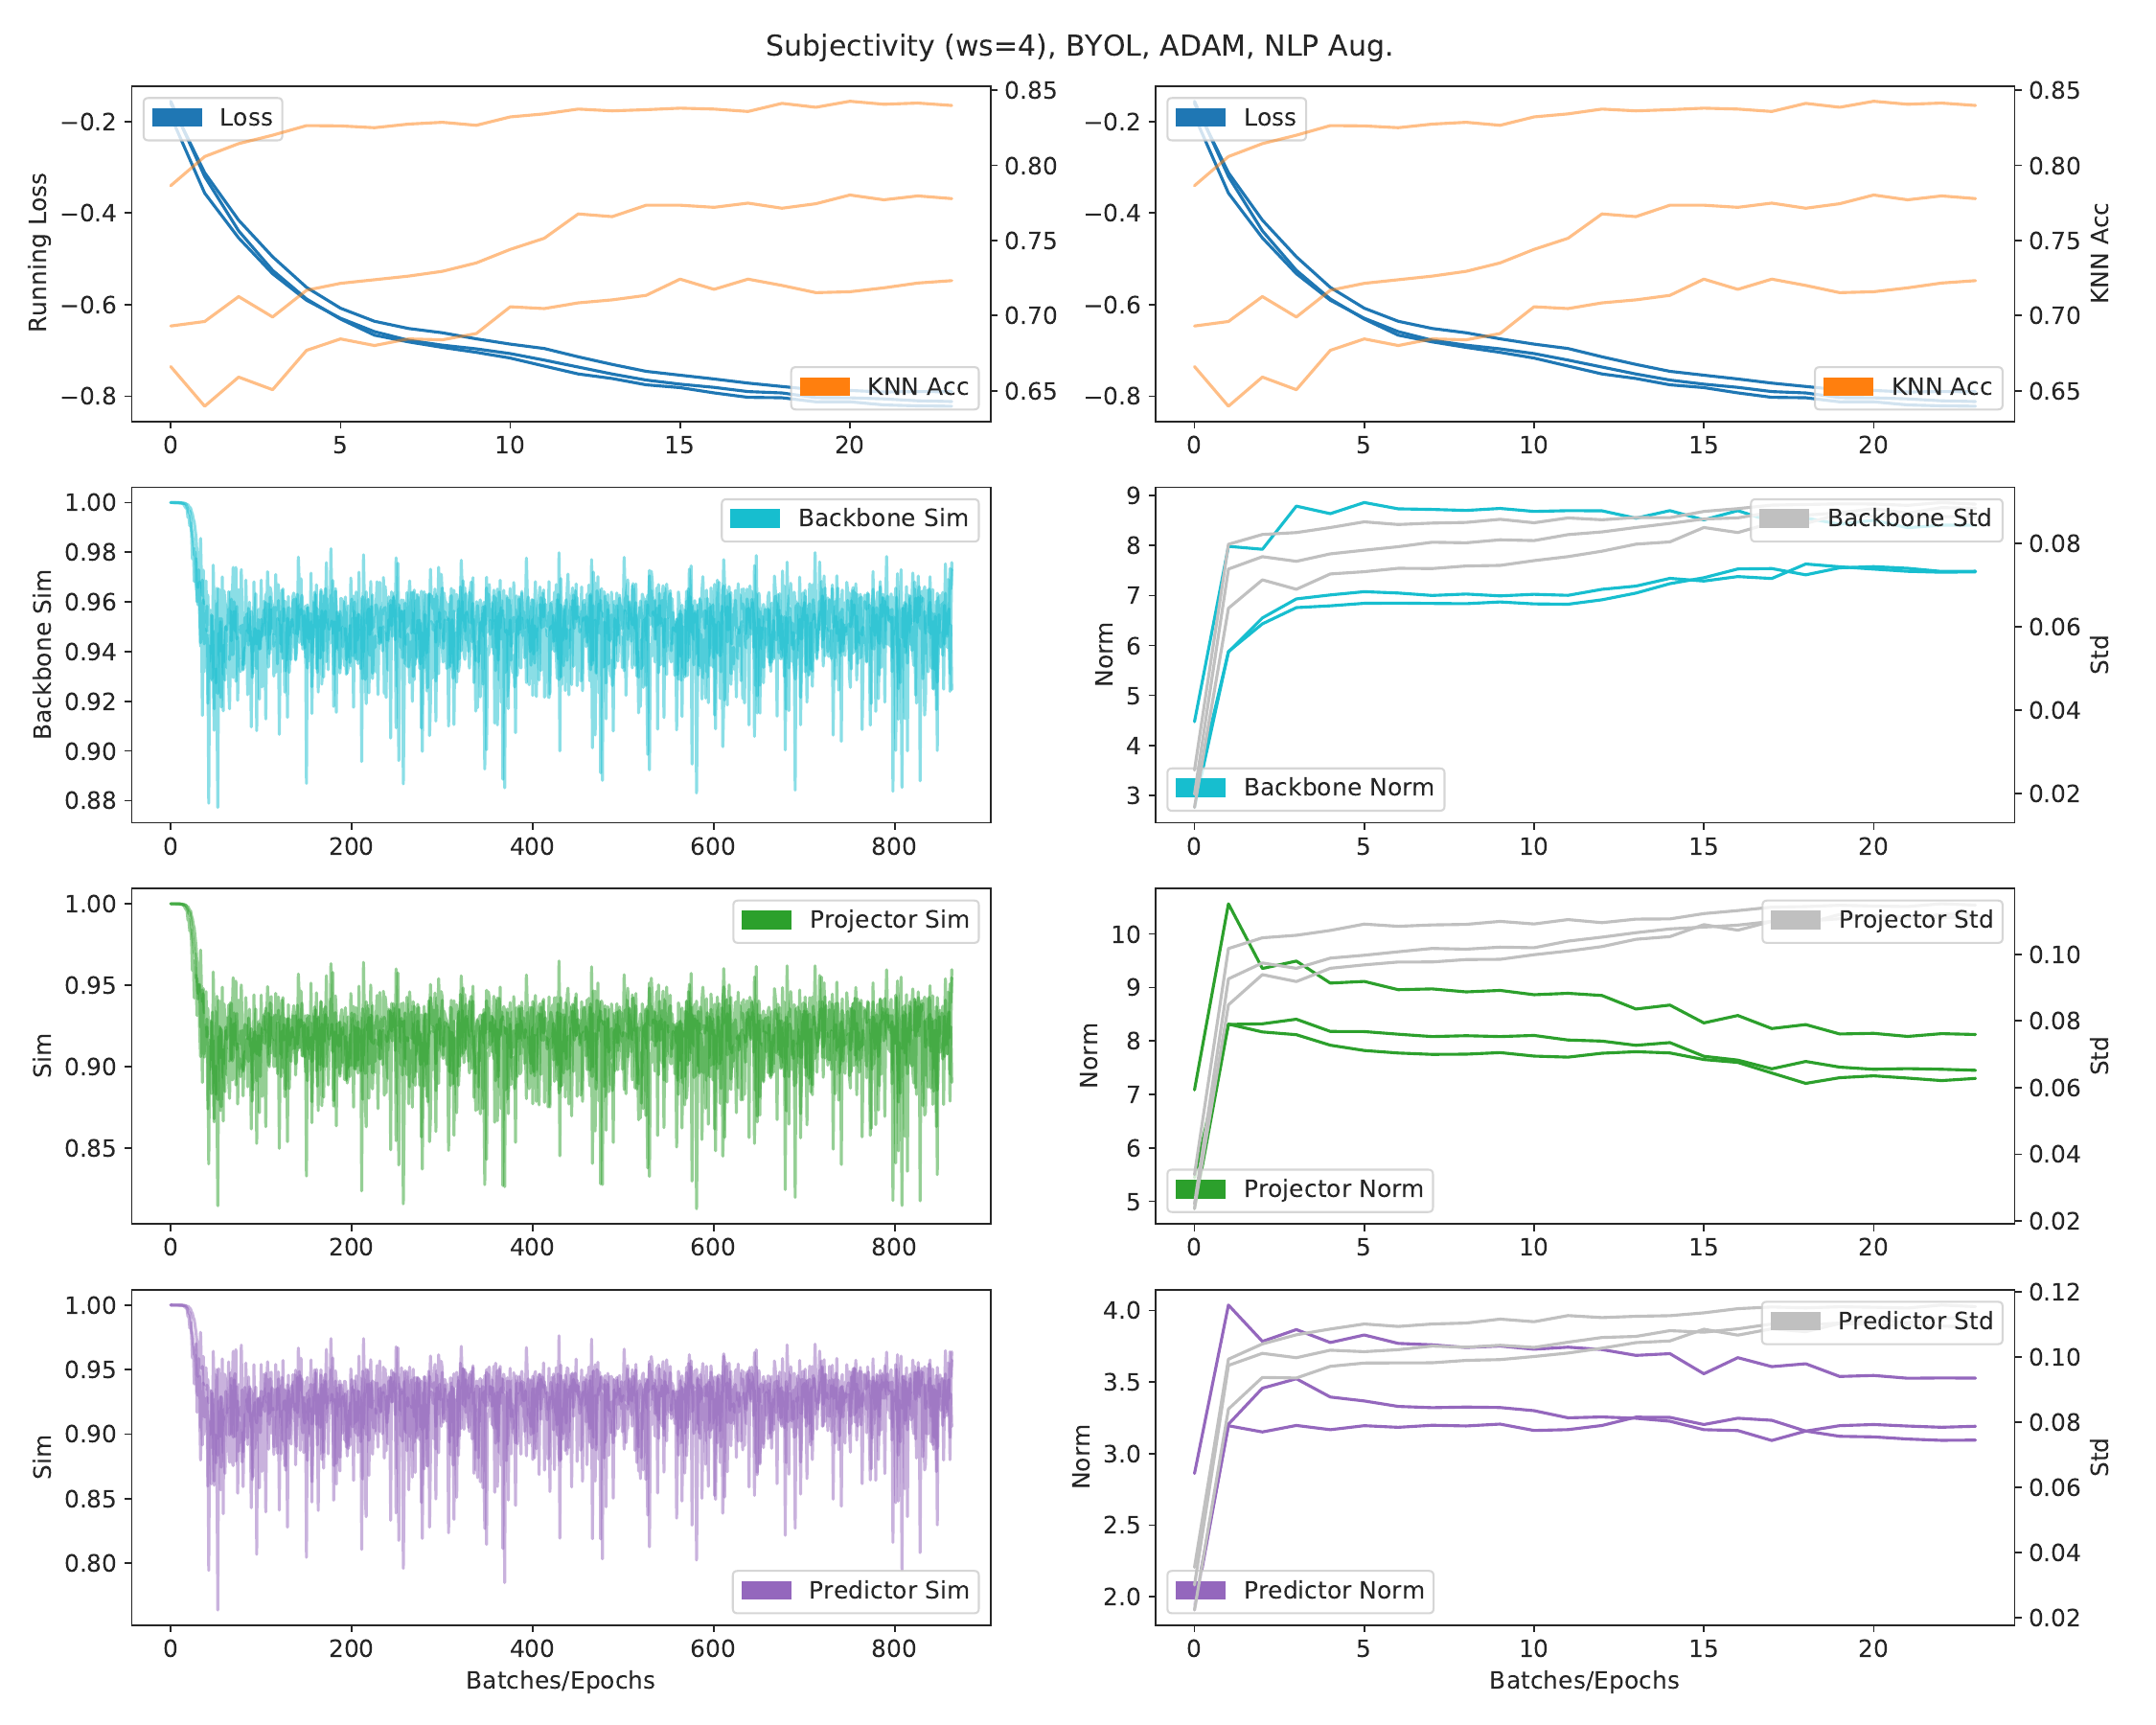}
    \caption{BYOL, WS=4, NLP Augmentations}
    \label{fig:byol_nlp_ws4}
\end{figure}
\begin{figure}[H]
    \centering
    \includegraphics[width=0.8\textwidth]{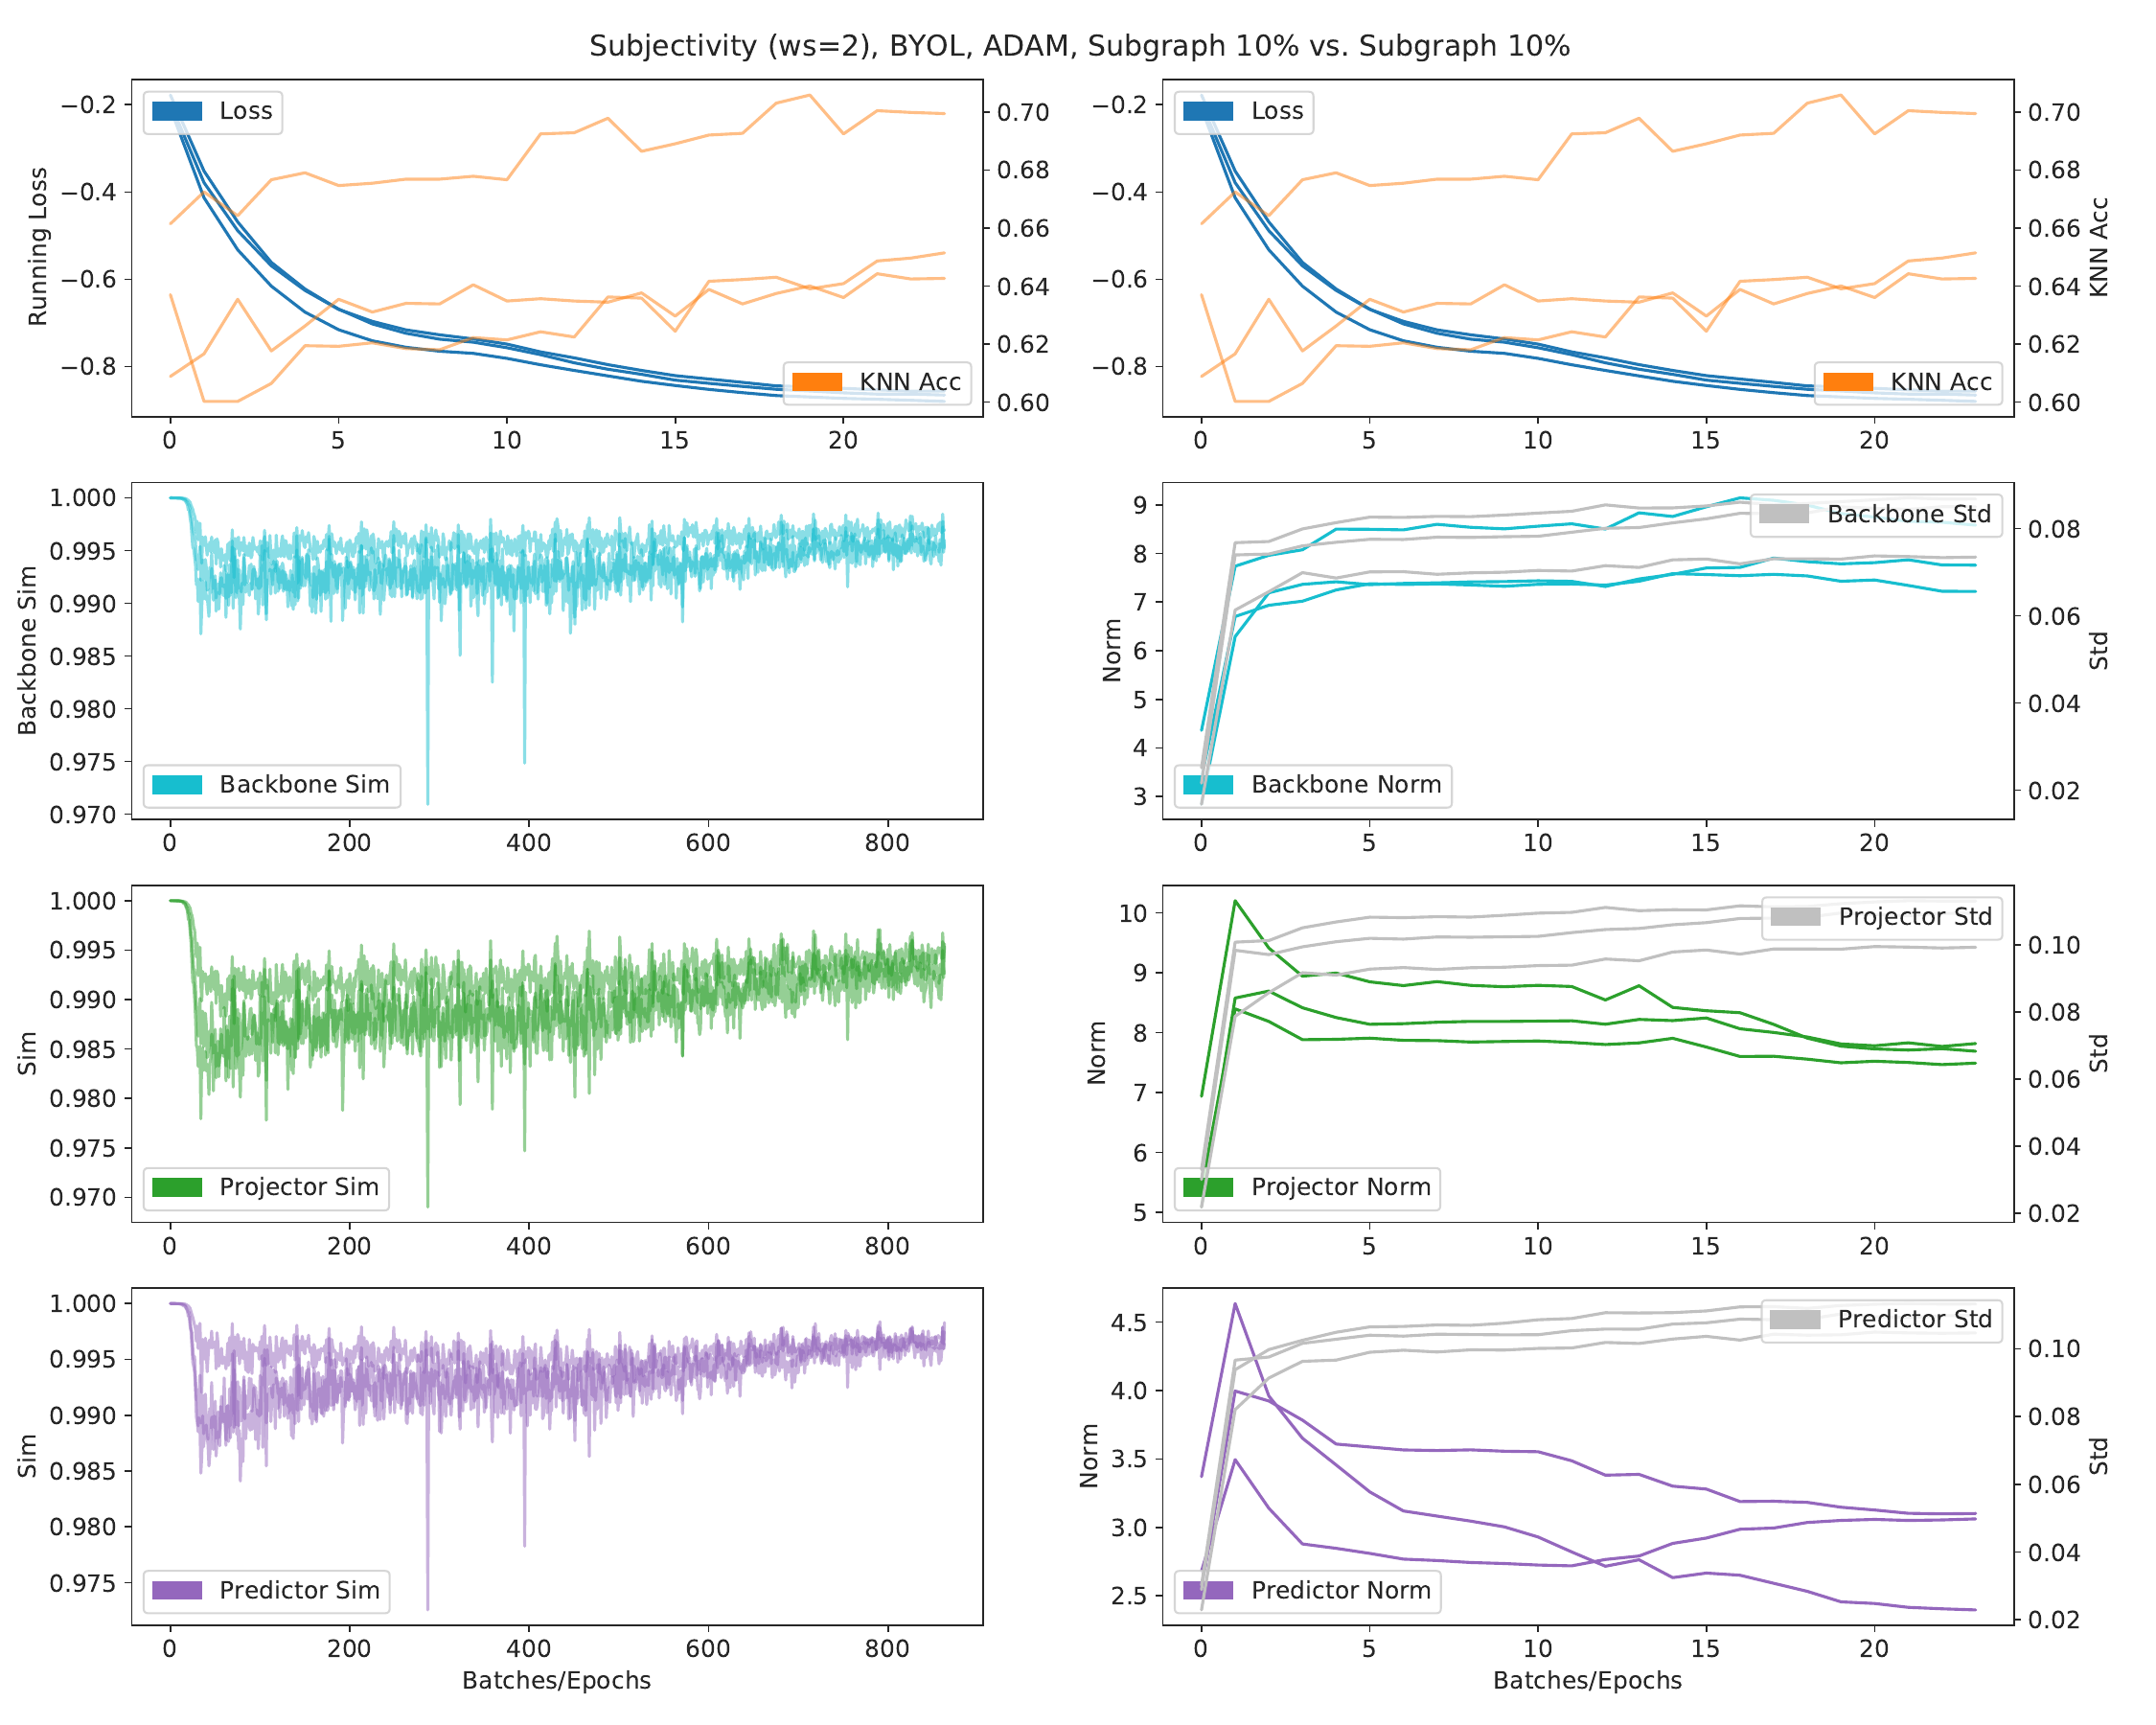}
    \caption{BYOL, WS=2, Subgraph 10\% vs. Subgraph 10\%}
    \label{fig:byol_nlp_ws2_sub10_v_sub10}
\end{figure}
\begin{figure}[H]
    \centering
    \includegraphics[width=0.8\textwidth]{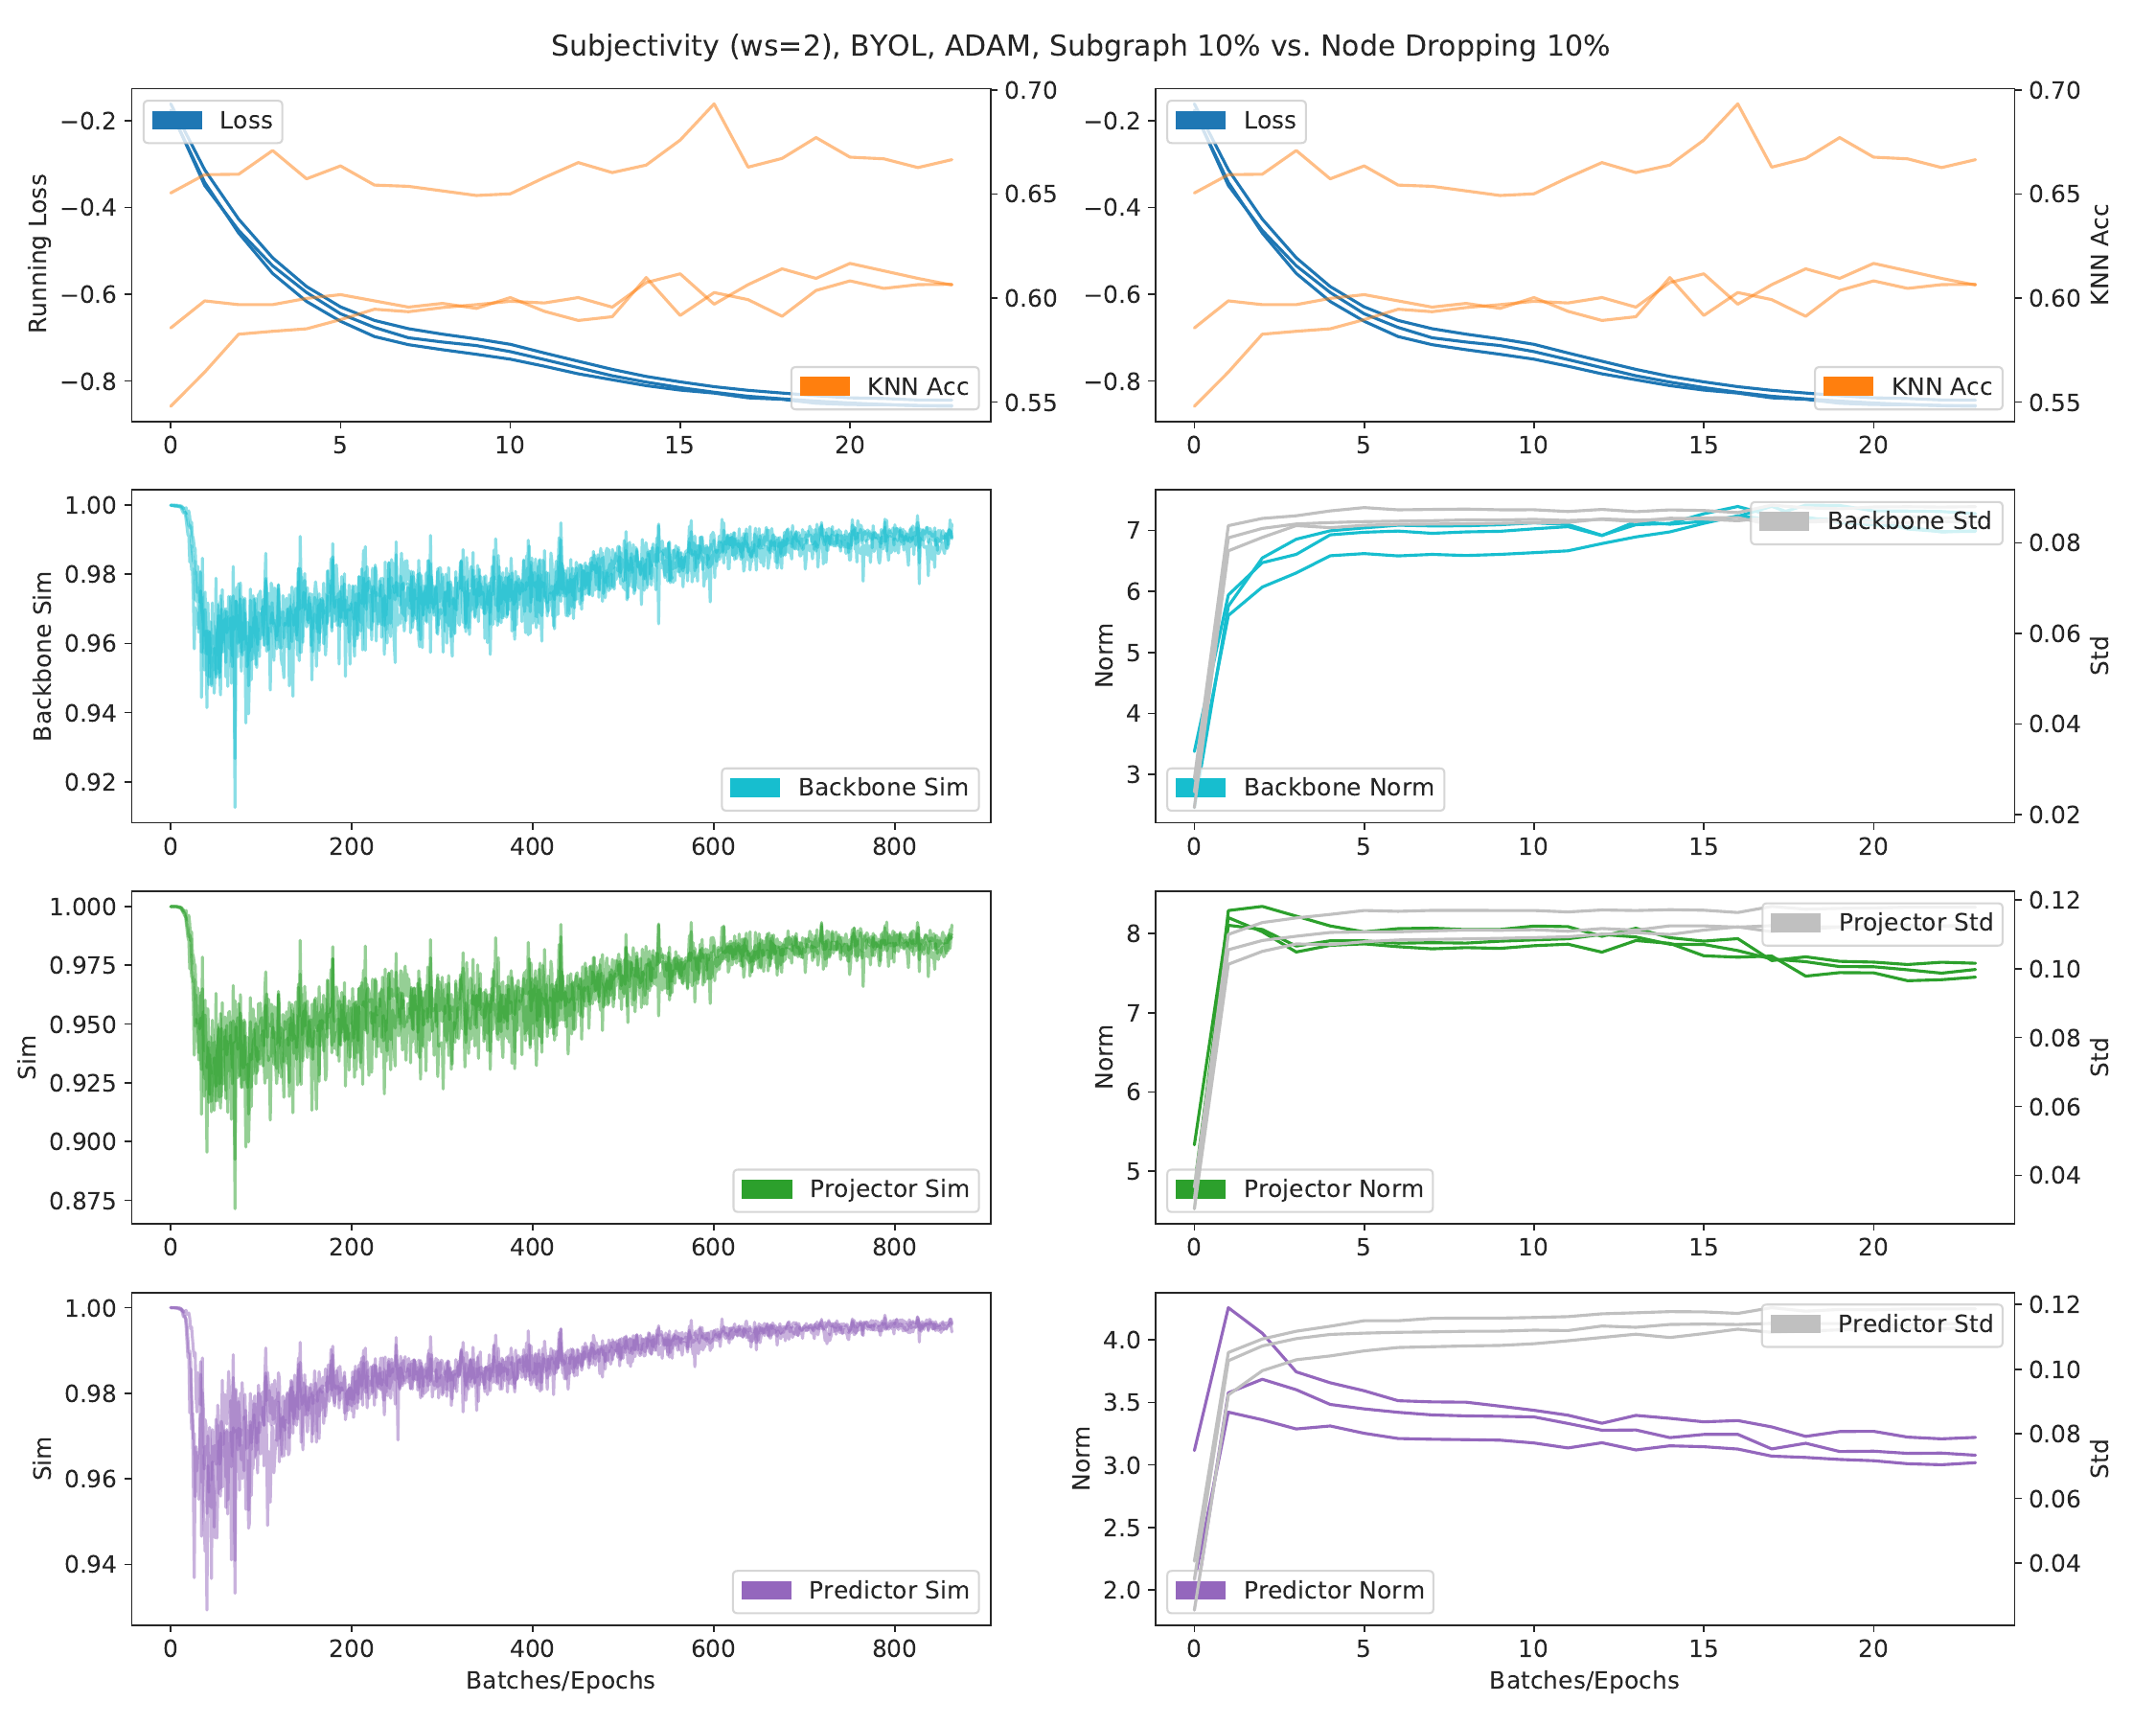}
    \caption{BYOL, WS=2, Subgraph 10\% vs. Node Dropping 10\%}
    \label{fig:byol_nlp_ws2_sub10_v_node10}
\end{figure}
\begin{figure}[H]
    \centering
    \includegraphics[width=0.8\textwidth]{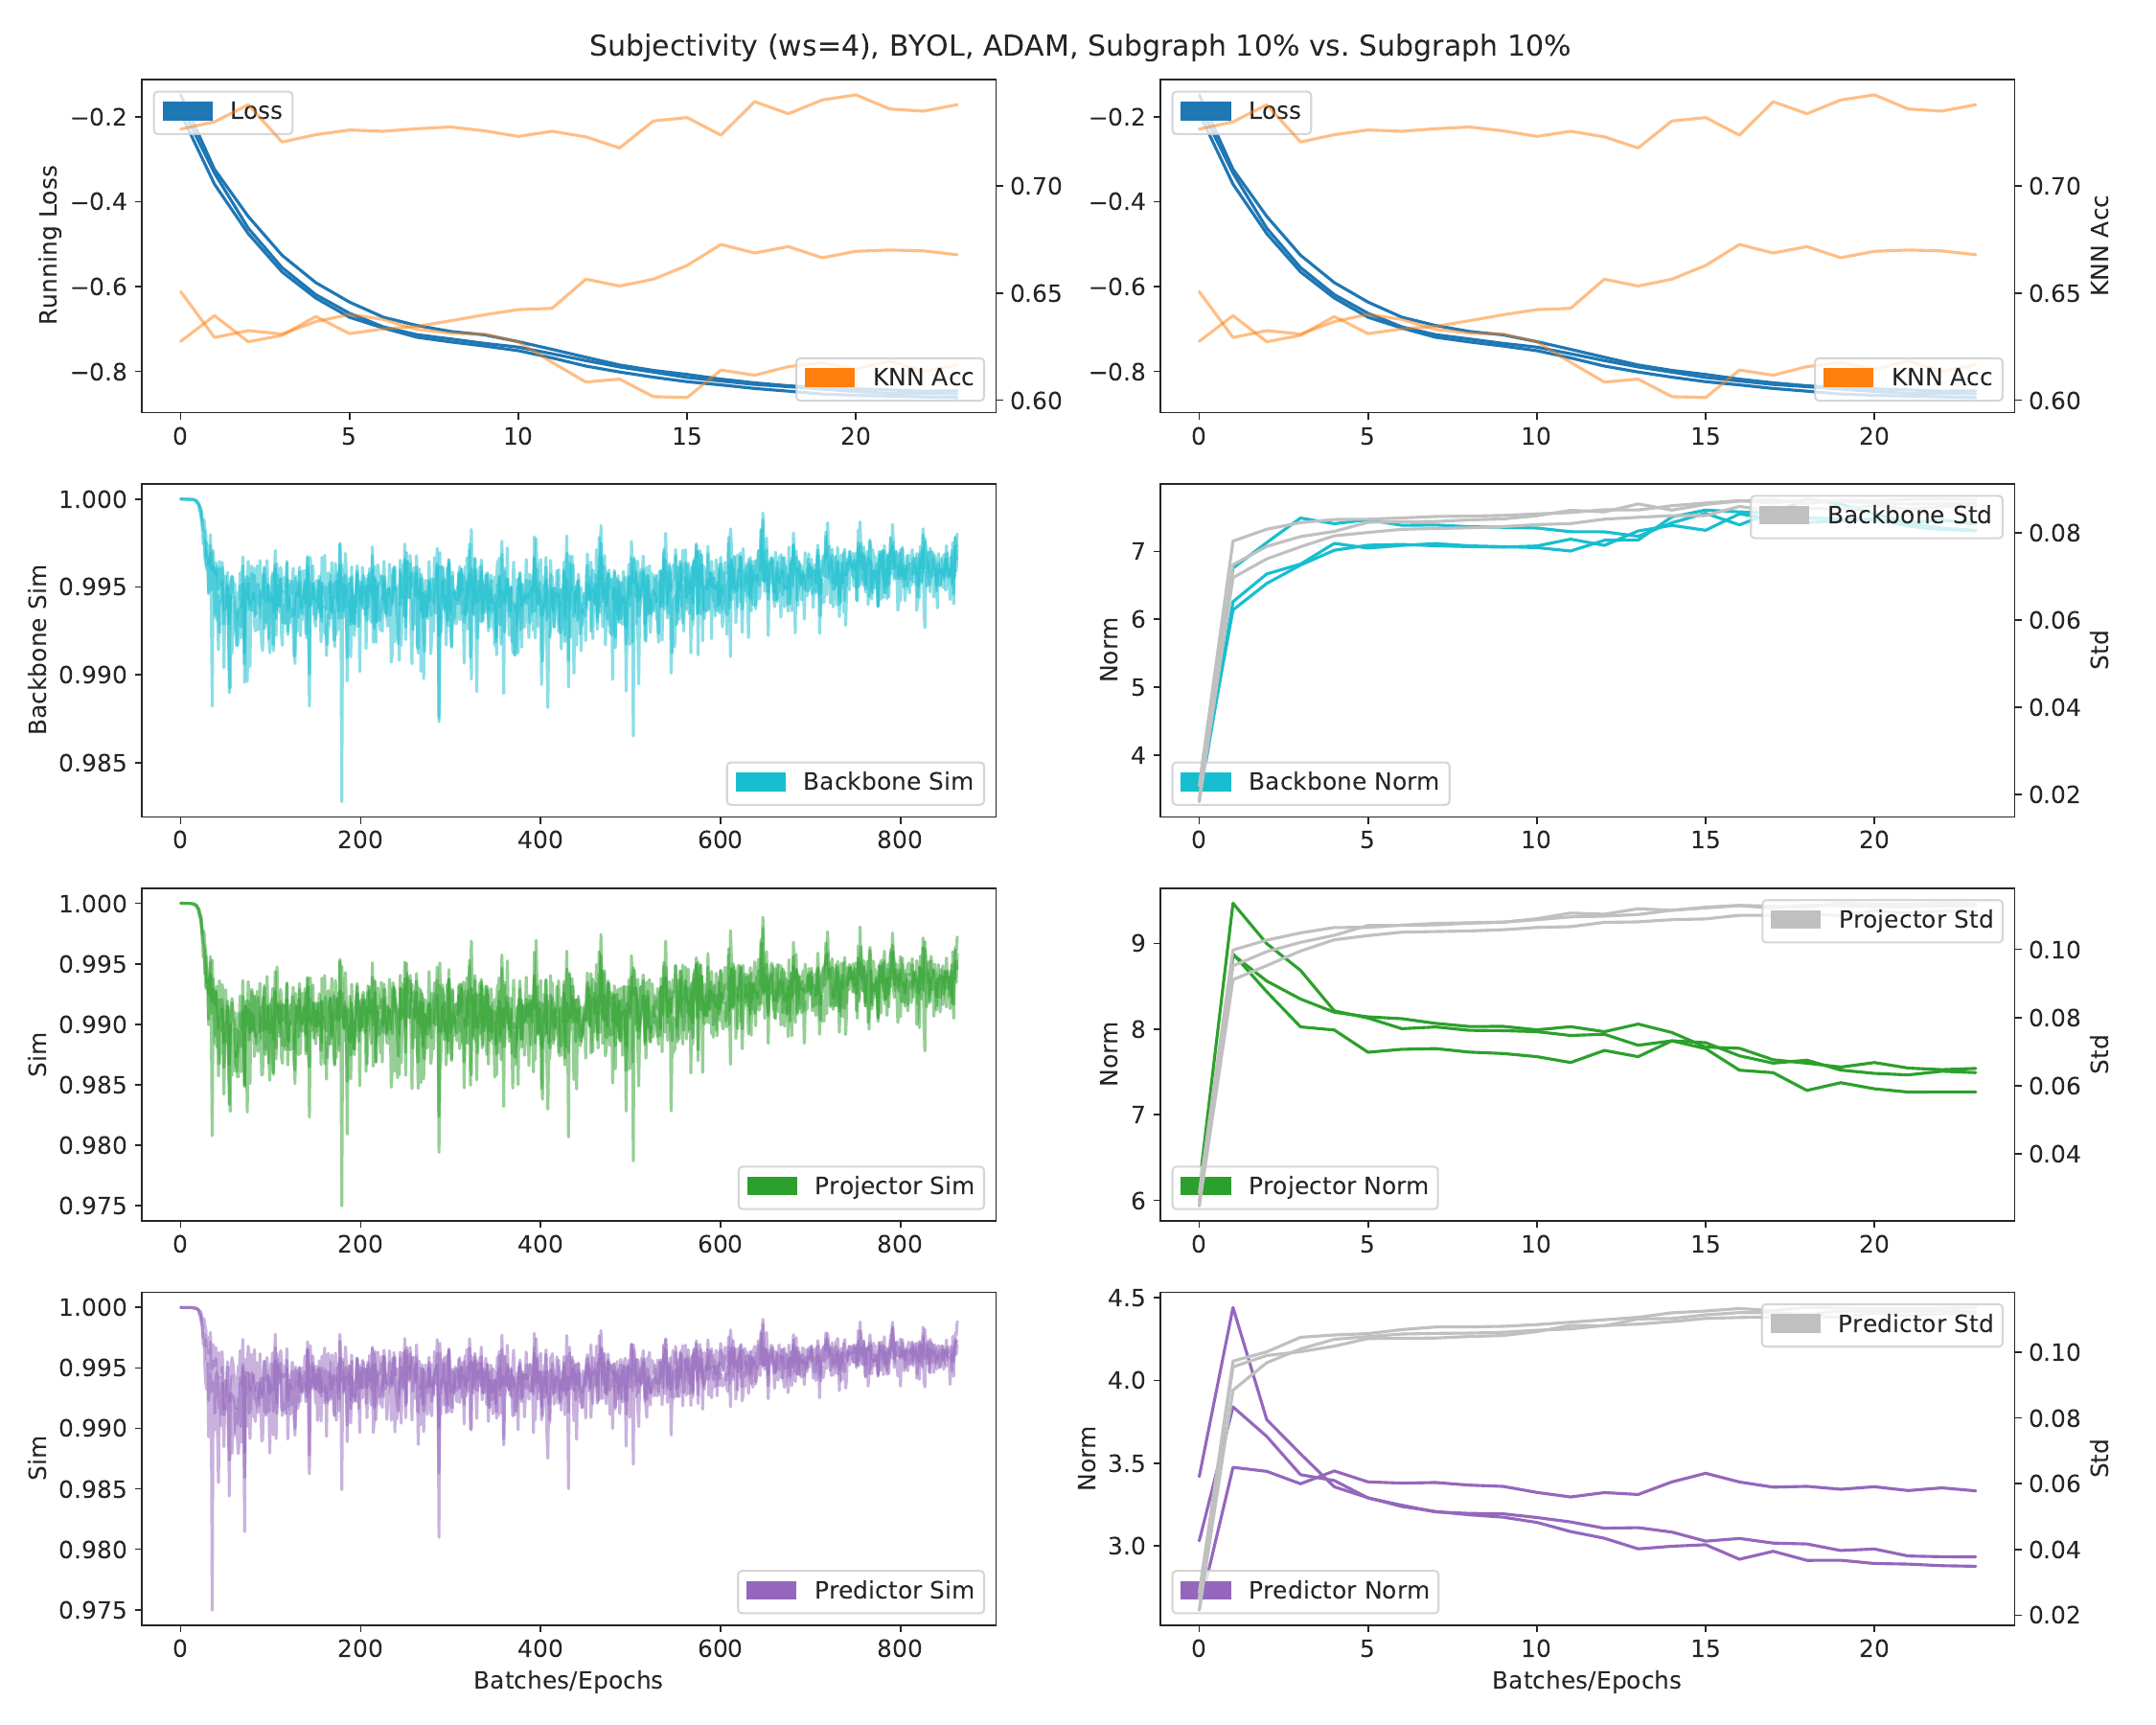}
    \caption{BYOL, WS=4, Subgraph 10\% vs. Subgraph 10\%}
    \label{fig:byol_nlp_ws4_sub10_v_sub10}
\end{figure}
\begin{figure}[H]
    \centering
    \includegraphics[width=0.8\textwidth]{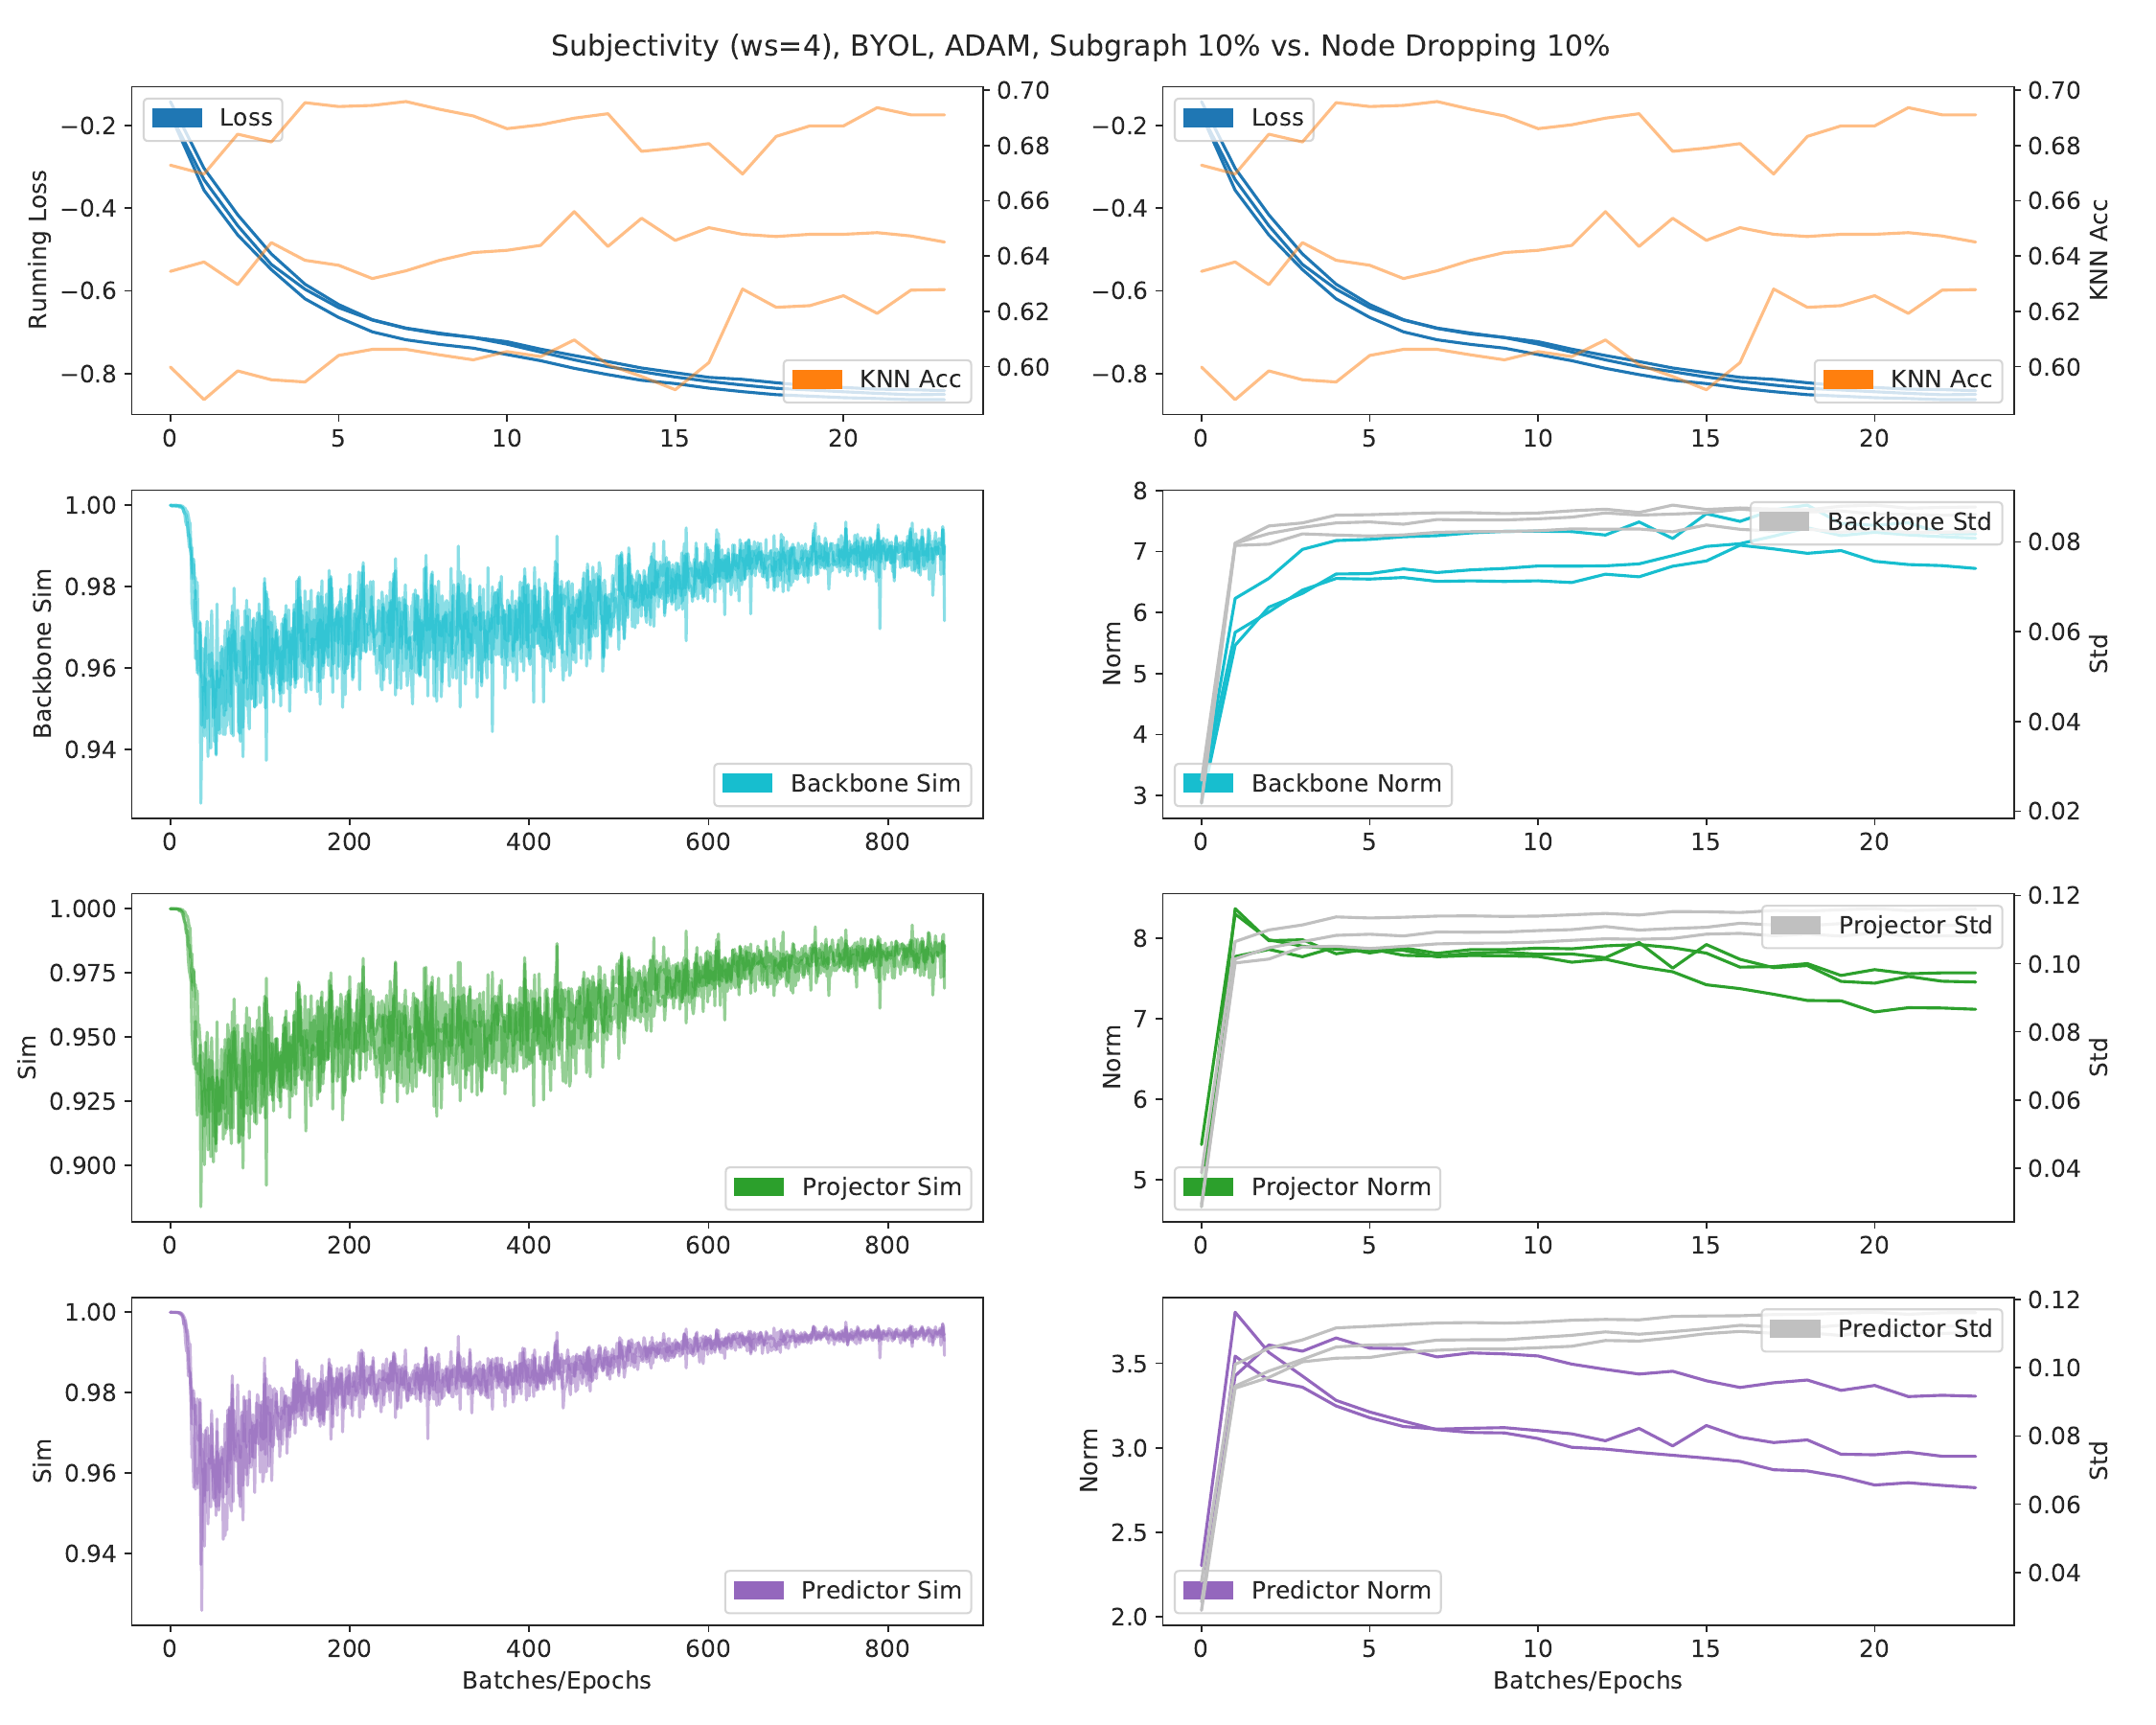}
    \caption{BYOL, WS=4, Subgraph 10\% vs. Node Dropping 10\%}
    \label{fig:byol_nlp_ws4_sub10_v_node10}
\end{figure}
