# Supplementary material for: Augmentations in Graph Contrastive Learning: Current Methodological Flaws & Towards Better Practices
Source: arXiv:2111.03220 source file (2022-03-11)
Supplement: Supplementary file 2 [file training_figures_superpixel.tex]

\subsection{SimSiam}\label{sec:app_mnist_simsiam}
In this section, we show results for superpixel classification using SimSiam (\cite{Chen20_SimSiam}), a positive-sample-only framework. We use the hyper-parameters discussed in Sec. \ref{sec:app_superpixel}. In Figs. (\ref{fig:simsiam_color},\ref{fig:simsiam_node_20}, \ref{fig:simsiam_node_30}), we plot KNN accuracy and loss as well as the norm, standard deviation, and similarity of backbone, encoder, and projector representations throughout training.
\begin{figure}[H]
\centering
\includegraphics[width=0.8\textwidth]{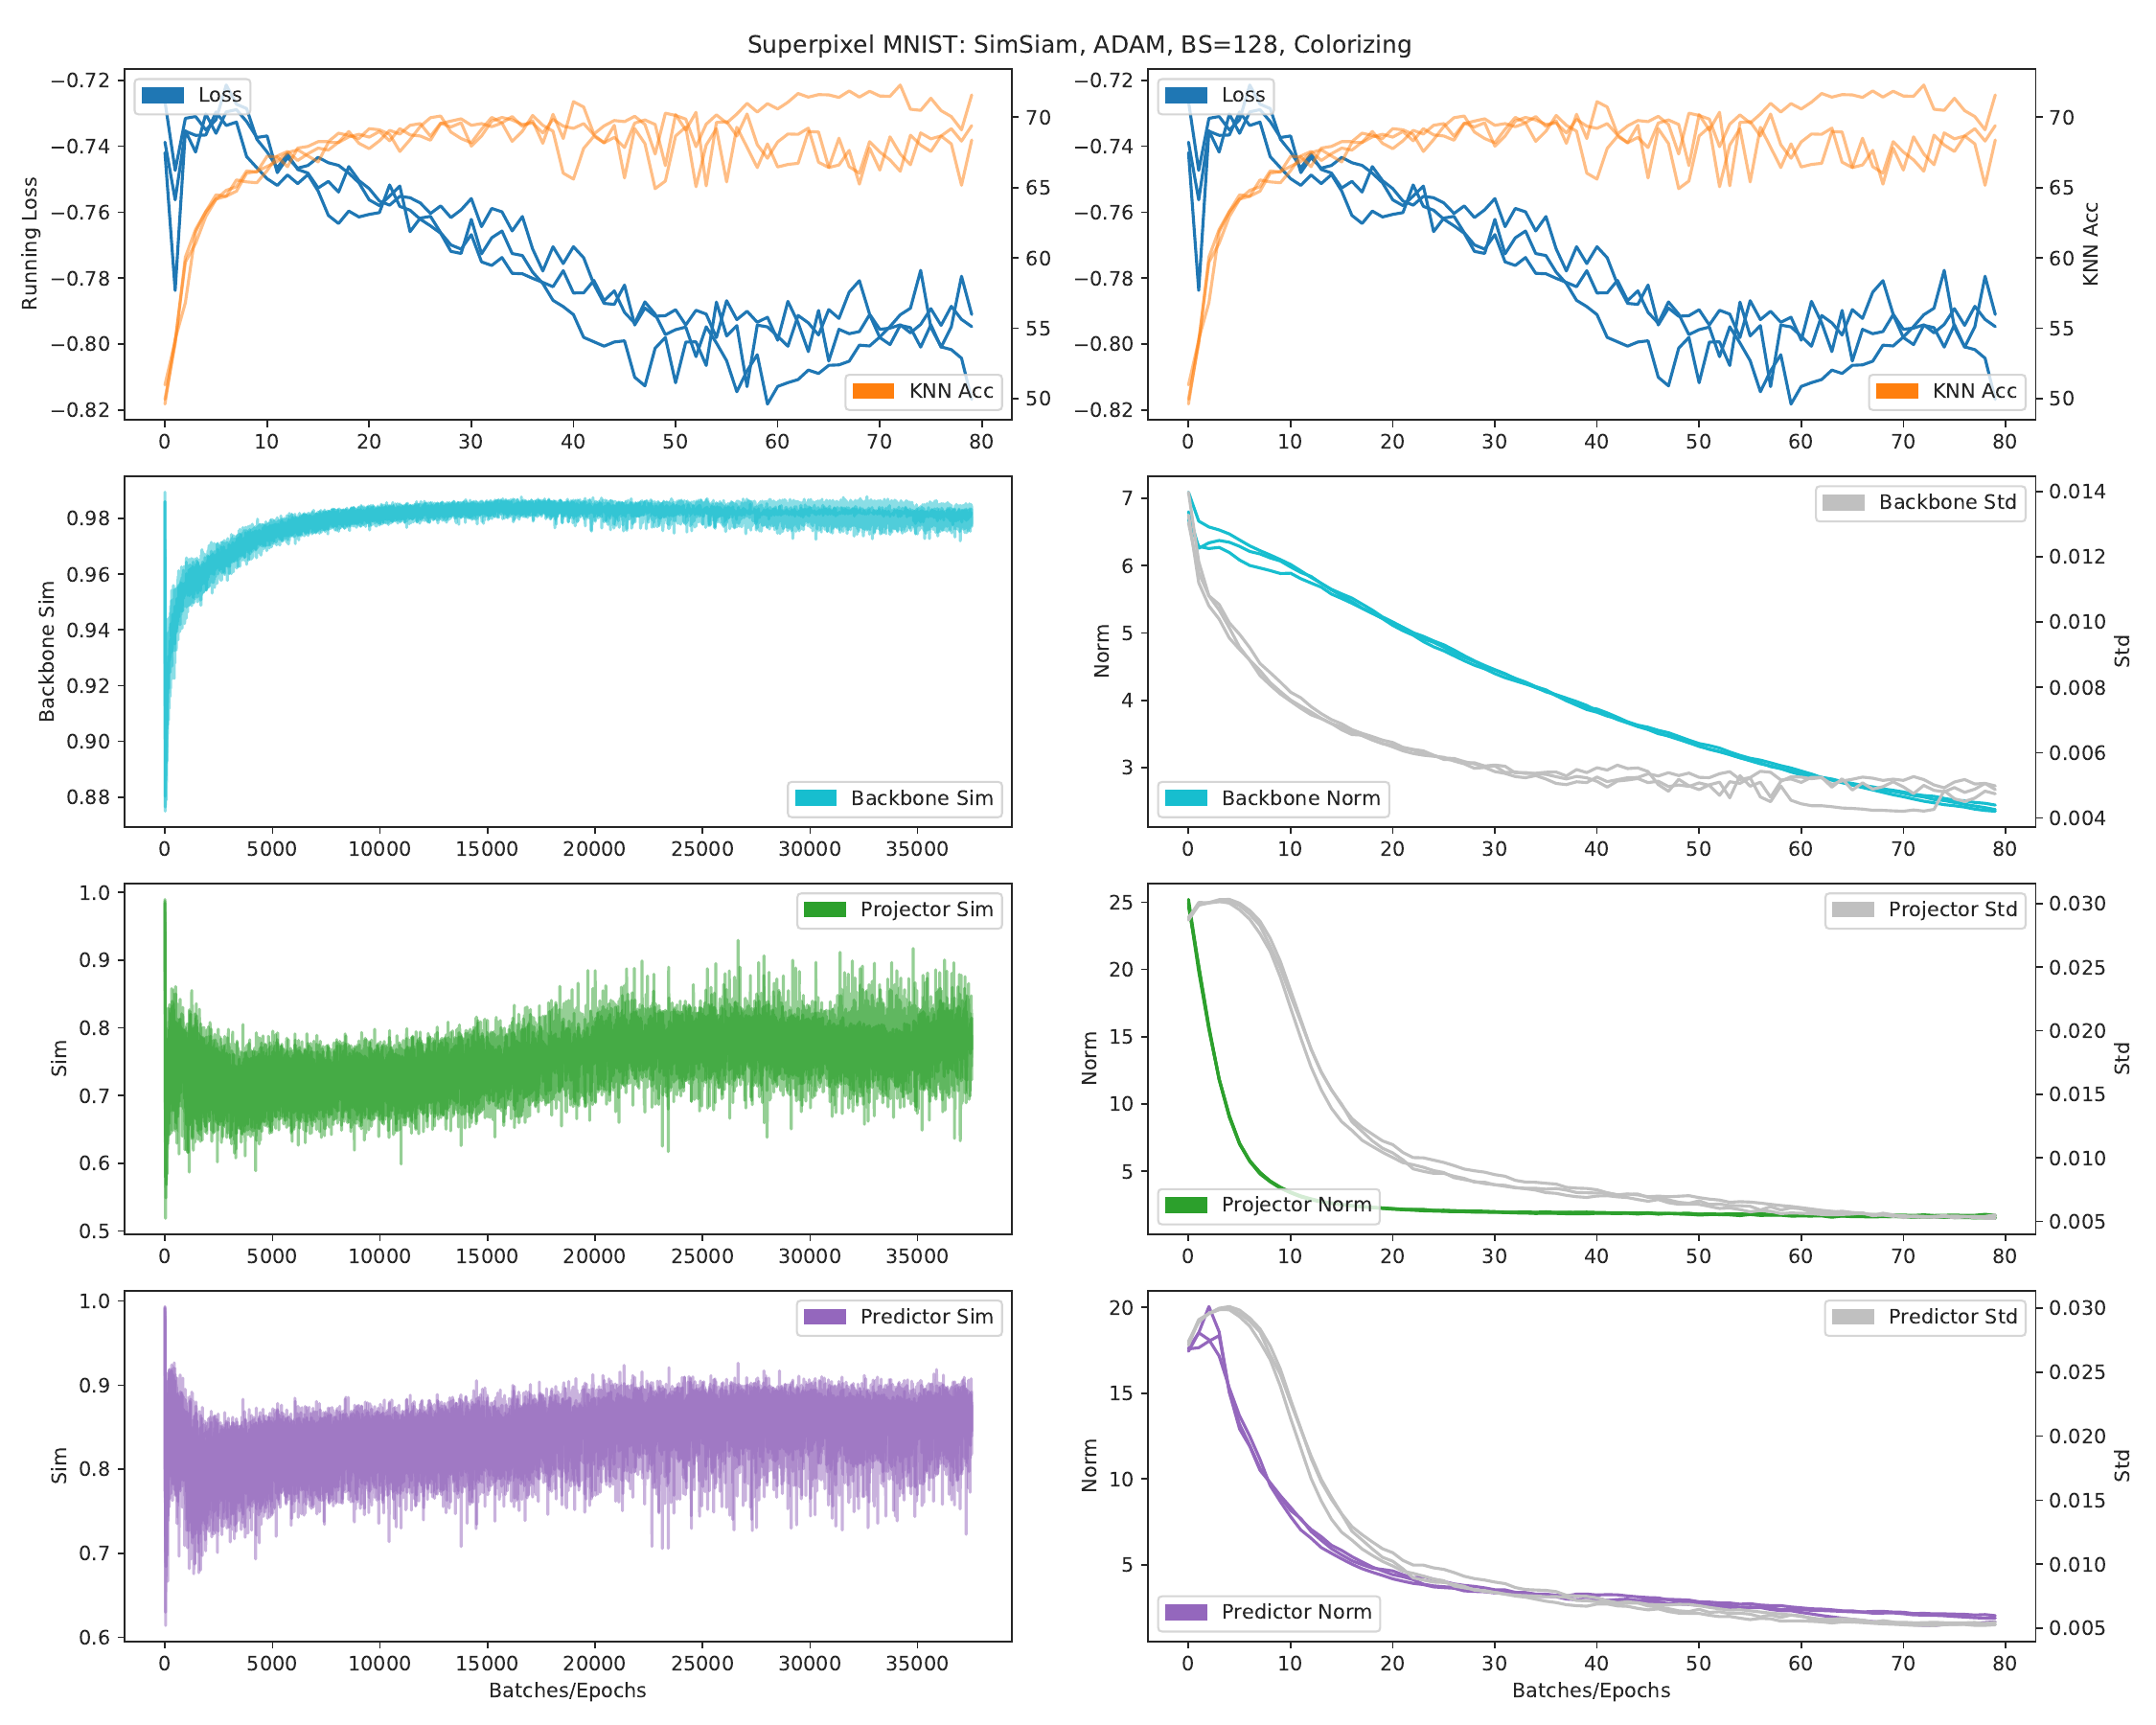}
\caption{SimSiam, Colorizing}
\label{fig:simsiam_color}
\end{figure}

\begin{figure}[H]
\centering
\includegraphics[width=0.8\textwidth]{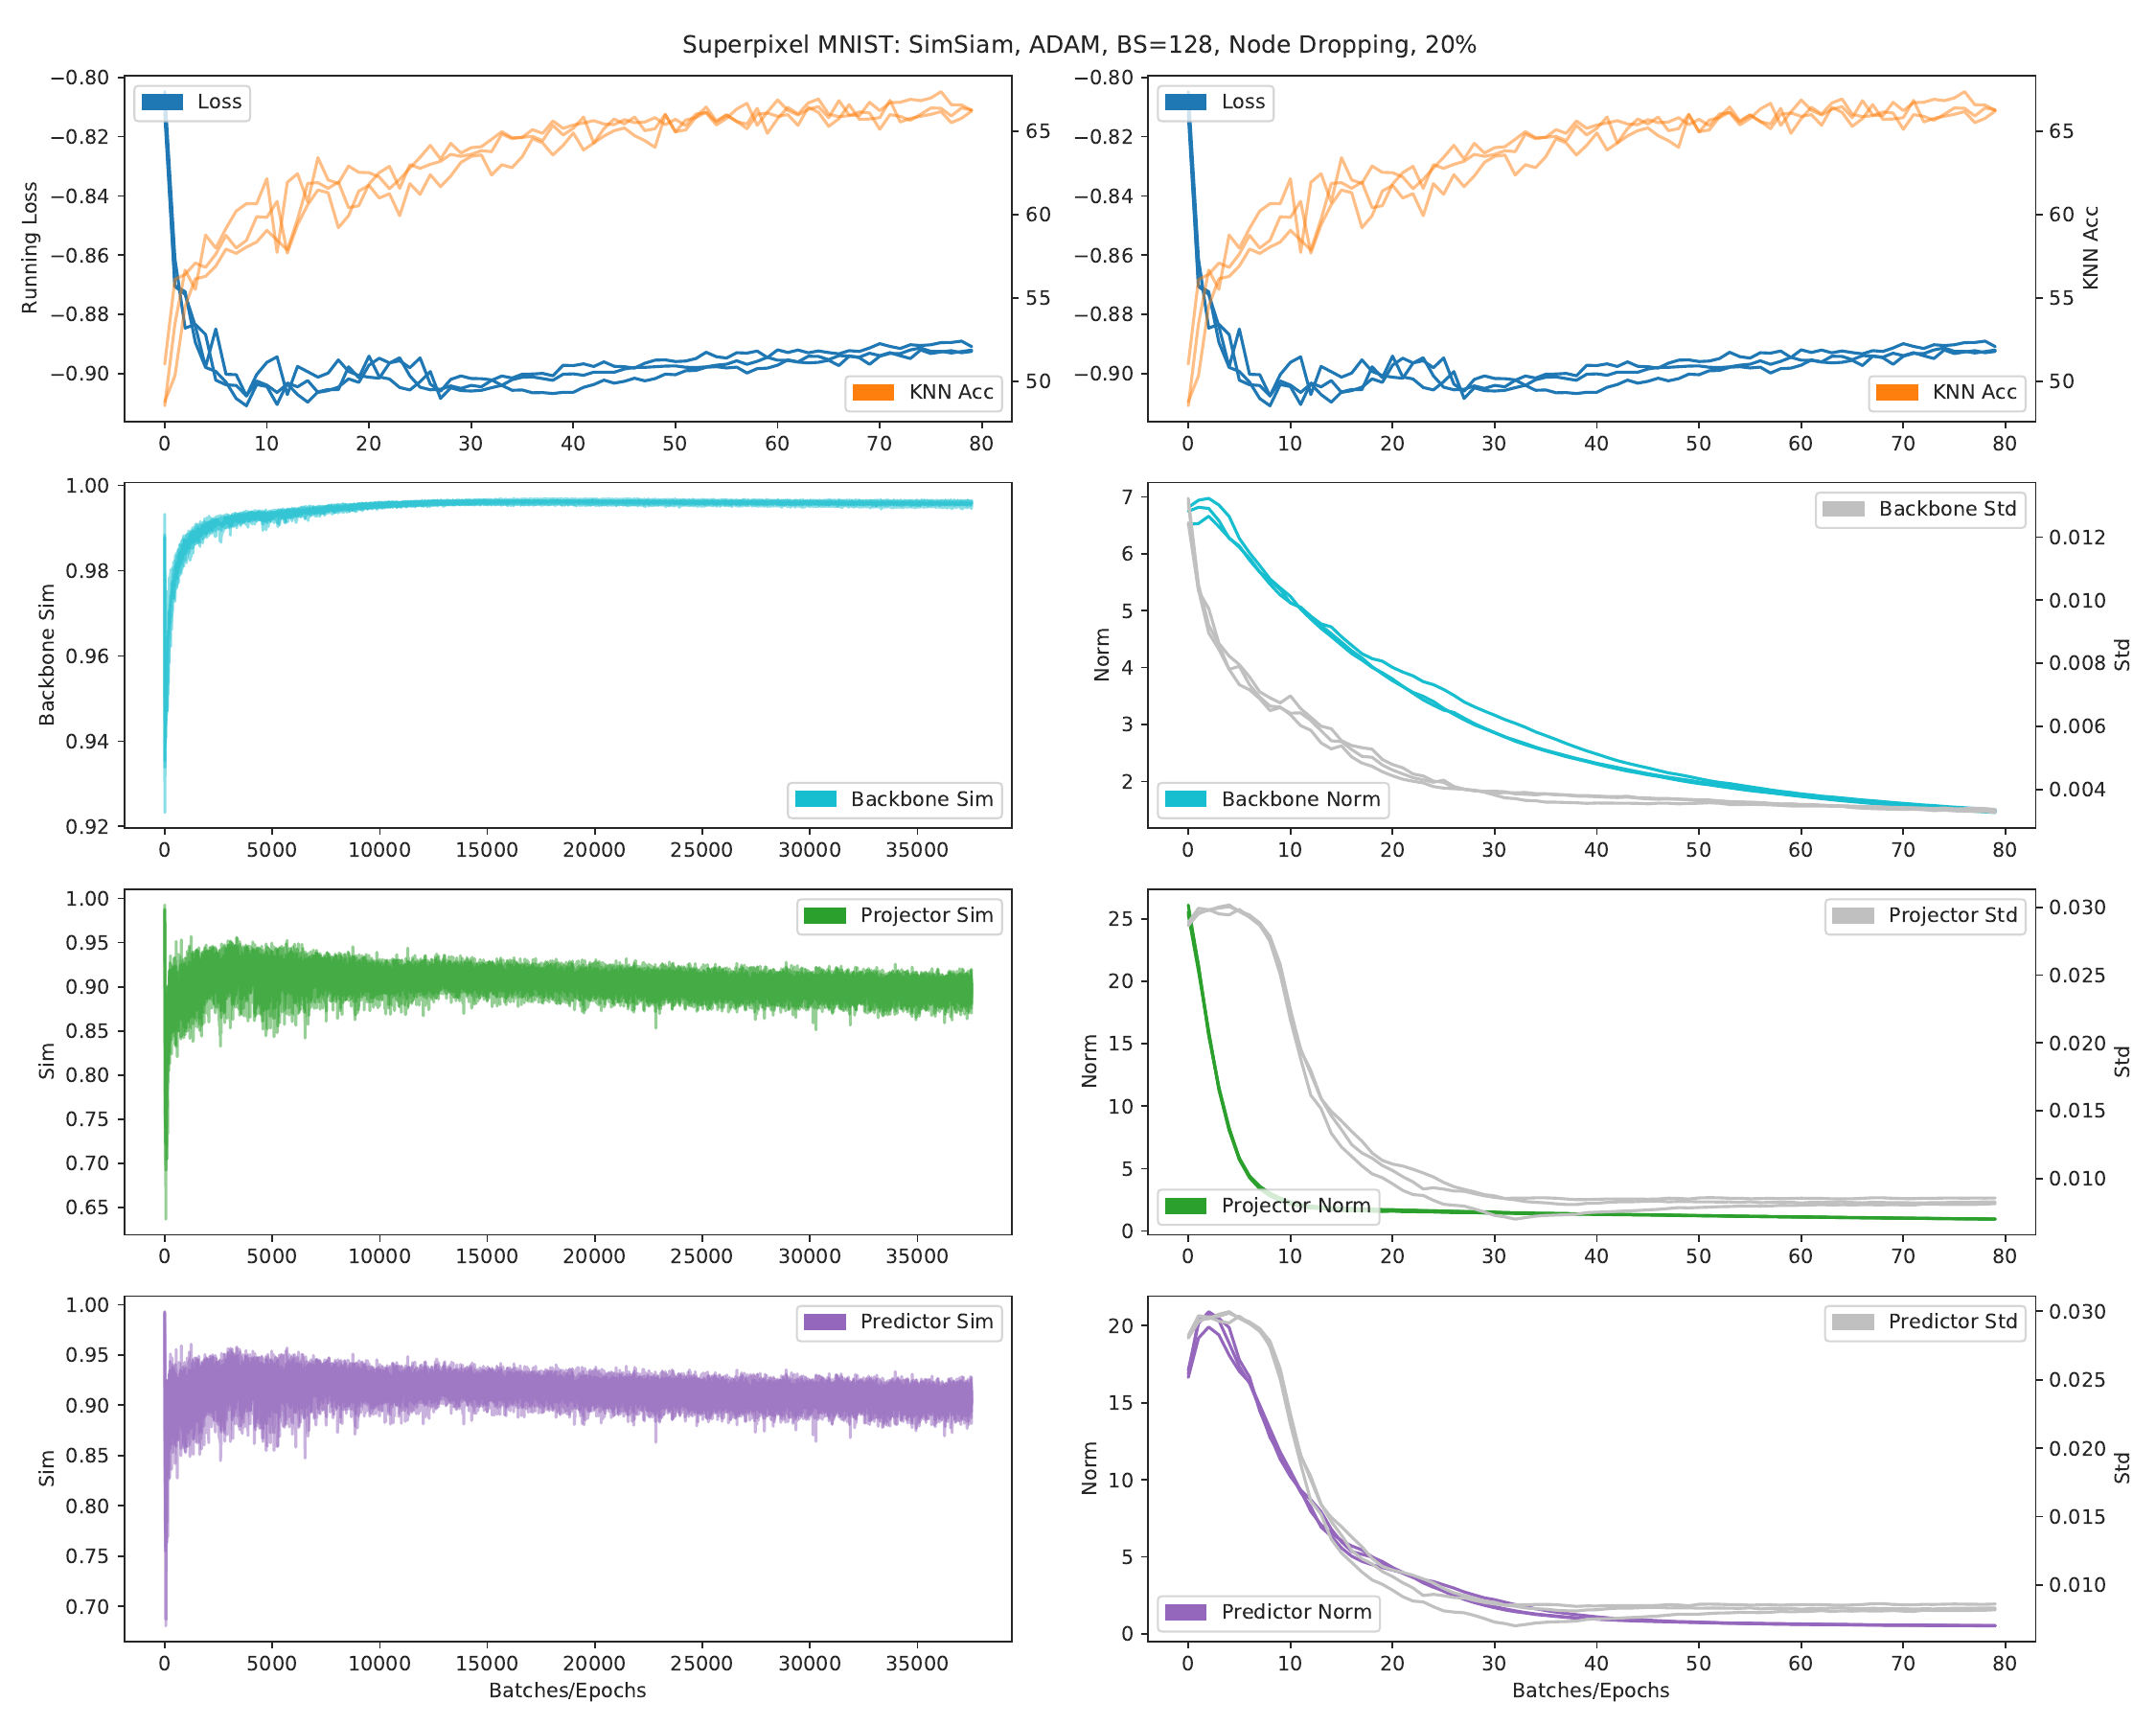}
\caption{SimSiam, Node Dropping 20\%}
\label{fig:simsiam_node_20}
\end{figure}

\begin{figure}[H]
\centering
\includegraphics[width=0.8\textwidth]{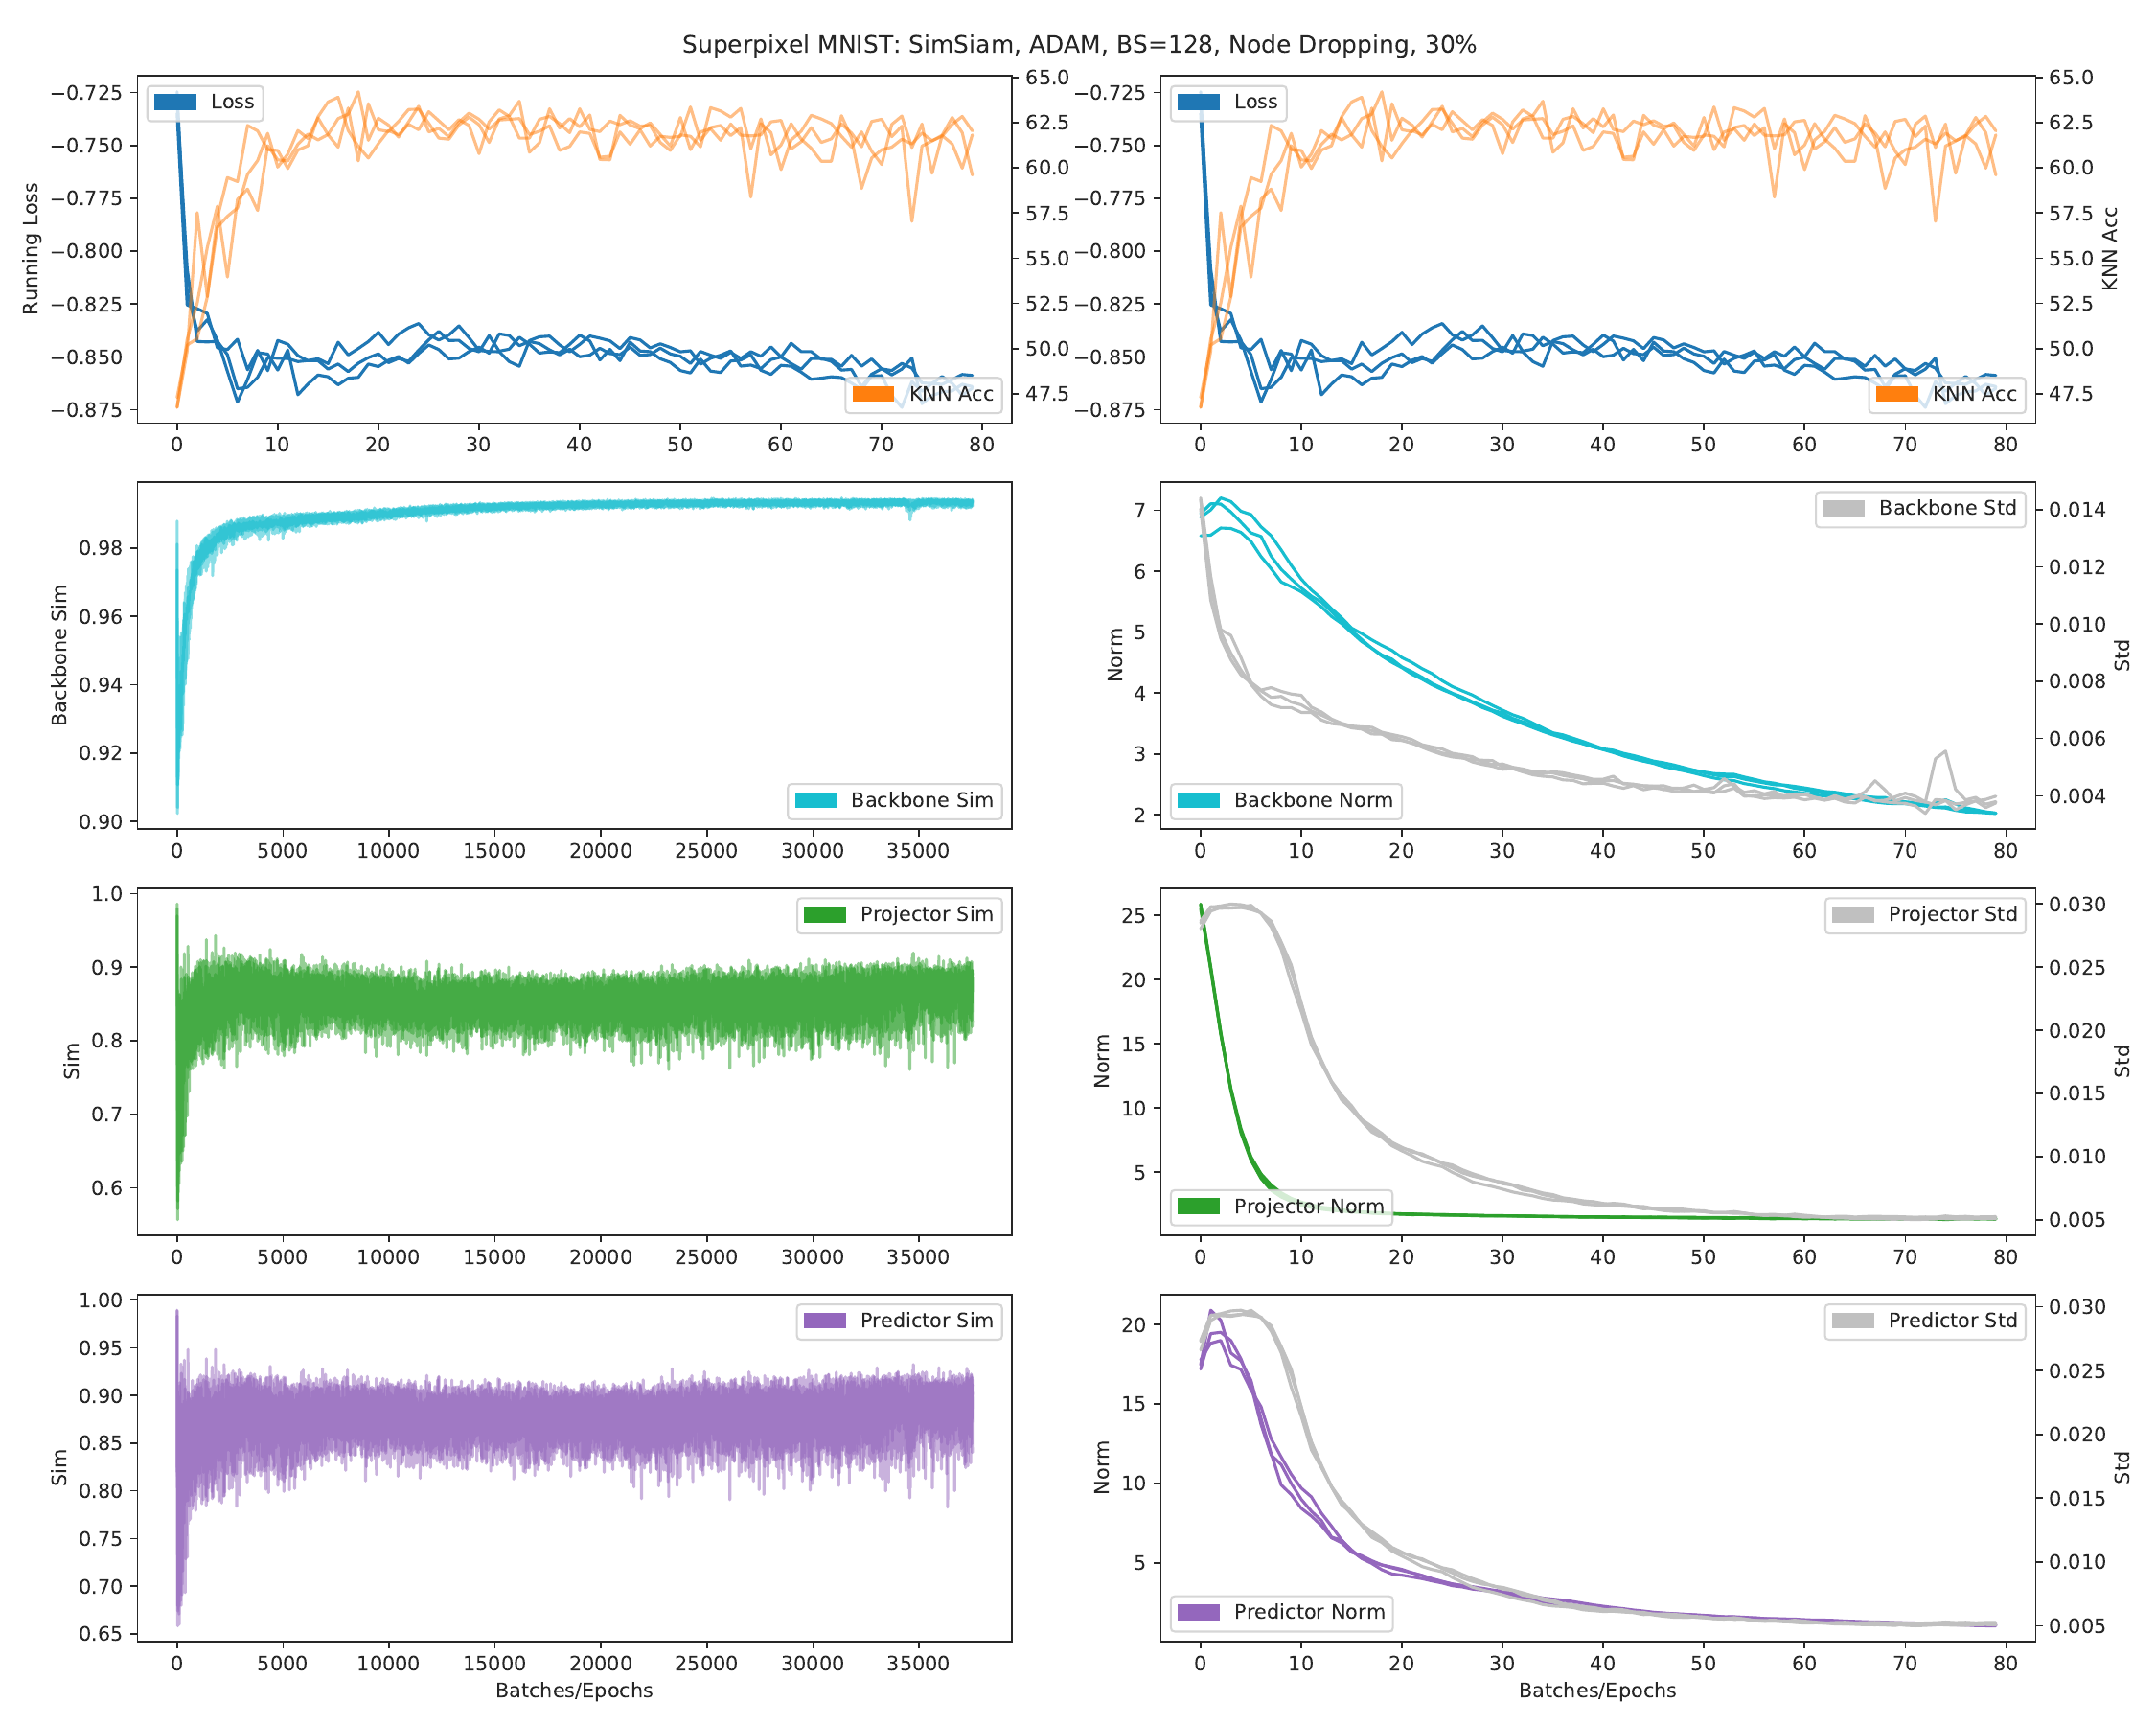}
\caption{SimSiam, Node Dropping 30\%}
\label{fig:simsiam_node_30}
\end{figure}

\newpage
\subsection{SimCLR}\label{sec:app_mnist_simclr}
In this section, we show results for superpixel classification using SimCLR (\cite{Chen20_SimCLR}), a negative-sample framework.  We use the hyper-parameters discussed in Sec. \ref{sec:app_superpixel}. In Figs. (\ref{fig:simclr_color},\ref{fig:simclr_node_20},\ref{fig:simclr_node_30}), we plot KNN accuracy and loss as well as the norm, standard deviation, and similarity of backbone, encoder, and projector representations throughout training. 
\begin{figure}[H]
\centering
\includegraphics[width=0.8\textwidth]{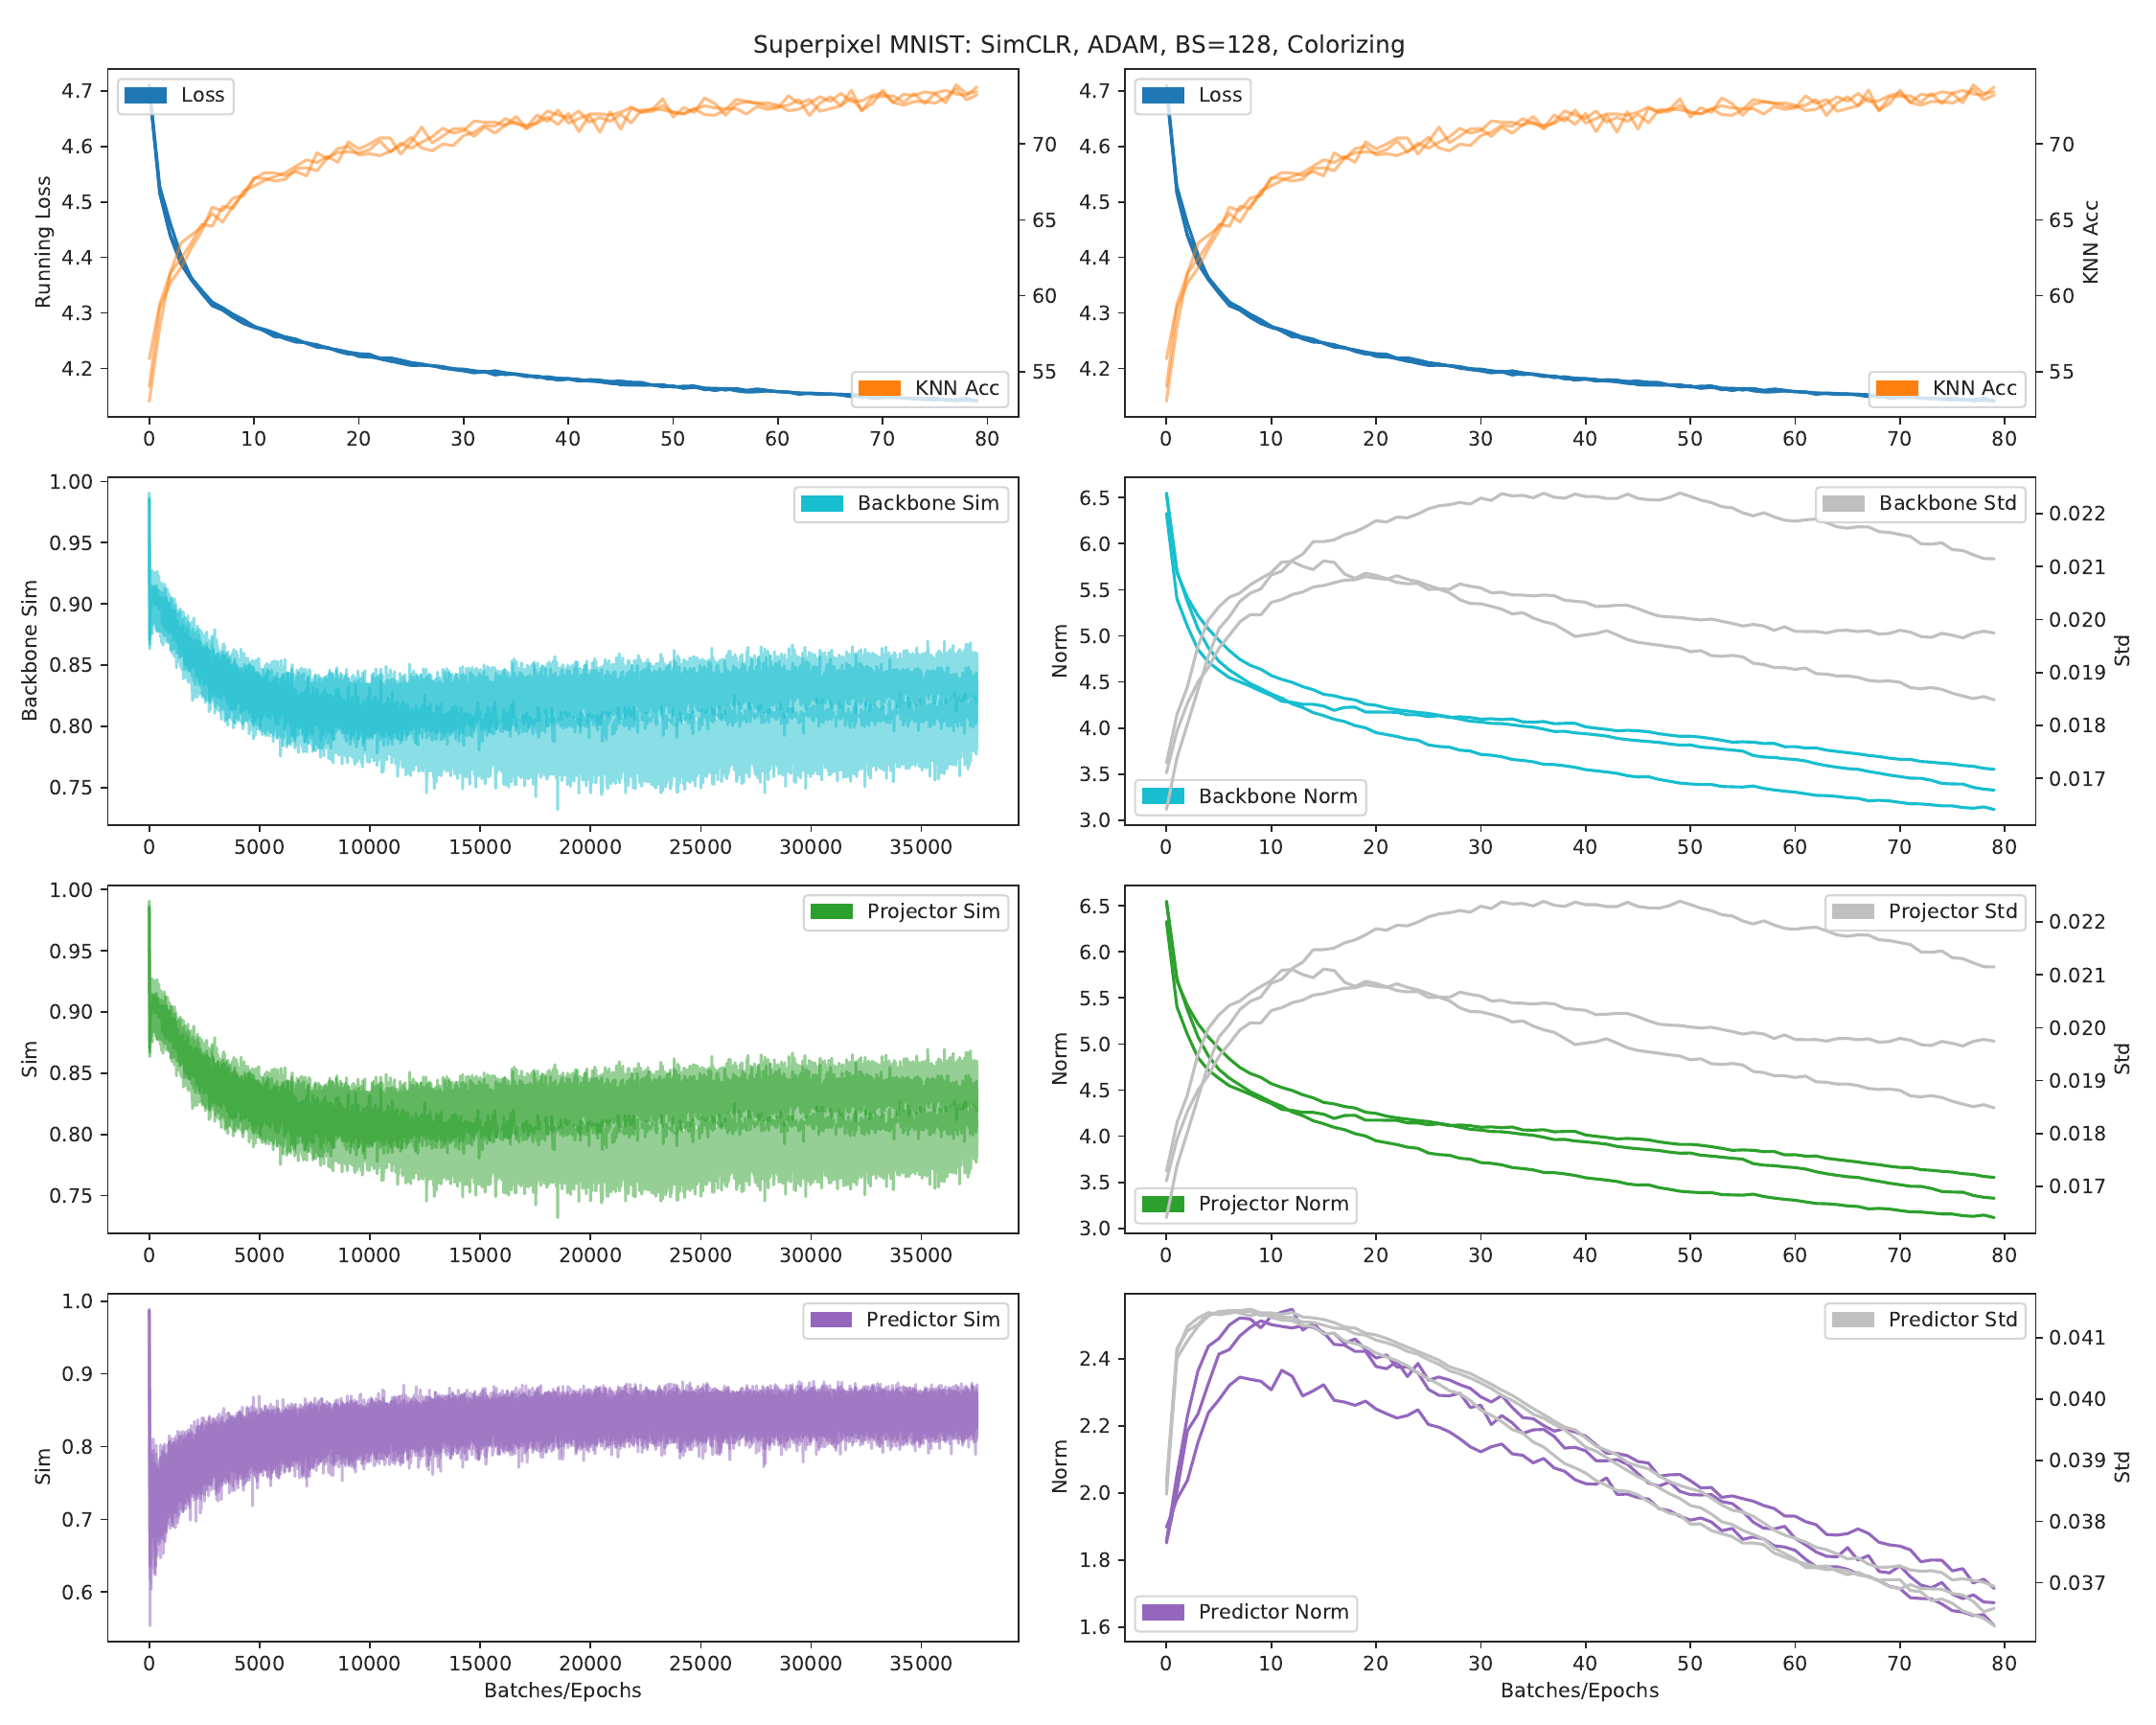}
\caption{SimCLR, Colorizing}
\label{fig:simclr_color}
\end{figure}

\begin{figure}[H]
    \centering
    \includegraphics[width=0.8\textwidth]{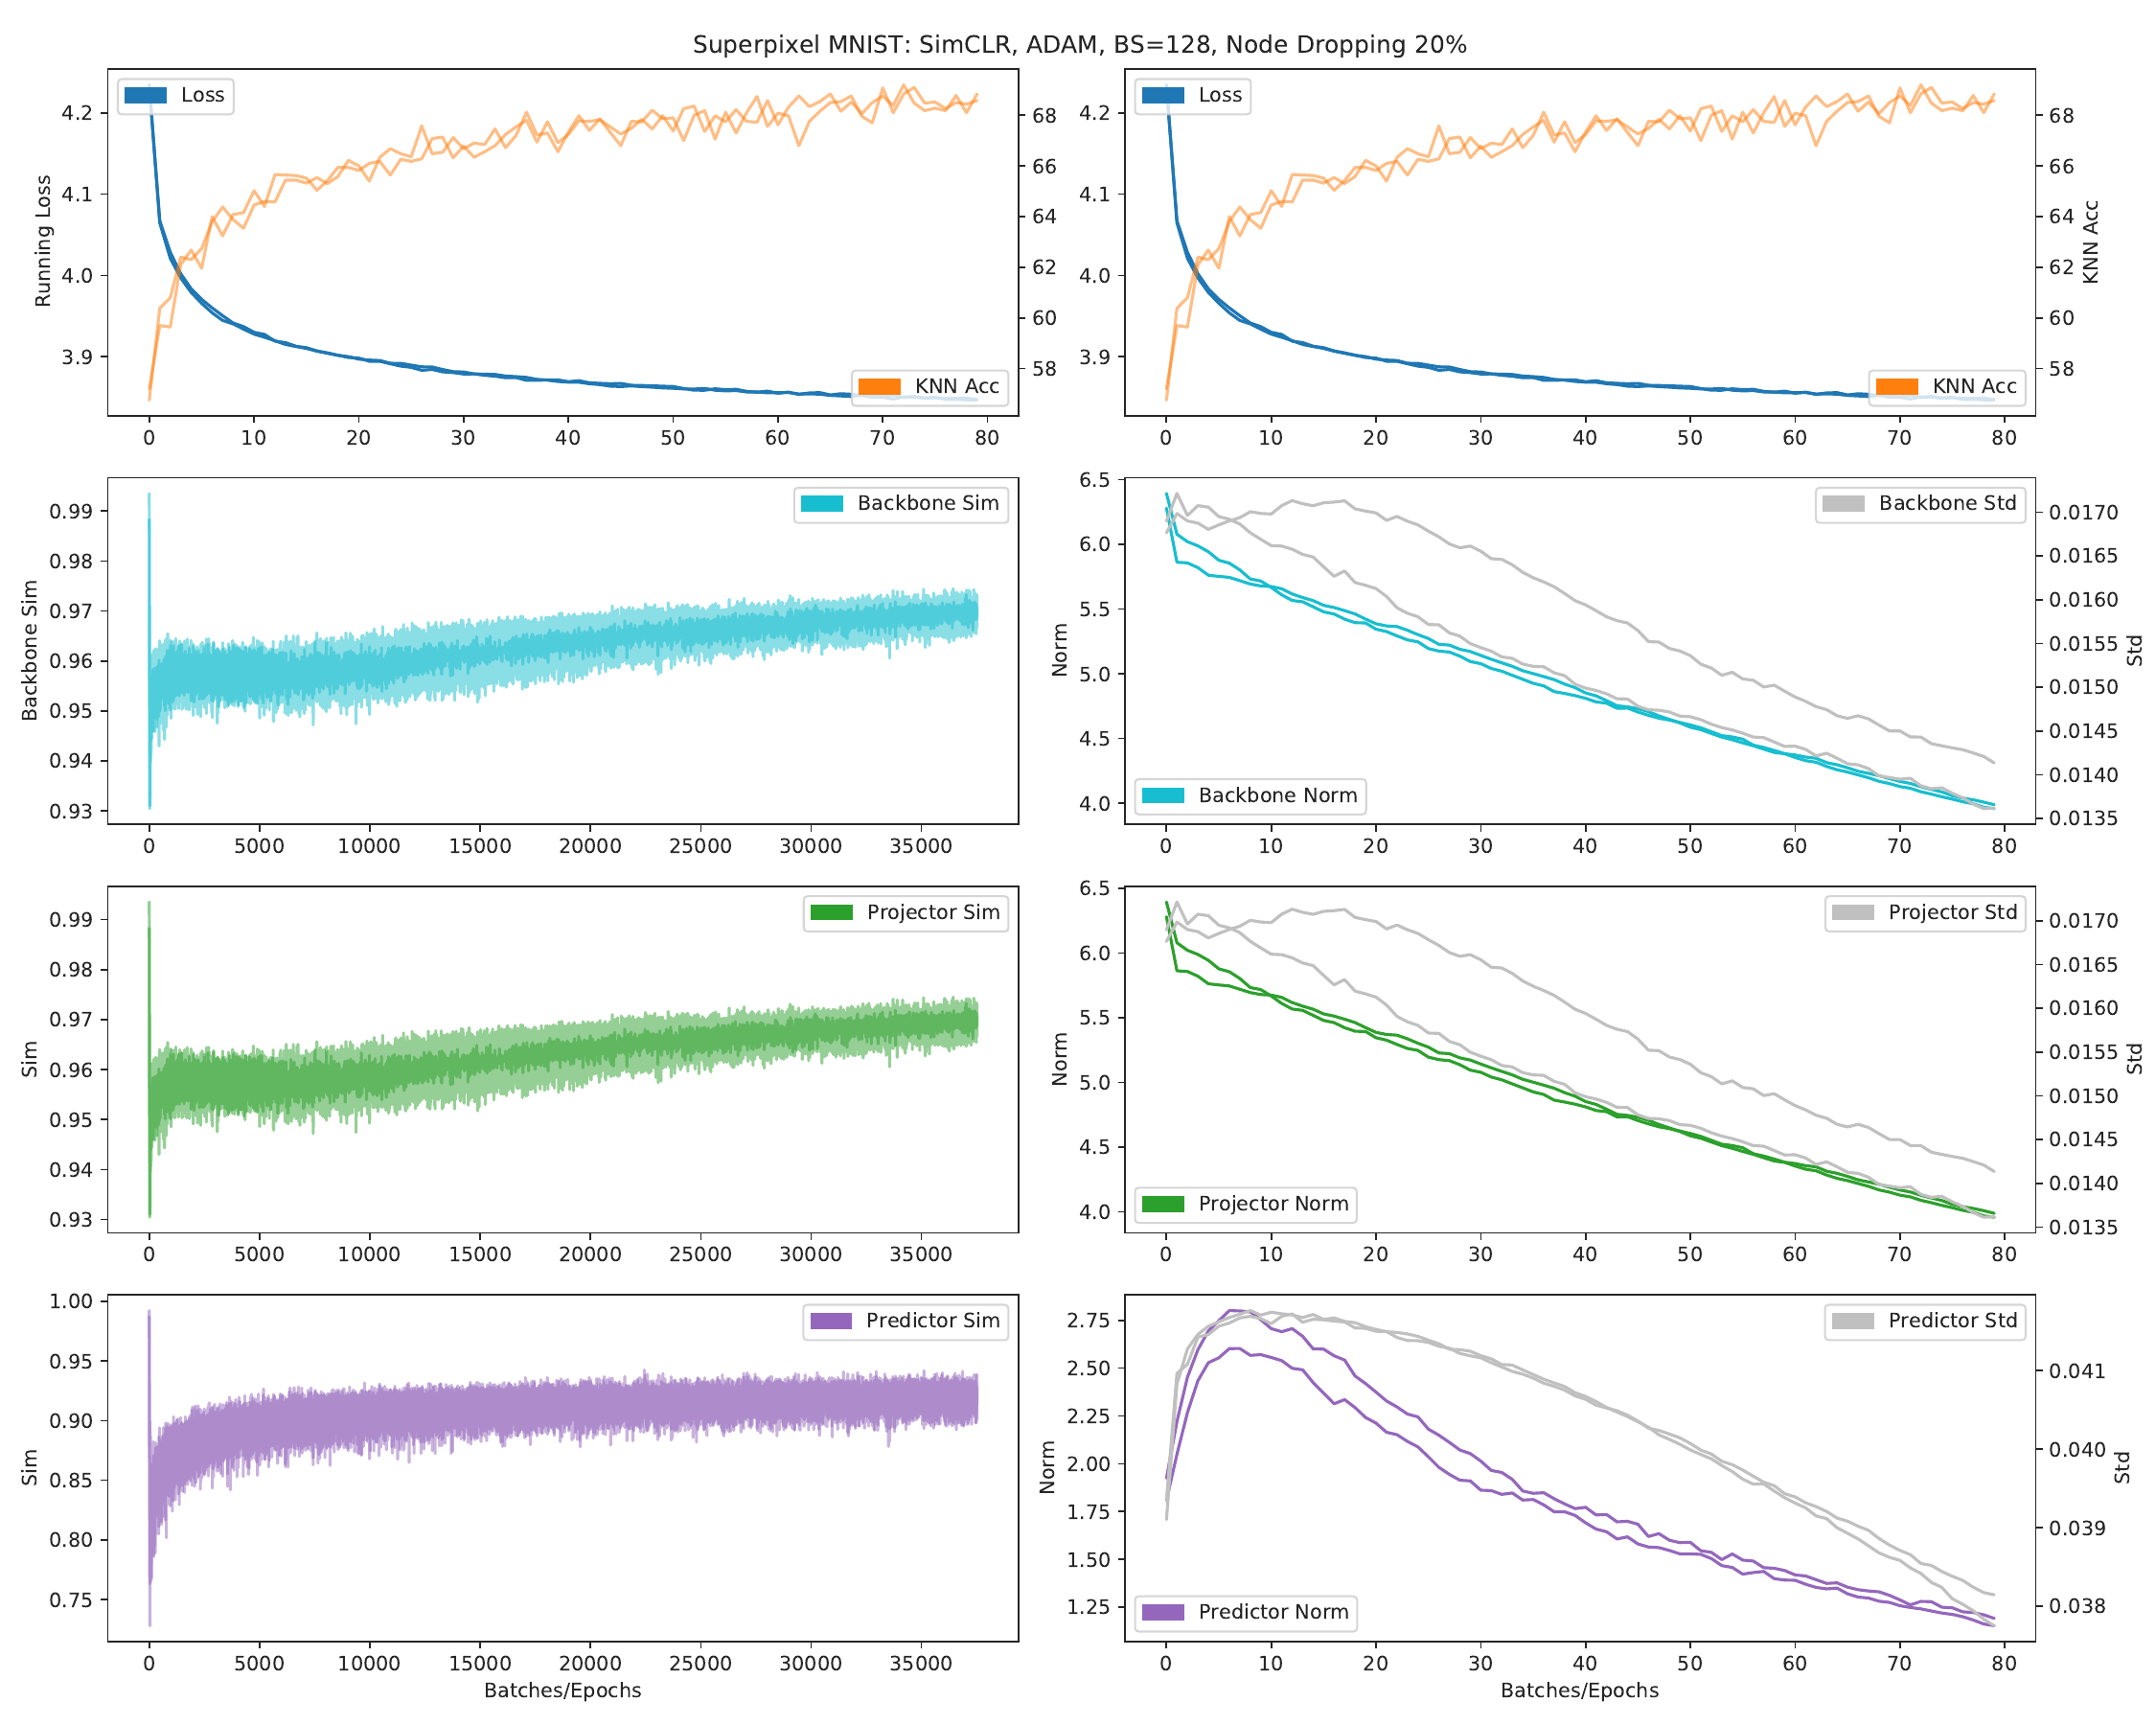}
    \caption{SimCLR, Node Dropping 20\%}
    \label{fig:simclr_node_20}
\end{figure}
\begin{figure}[H]
    \centering
    \includegraphics[width=0.8\textwidth]{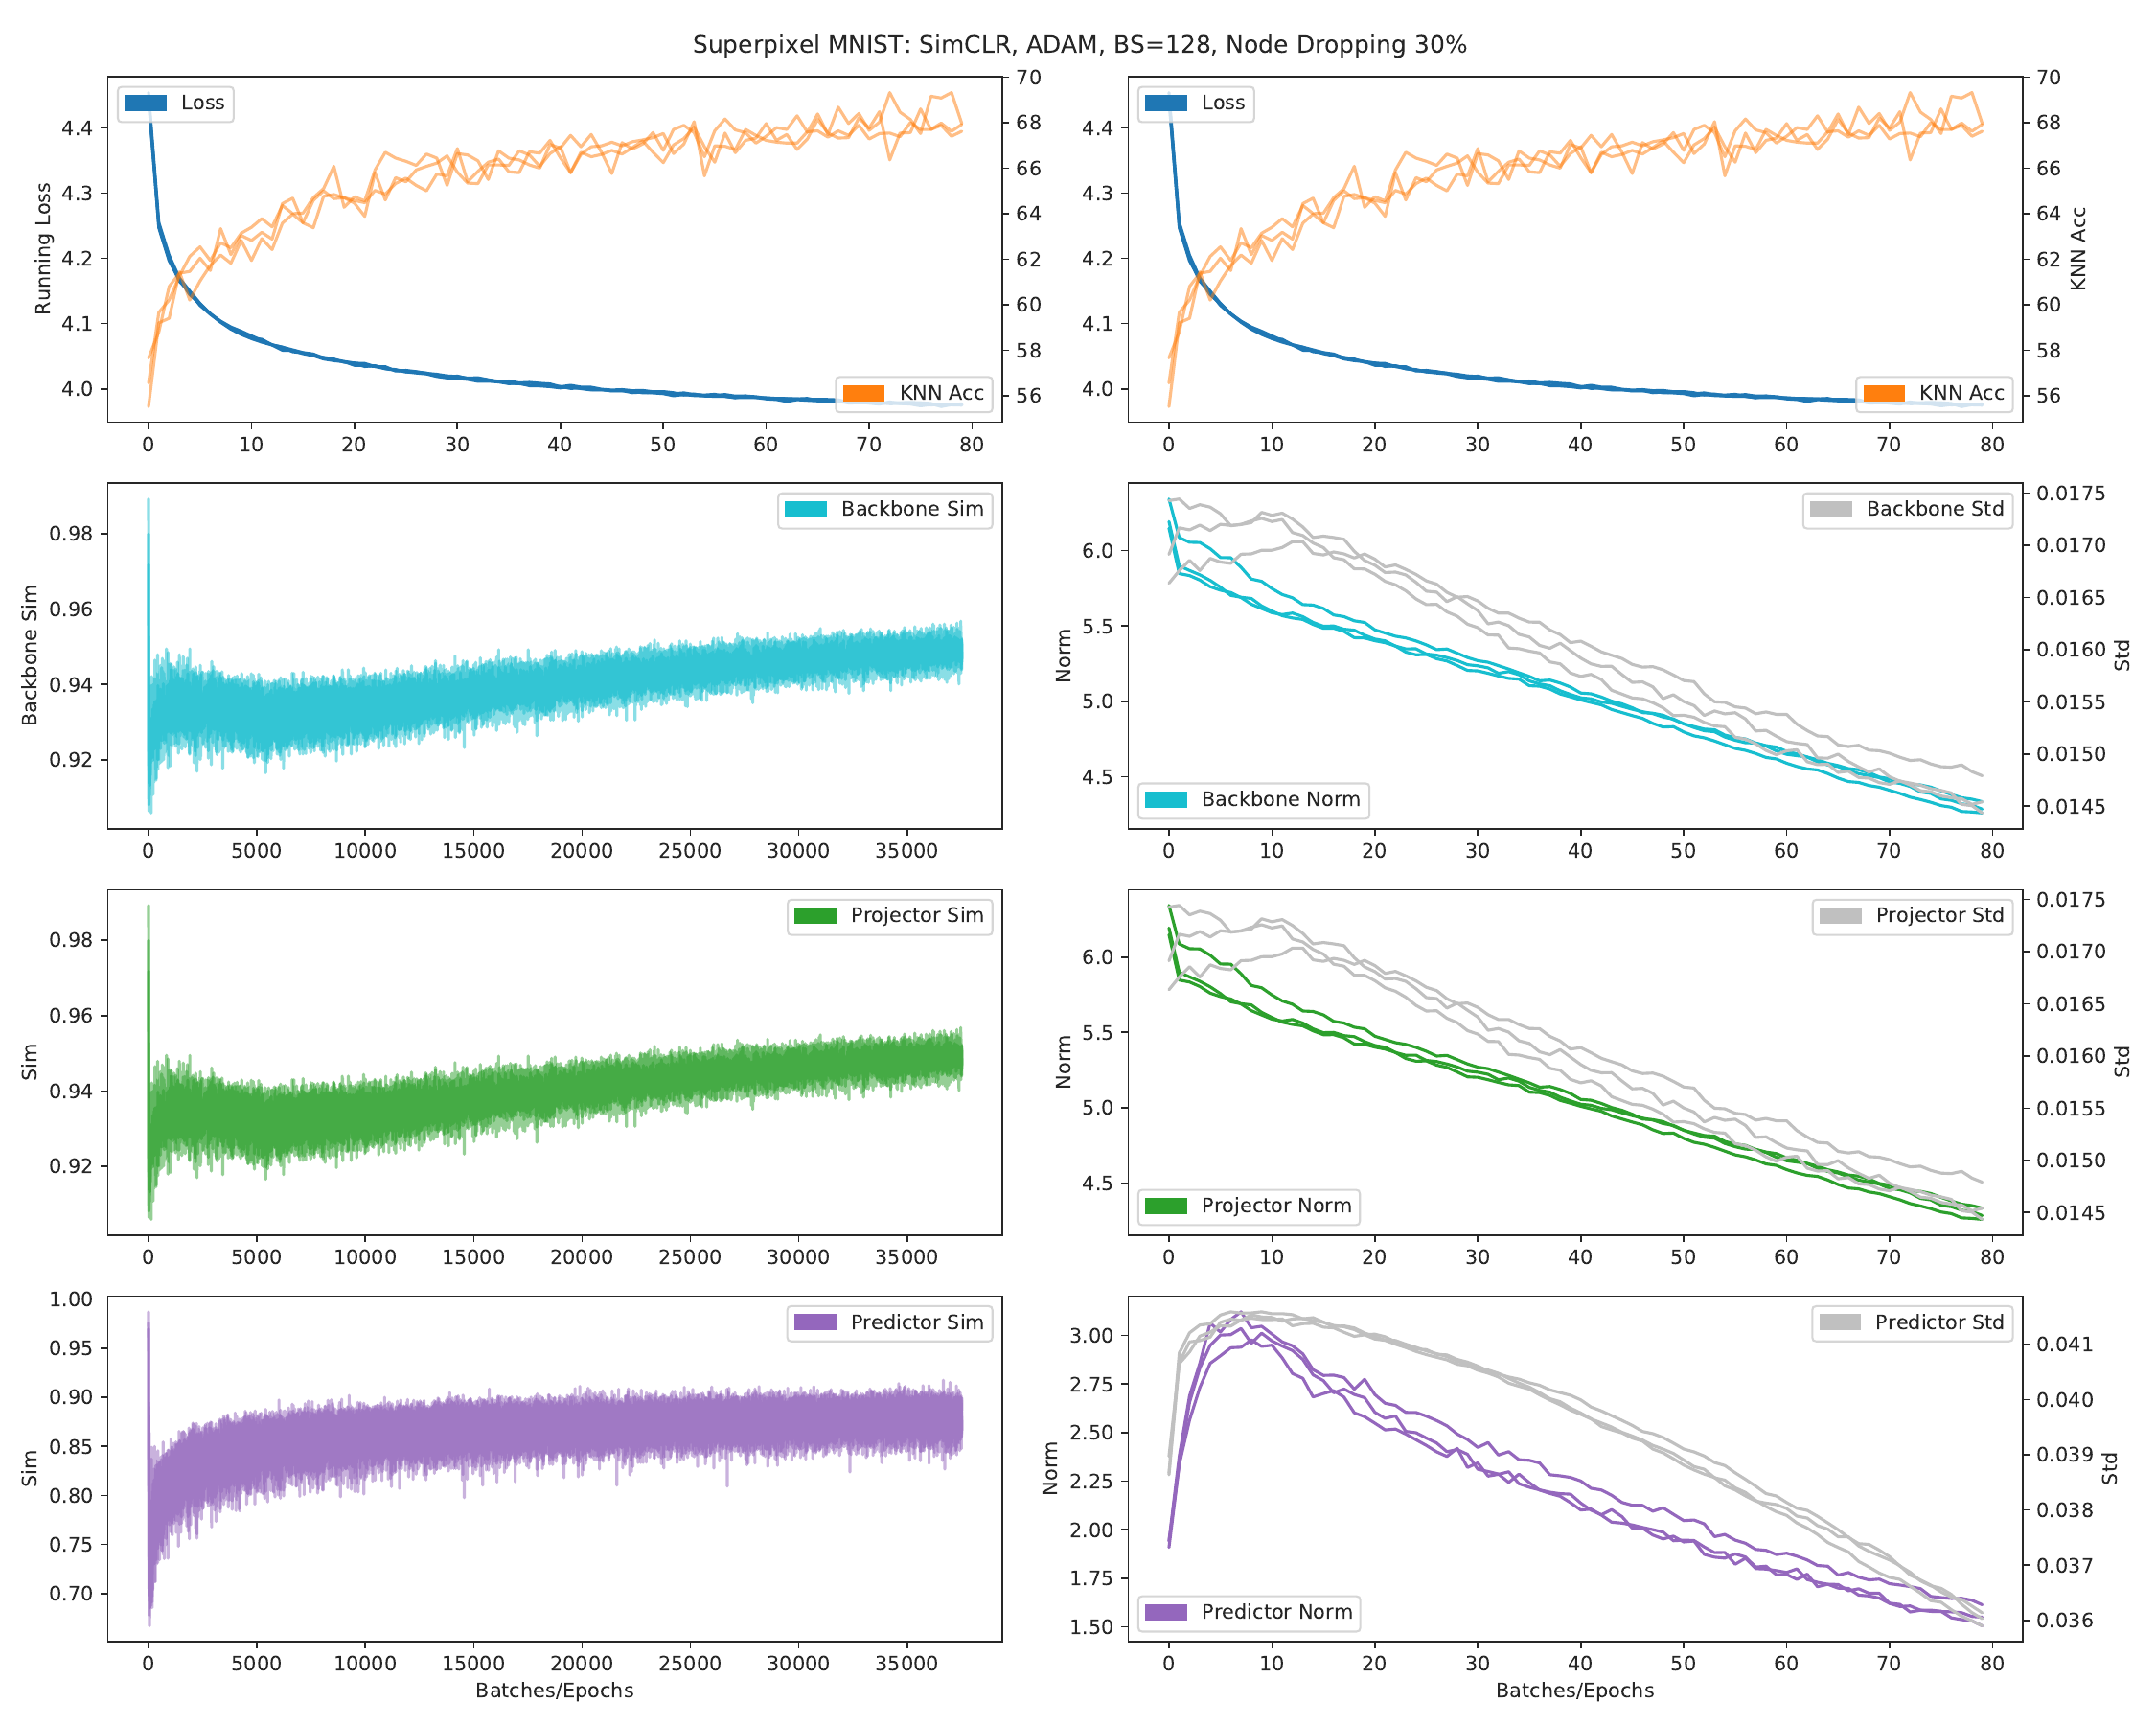}
    \caption{SimCLR, Node Dropping 30\%}
    \label{fig:simclr_node_30}
\end{figure}

\newpage
\subsection{BYOL}\label{sec:app_mnist_byol}
In this section, we show results for superpixel classification using BYOL (\cite{Grill20_BYOL}), a positive-sample-only framework.  We use the hyper-parameters discussed in Sec. \ref{sec:app_superpixel} and BYOL's performance for different batch-sizes in \autoref{tab:app_superpixel}. In Figs. (\ref{fig:byol_color}, \ref{fig:byol_node_20}, \ref{fig:byol_node_30}), we plot KNN accuracy and loss as well as the norm, standard deviation, and similarity of backbone, encoder, and projector representations throughout training. 

\begin{table}[h!]
\small
 \caption{\textbf{Superpixel Classification.} Accuracy of randomly initialized model is $37.79 \pm 0.03$. We report BYOL's performance at different batch-sizes.}
 \label{tab:app_superpixel}
 \centering
 \resizebox{.5\textwidth}{!}{
 \begin{tabular}{c c c} 
\toprule
  \textbf{Batchsize} & \textbf{Node Dropping 20\%} & \textbf{Colorize} \\
    \cmidrule(r){1-3}
  1024  & $58.68 \pm 1.71$  & $49.19 \pm 4.01$ \\
  512  & $54.33 \pm 2.16$  & $43.92 \pm 7.76$ \\
  %256 & $57.76 \pm 0.97$  & -\\
  128 & $65.32 \pm 0.95$ & $64.42 \pm 2.385$\\
  SimCLR & $68.56 \pm 0.16 $  & $73.67 \pm 0.10$ \\
  SimSiam & $66.30 \pm 0.33$  & $68.95 \pm 1.20$ \\
\bottomrule
\end{tabular}}
\vspace{2cm}
\end{table}

\begin{figure}[h]
\centering
\includegraphics[width=0.8\textwidth]{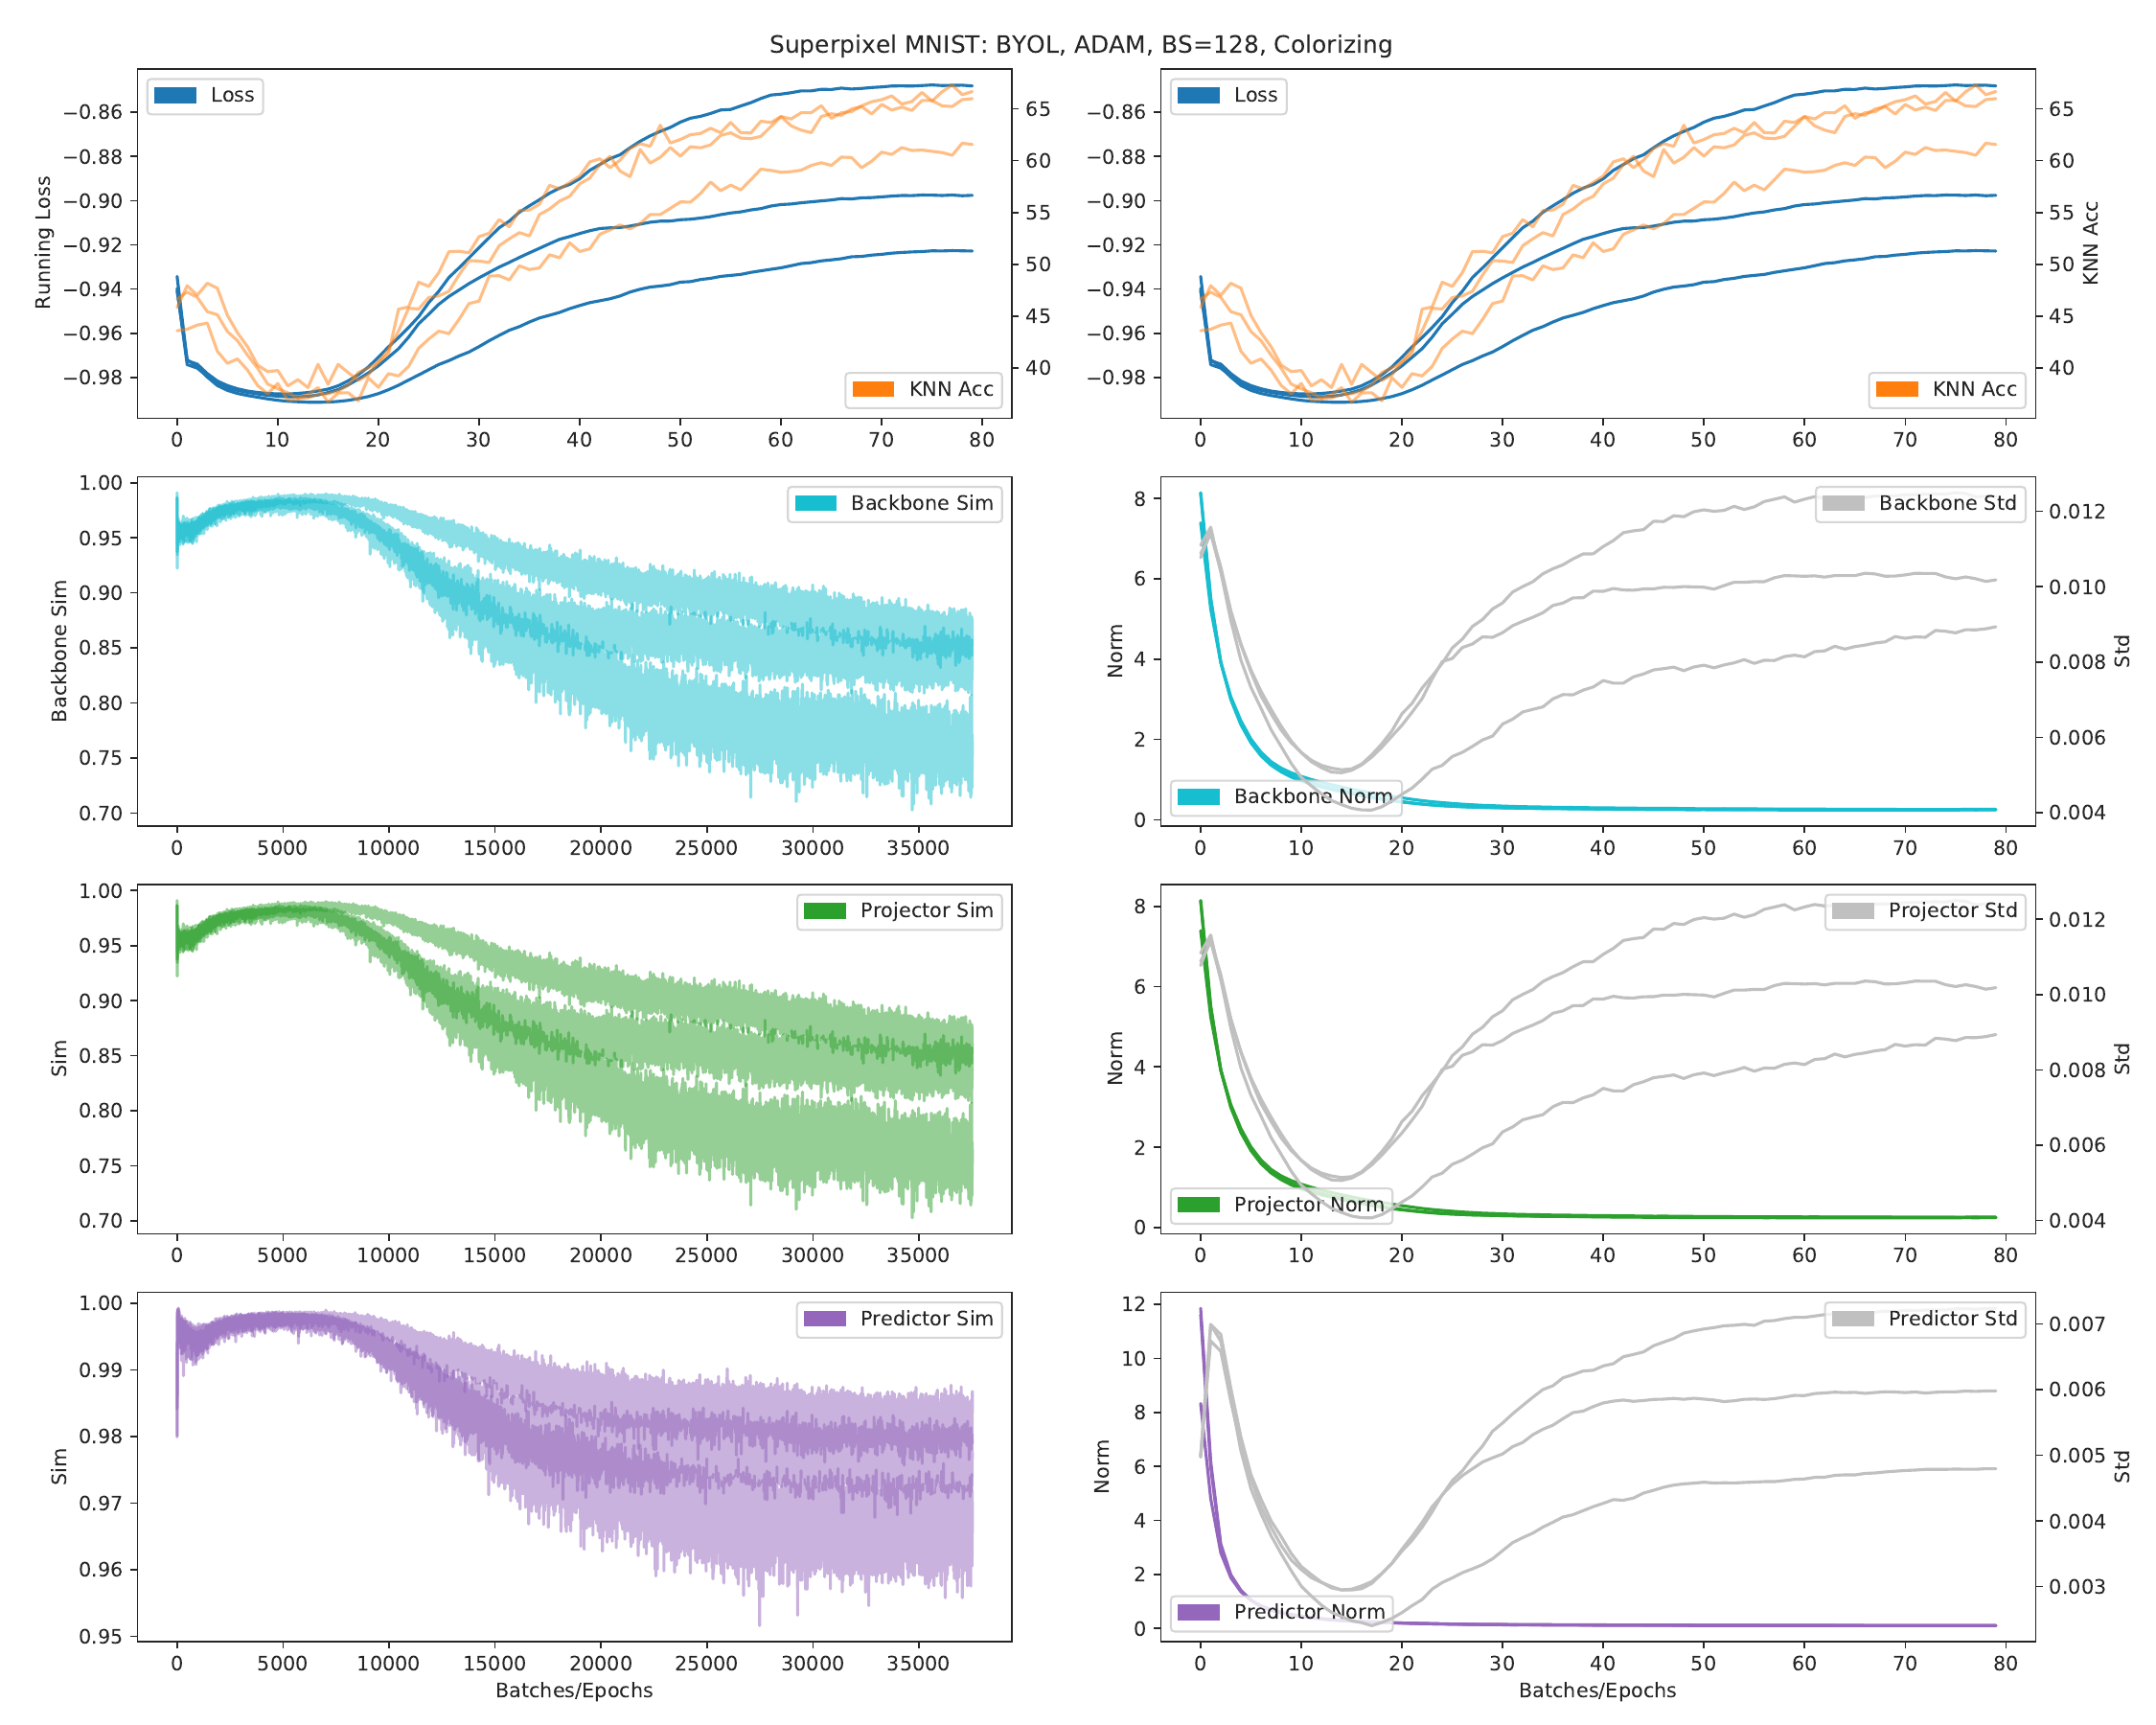}
\caption{BYOL, Colorizing}
\label{fig:byol_color}
\end{figure}

\newpage
\begin{figure}[H]
    \centering
    \includegraphics[width=0.8\textwidth]{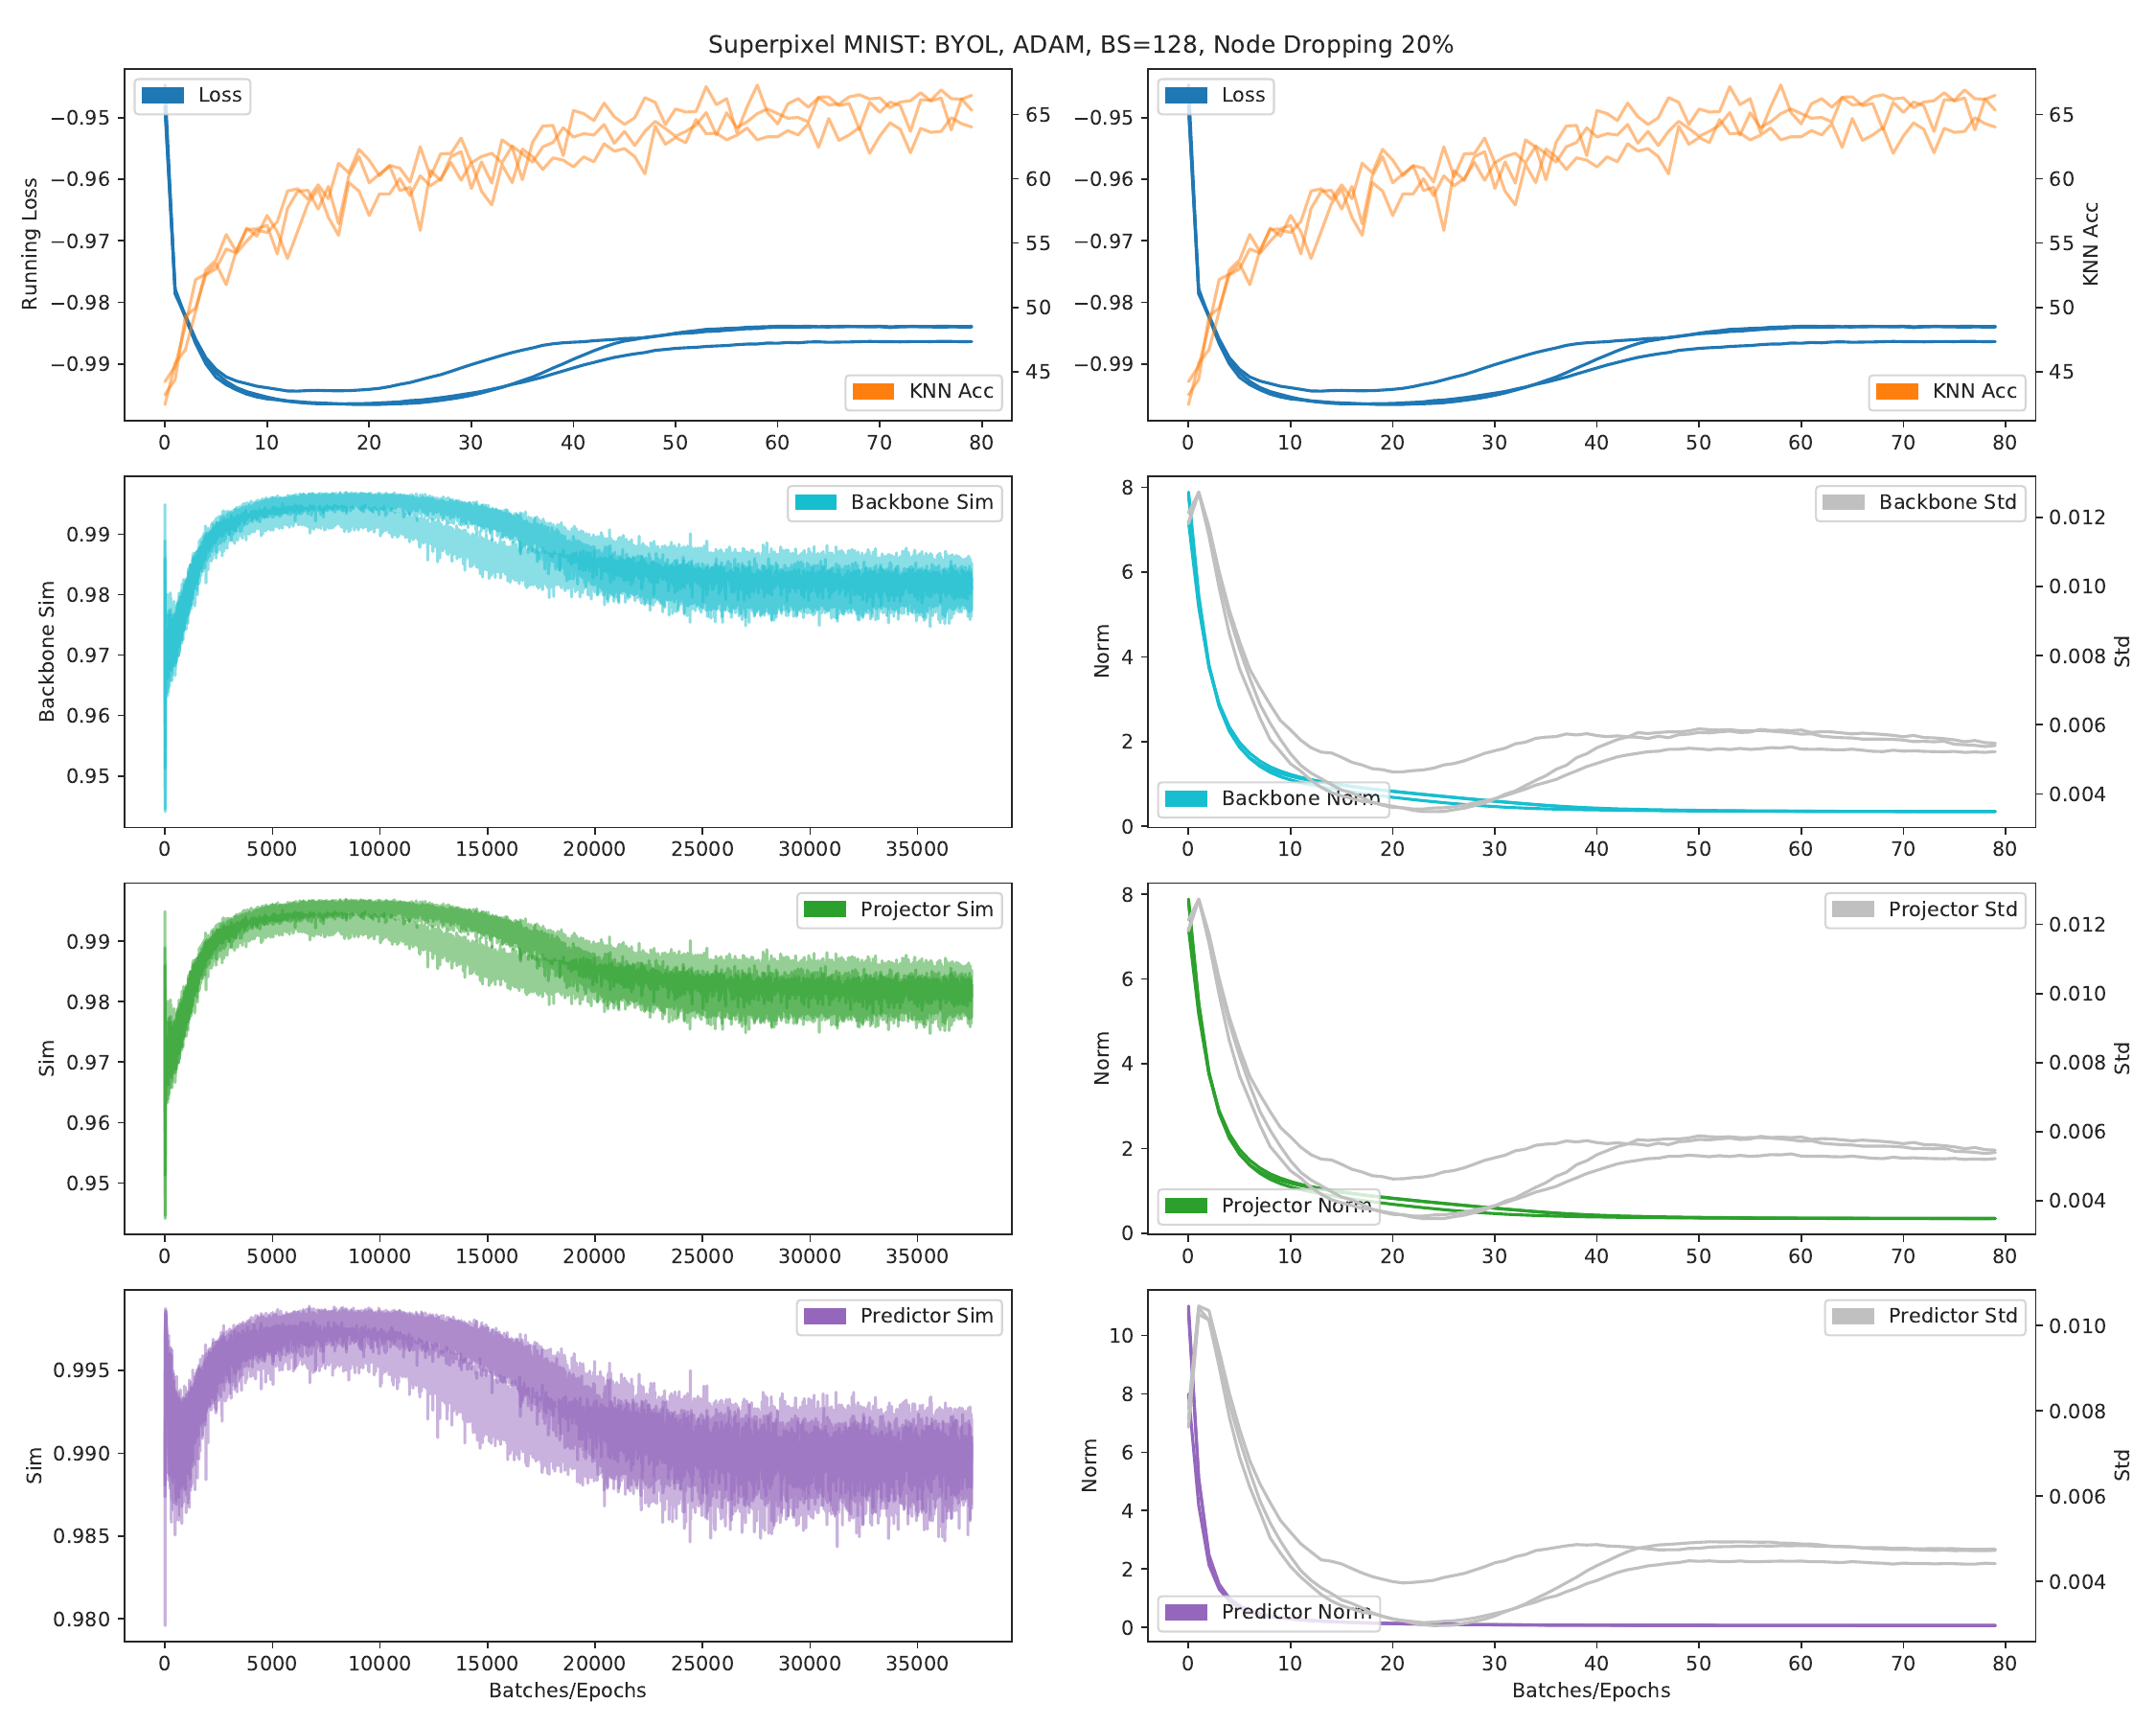}
    \caption{BYOL, Node Dropping 20\%}
    \label{fig:byol_node_20}
\end{figure}

\begin{figure}[H]
    \centering
    \includegraphics[width=0.8\textwidth]{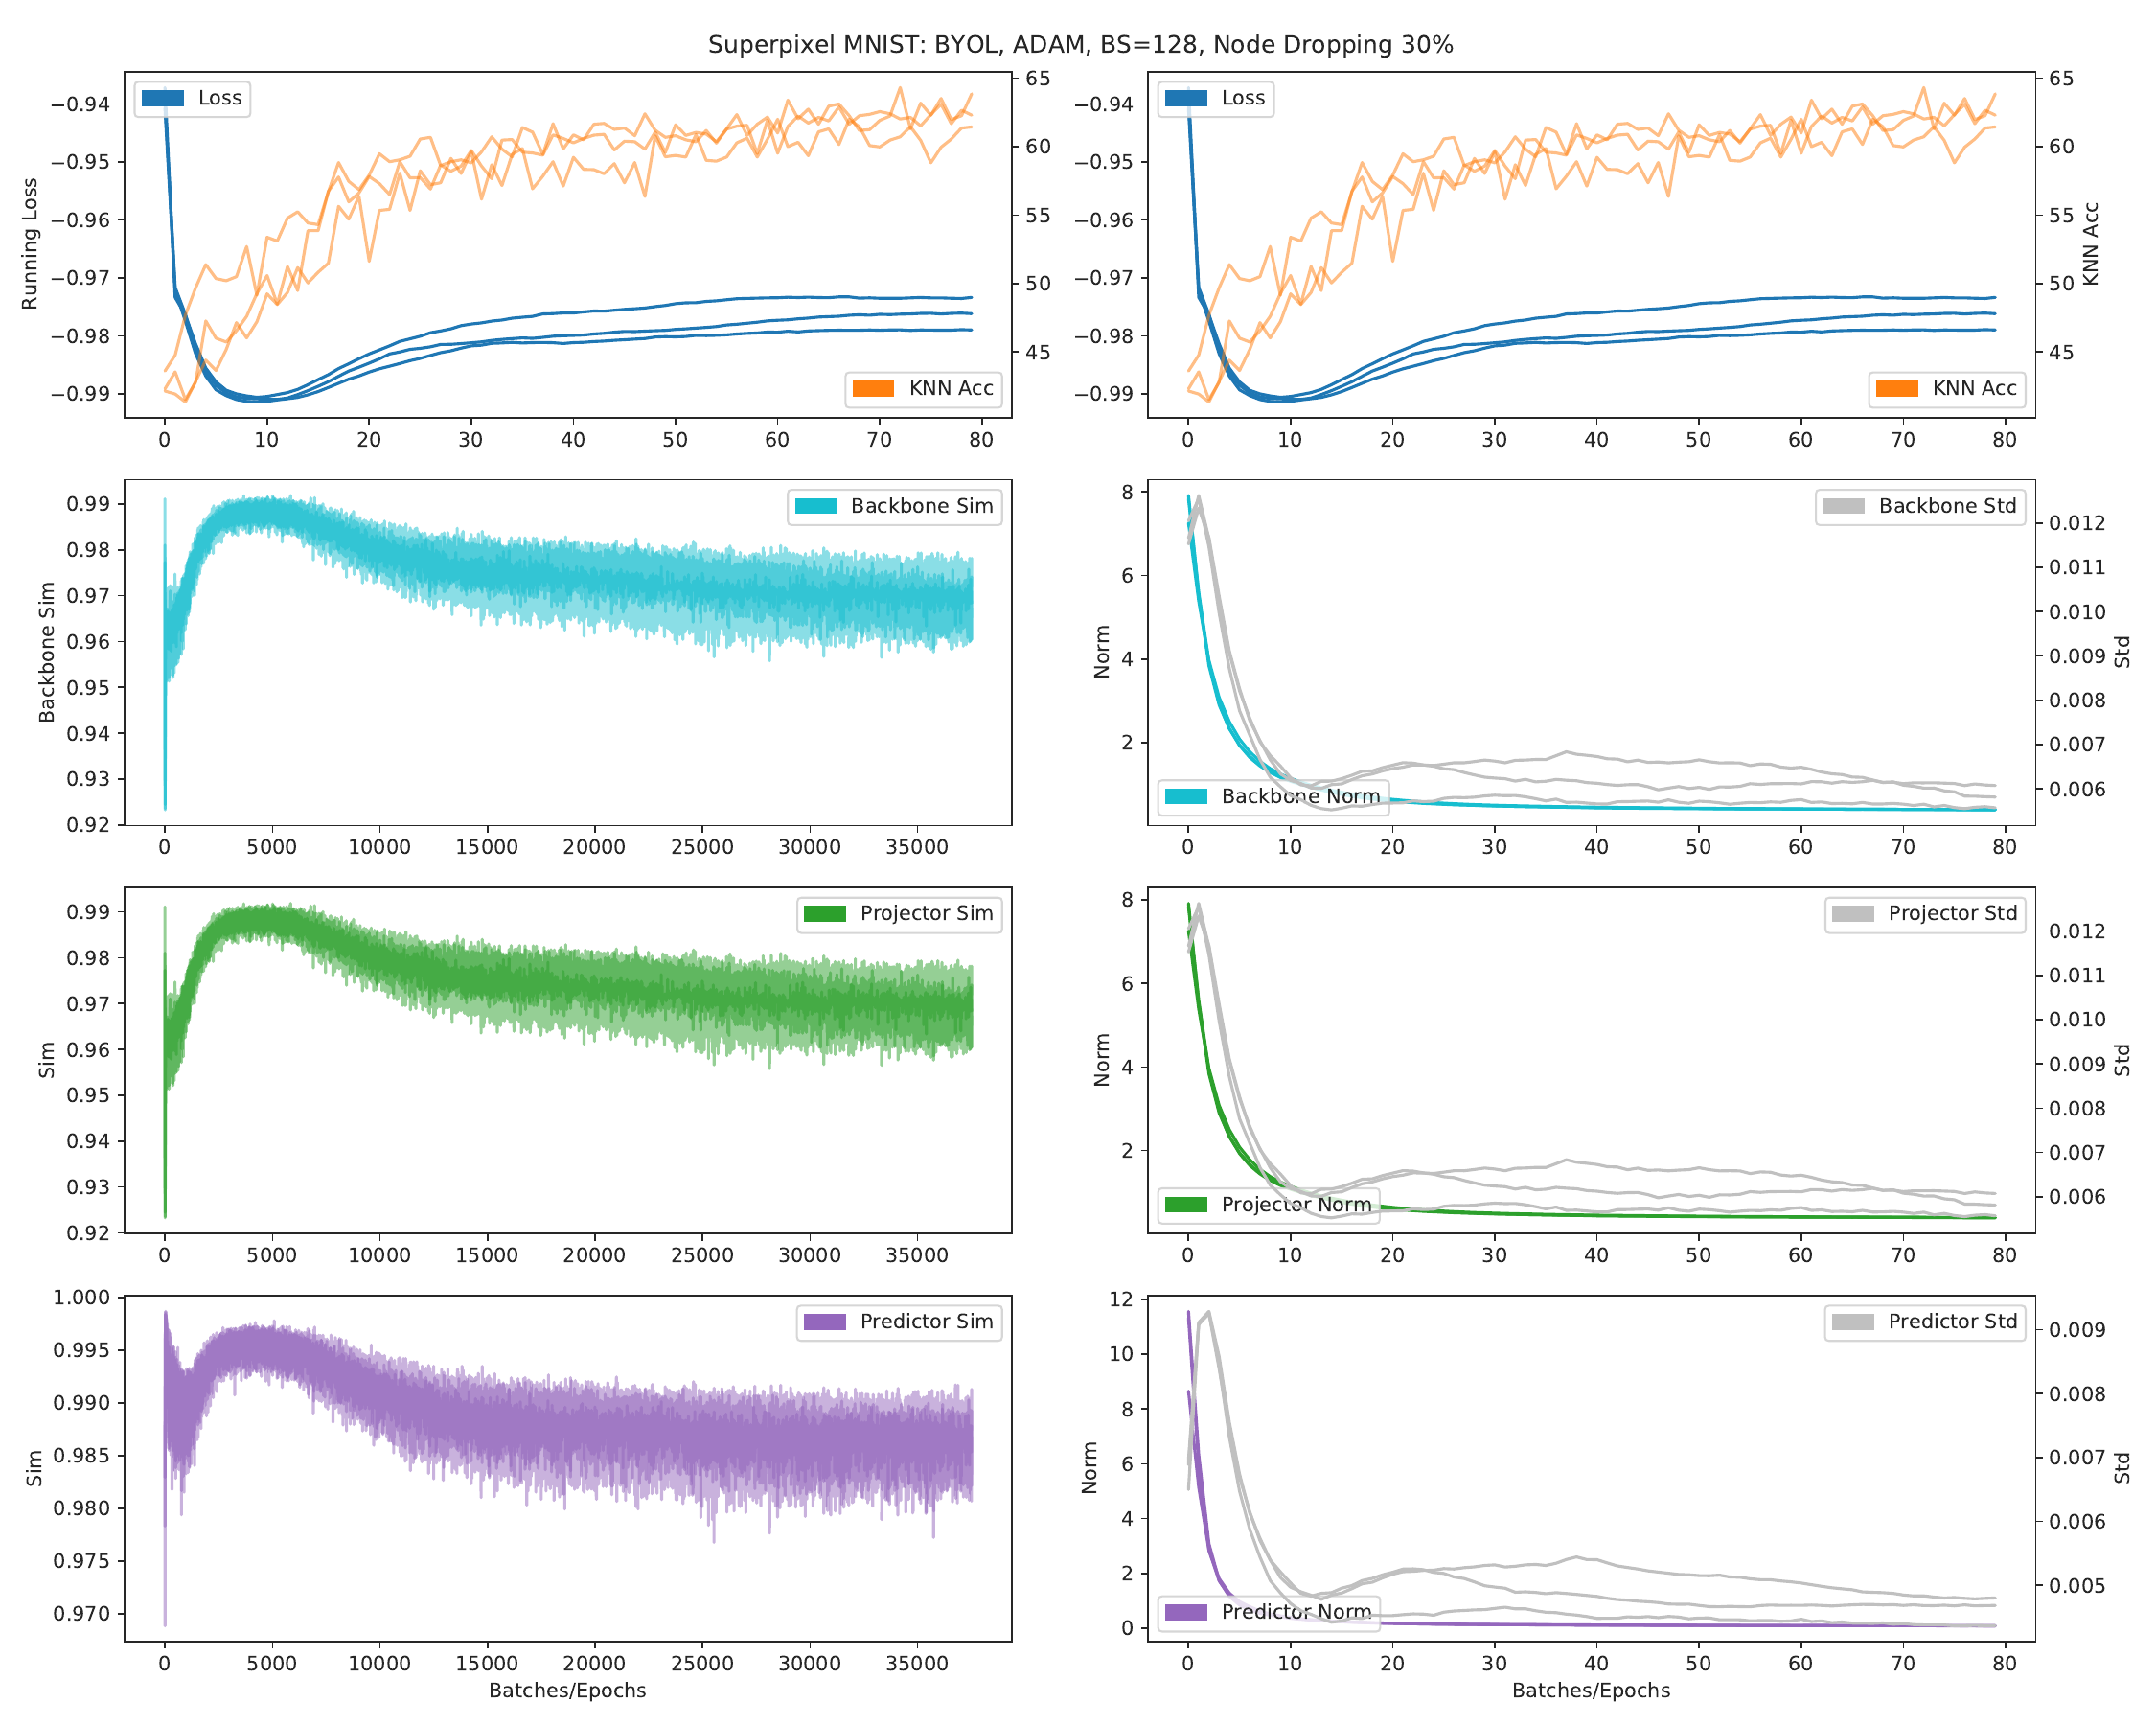}
    \caption{BYOL, Node Dropping 30\%}
    \label{fig:byol_node_30}
\end{figure}

\newpage
\subsection{Understanding the Effects of Augmentations}\label{app_understandingaug}
While many augmentations are used in image classification, it is unclear how such augmentations will effect superpixel graphs and node features. To understand the effects of image augmentations, we use the following procedure. For each sample in the dataset, we compute the structural similarity (\cite{Wang04_SSIM}) between original and augmented images. Then, we convert both the original and augmented images to super-pixel graphs. We compute the cosine similarity between their features, assuming a one-to-one correspondence between nodes. To compute graph similarity, we first compute the Laplacian spectrum, $L$, of both graphs. We find the number of eigenvectors, $k$, needed to cover at least 90\% of the spectrum. Using $k = \min\{k_{orig},k_{aug}\}$, we report $\sum(L_{data}[:k] - L_{aug}[:k])^2$ as a measure of graph similarity. 
 
 In Figures (\ref{fig:app_affine},\ref{fig:app_color},\ref{fig:app_affine_color},\ref{fig:app_horizflip},\ref{fig:app_center_crop}), we plot the structural similarity, feature similarity, weighted eigenvector similarity, and unweighted eigenvector similarity for 10000 samples, given different augmentations. Higher structural similarity and feature similarity indicates more similarity. Lower eigenvector similarity scores indicates more similarity in the graph space. By measuring the effects of augmentations in image, feature and graph space, we are able to better understand the effects of augmentations. For example, we see that the Colorize transformation (Fig. \ref{fig:app_color}) maintains high structural and graph similarity but relatively low feature similarity. Therefore, we expect that label information is preserved both in the image space and the graph space as underlying graph topology has not changed substantially. Center Cropping (Fig. \ref{fig:app_center_crop}) has relatively low structural similarity, and graph similarity. This suggests that task relevant information may be destroyed in the image space as well as graph space.  While the underlying metrics are imperfect, we note this analysis suggests a general approach for evaluating potential augmentations. For example, when working with molecular graphs, similarity coefficients designed for molecular fingerprints (e.g. (Tanimoto, Dice,etc) can be used in lieu of structural similarity.
 
\begin{figure}[t]
    \centering
    \includegraphics[width=0.9\textwidth]{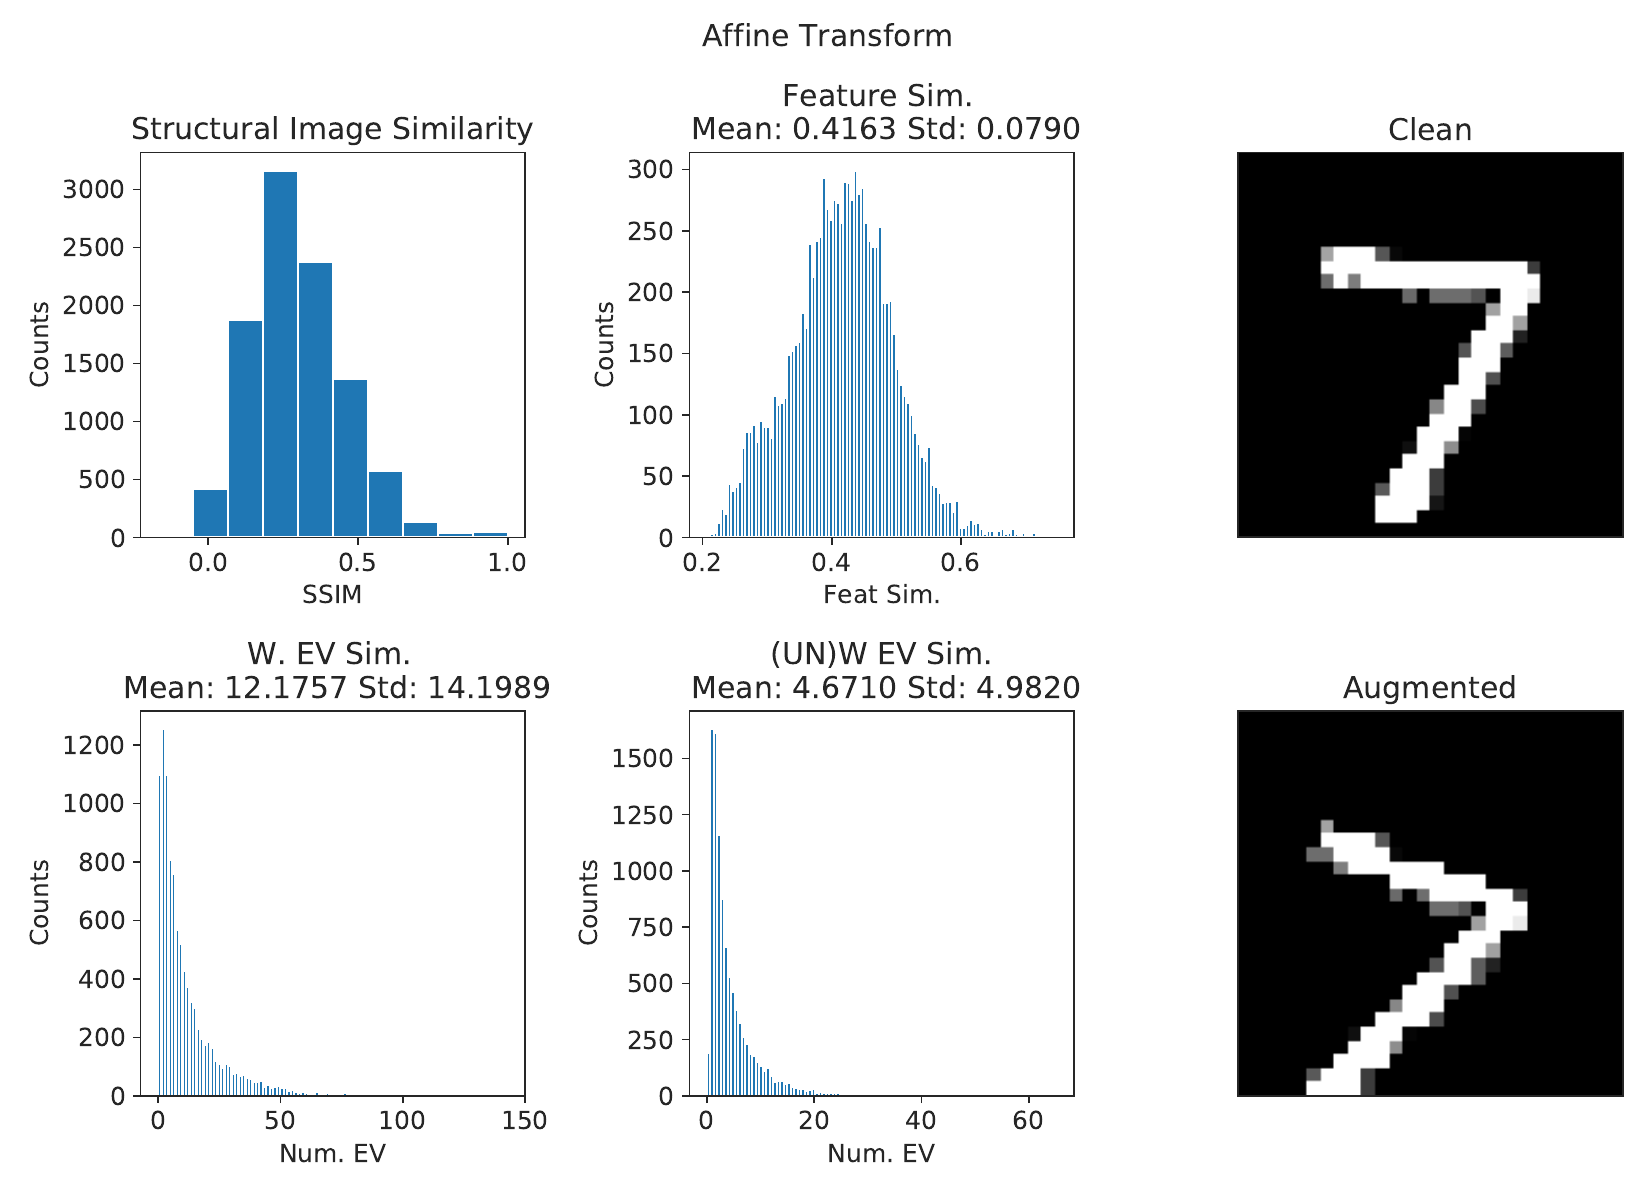}
    \caption{Affine Transformation: Structural image similarity, feature similarity, weighted eigenvector similarity and unweighted eigenvector similarity between original and augmented samples.}
    \label{fig:app_affine}
\end{figure}

\begin{figure}[t]
    \centering
    \includegraphics[width=0.9\textwidth]{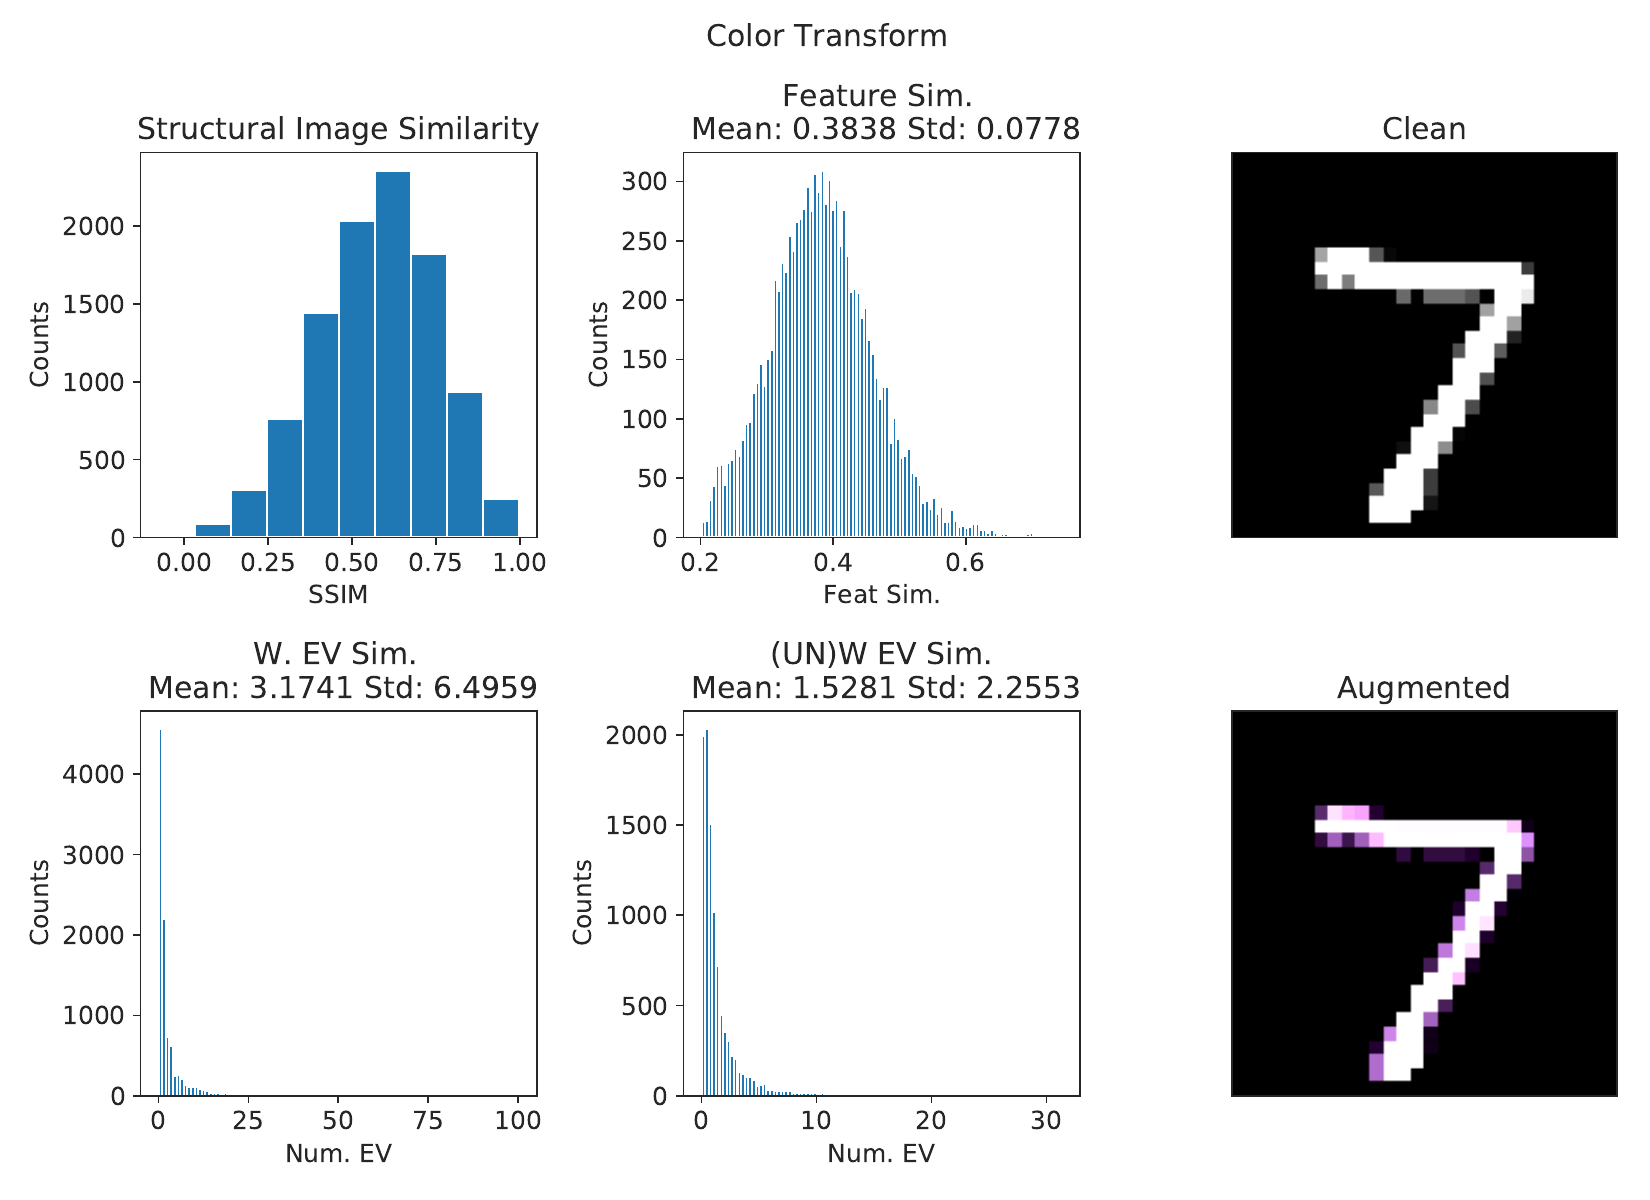}
    \caption{Colorize Transformation: Structural image similarity, feature similarity, weighted eigenvector similarity and unweighted eigenvector similarity between original and augmented samples.}
    \label{fig:app_color}
\end{figure}

\begin{figure}[H]
    \centering
    \includegraphics[width=0.9\textwidth]{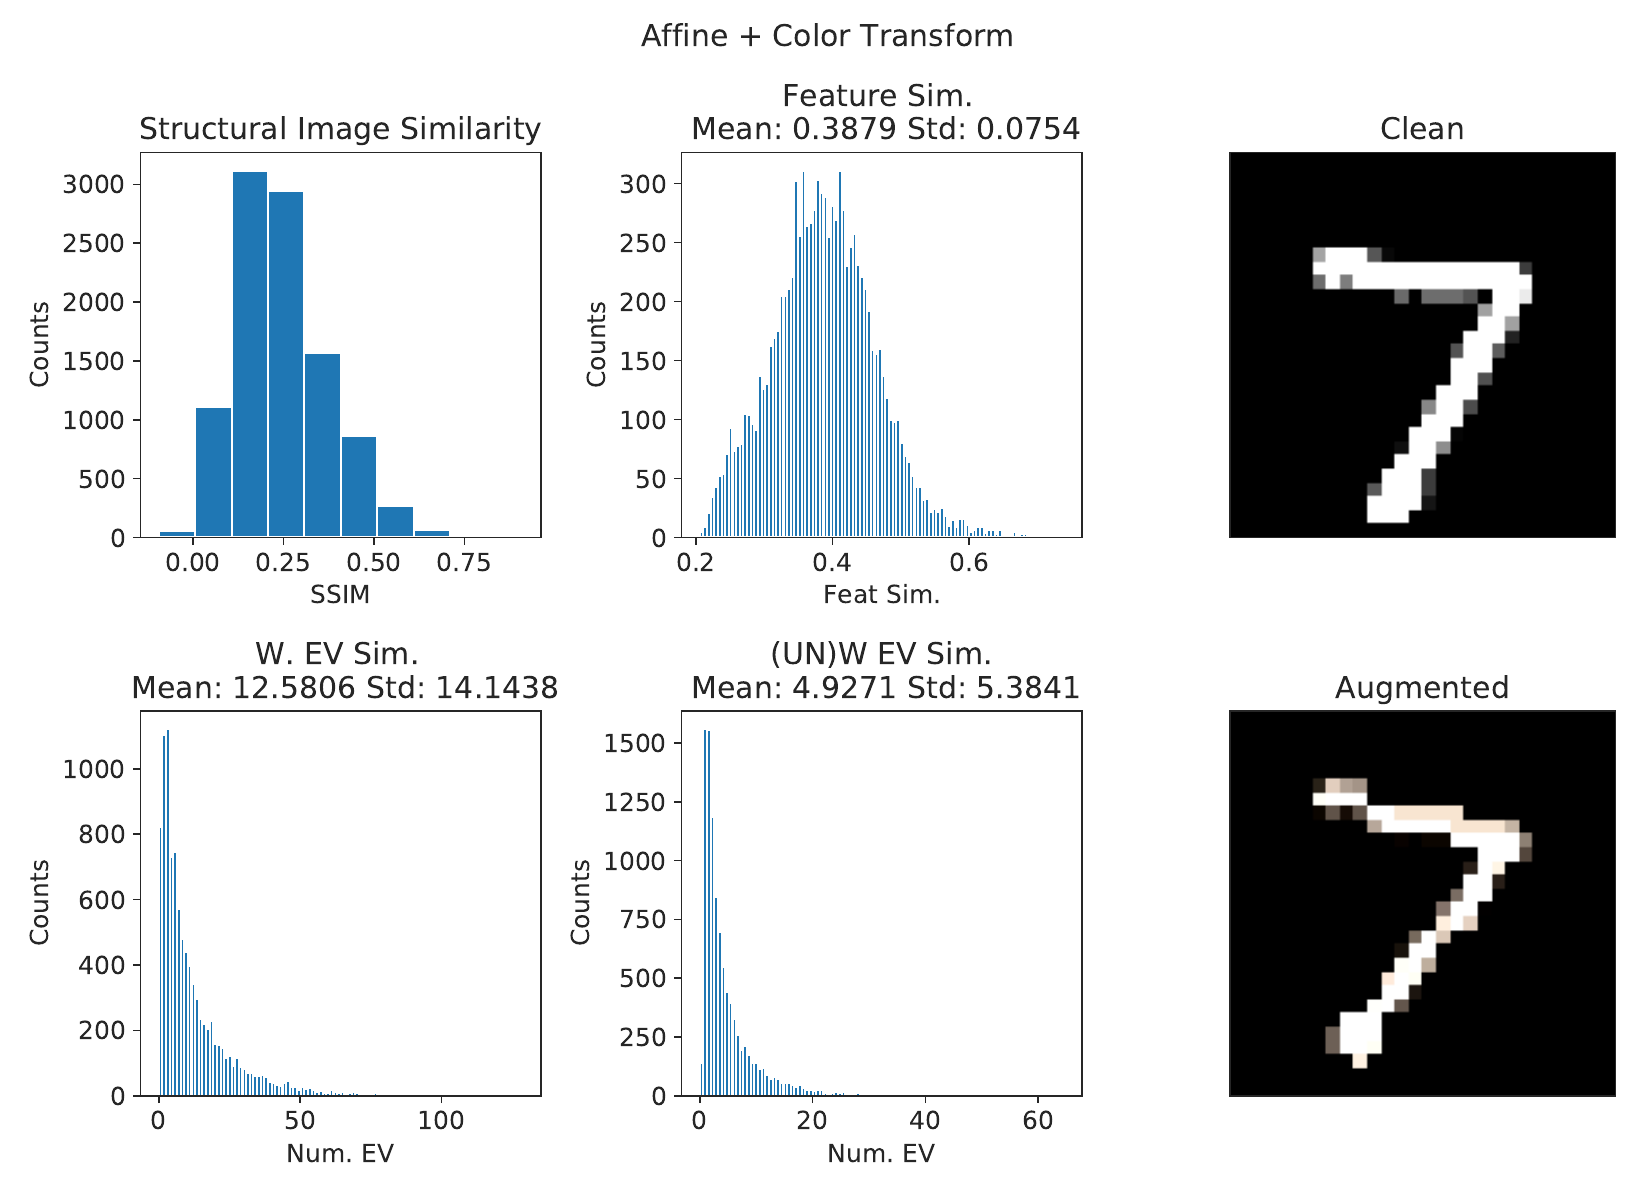}
    \caption{Affine Color Transformation: Structural image similarity, feature similarity, weighted eigenvector similarity and unweighted eigenvector similarity between original and augmented samples.}
    \label{fig:app_affine_color}
\end{figure}

\begin{figure}[t]
    \centering
    \includegraphics[width=0.9\textwidth]{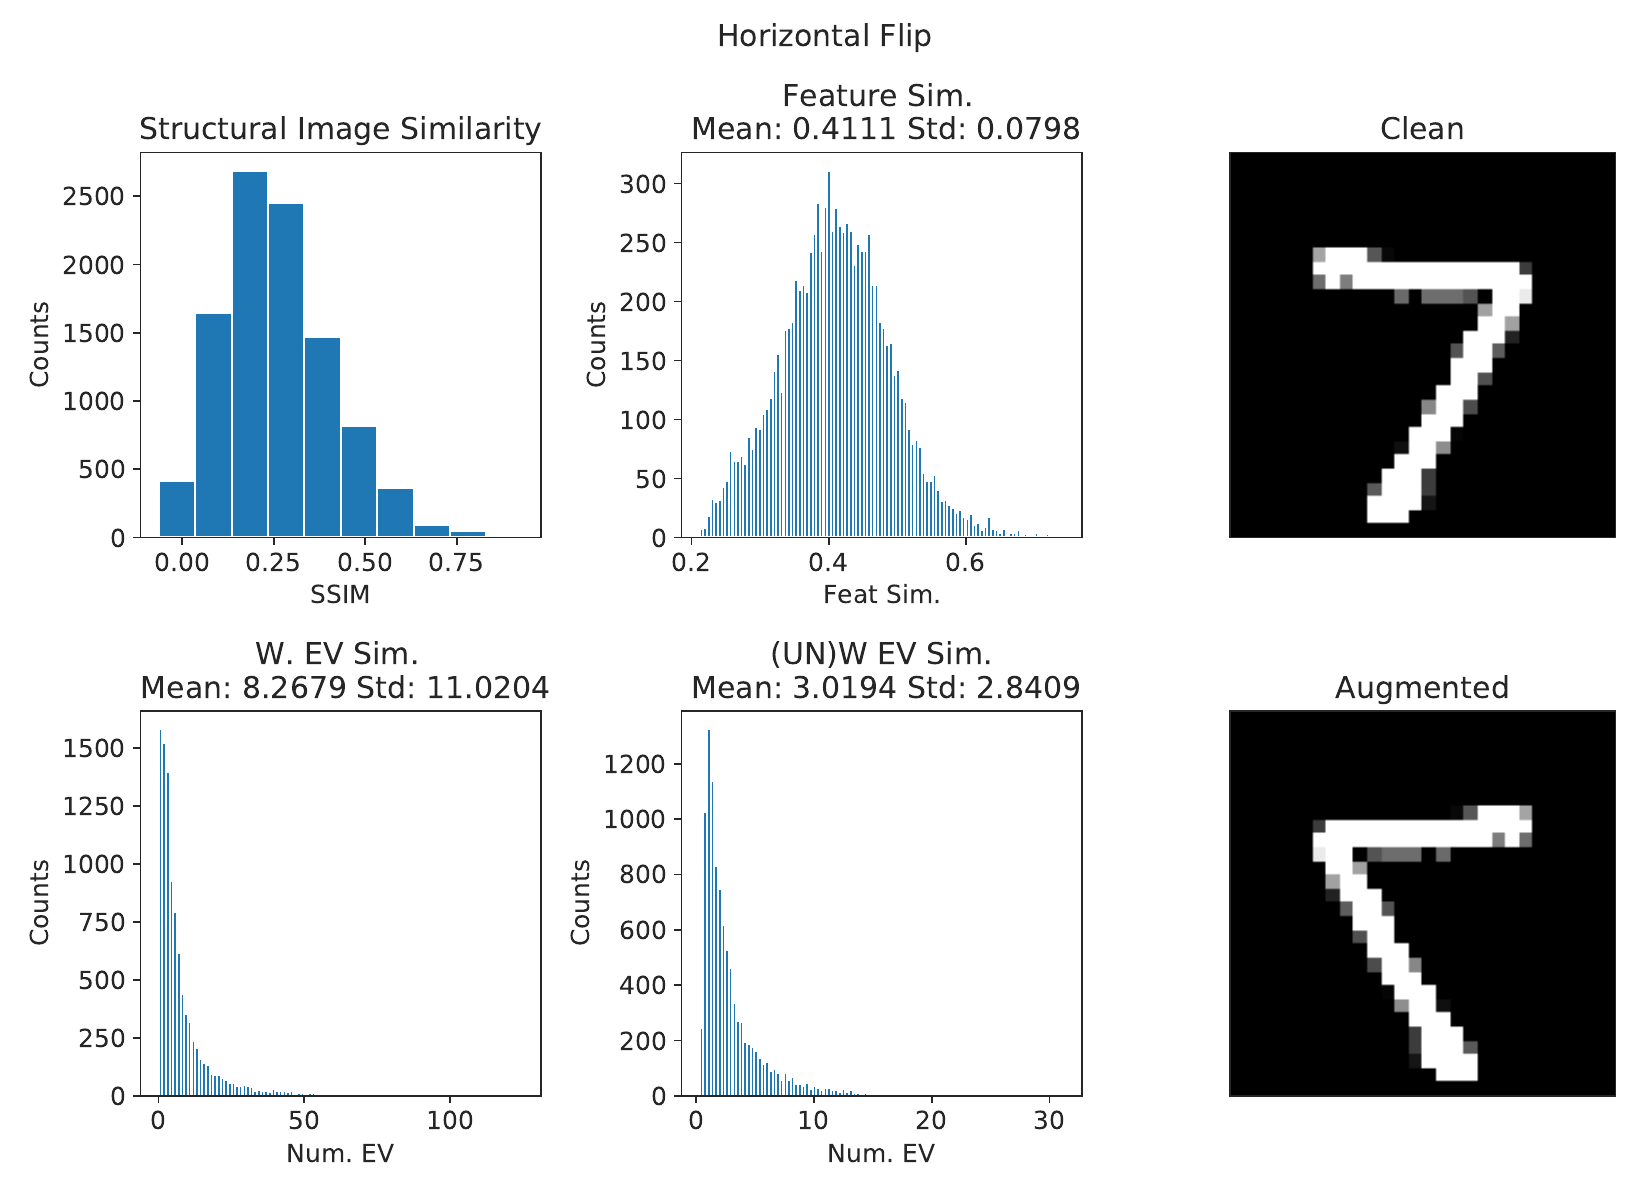}
    \caption{Horizontal Flip Transformation: Structural image similarity, feature similarity, weighted eigenvector similarity and unweighted eigenvector similarity between original and augmented samples.}
    \label{fig:app_horizflip}
\end{figure}

\begin{figure}[t]
    \centering
    \includegraphics[width=0.9\textwidth]{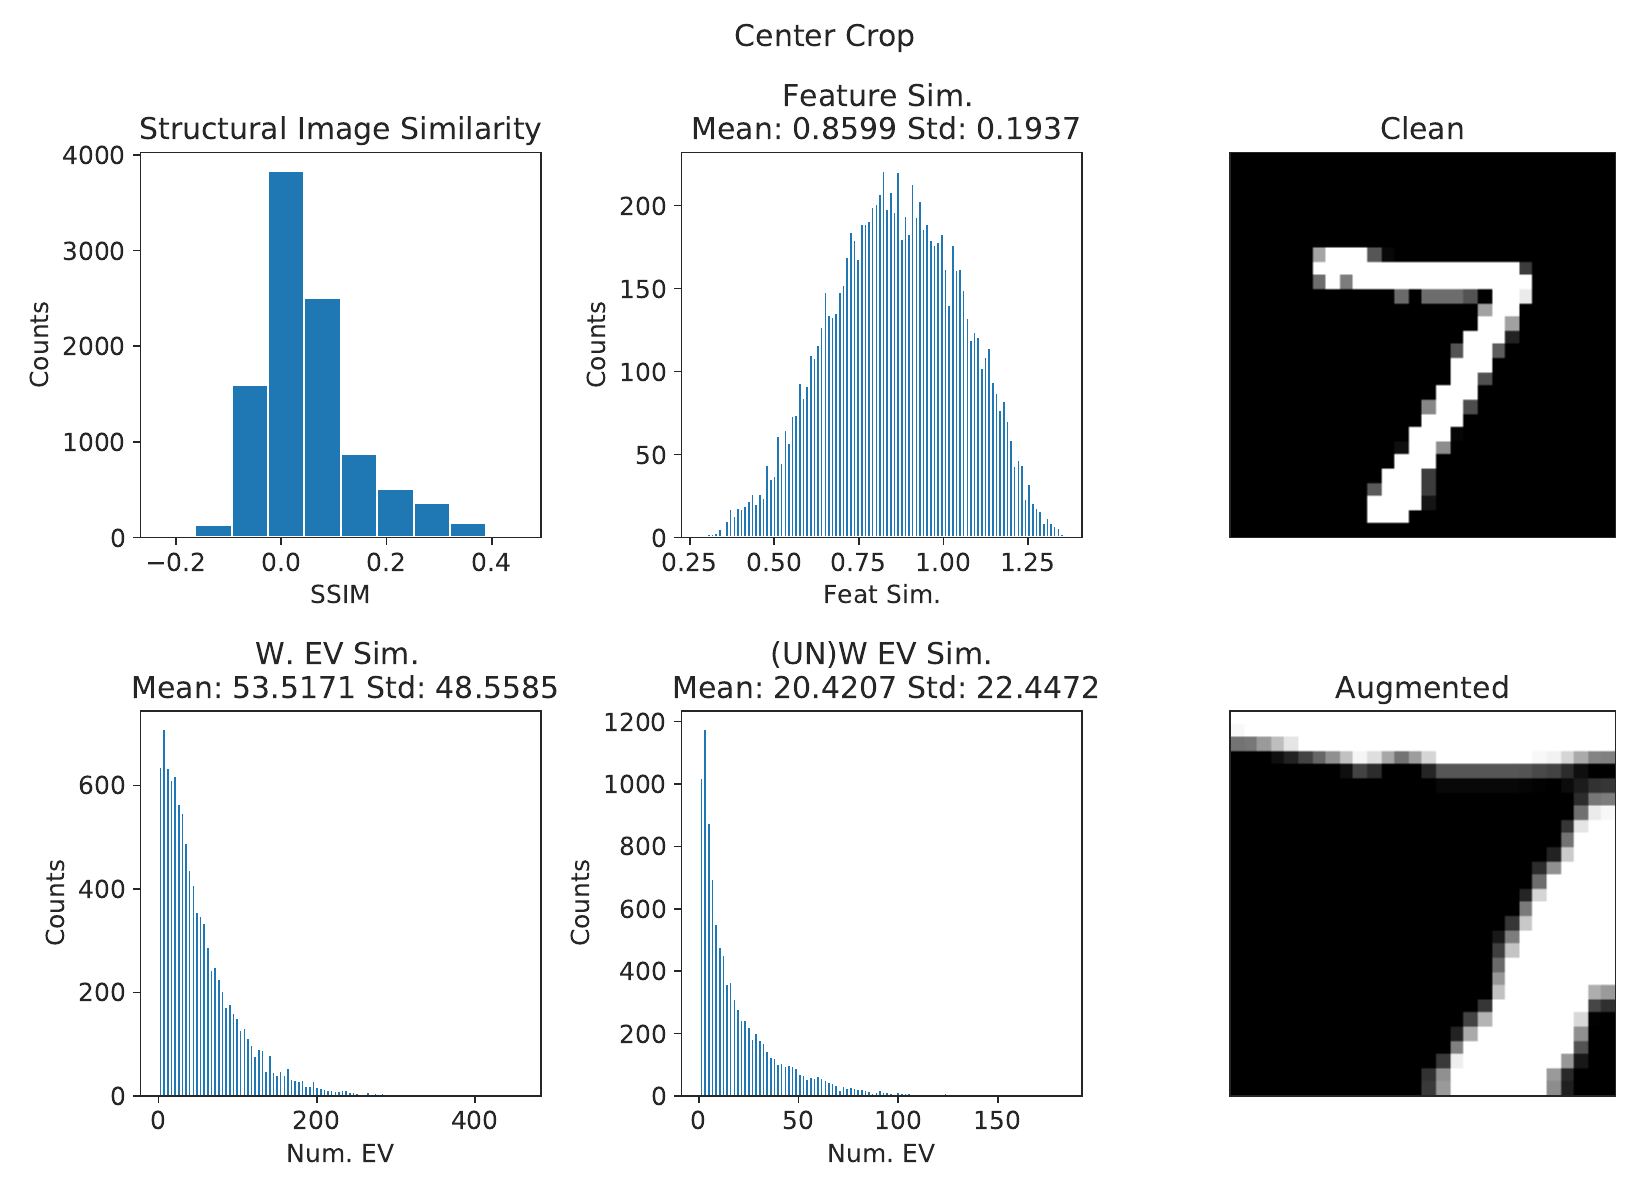}
    \caption{Center Crop Transformation: Structural image similarity, feature similarity, weighted eigenvector similarity and unweighted eigenvector similarity between original and augmented samples.}
    \label{fig:app_center_crop}
\end{figure}

\begin{figure}[t]
    \centering
    \includegraphics[width=0.9\textwidth]{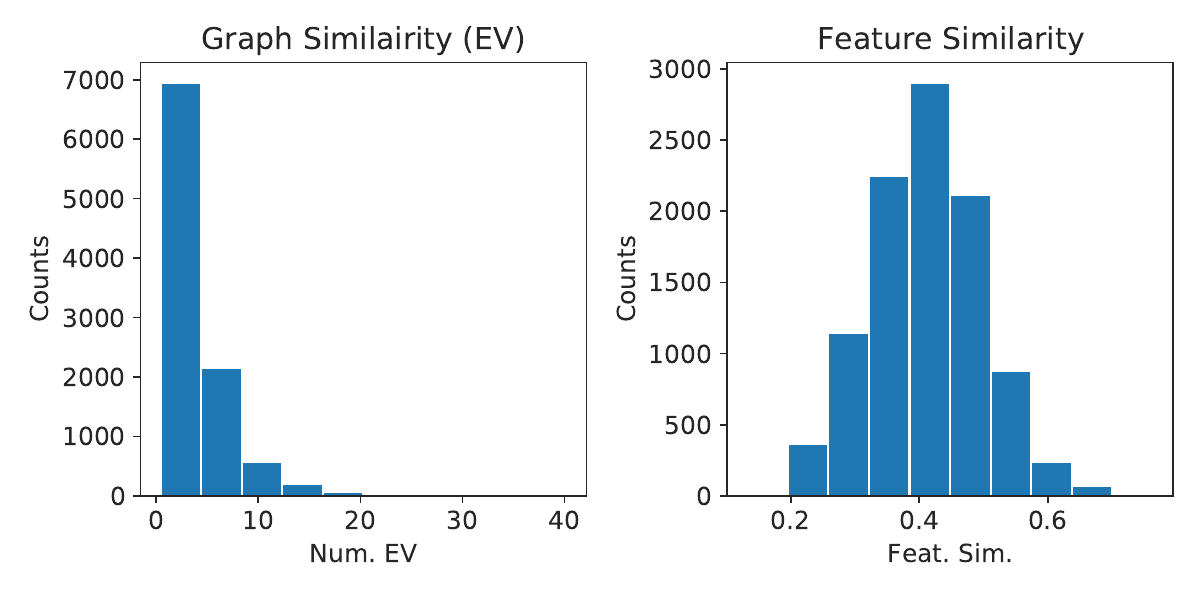}
    \caption{Node Dropping, 20\%: Weighted eigenvector similarity and feature similarity between original and augmented superpixel graphs.}
    \label{fig:app_node_20}
\end{figure}
