# Supplementary material for: Augmentations in Graph Contrastive Learning: Current Methodological Flaws & Towards Better Practices
Source: arXiv:2111.03220 source file (2022-03-11)
Supplement: Supplementary file 3 [file Obs1.tex]

In Sec.~\ref{sec:l1}, we show that domain agnostic graph augmentations are susceptible to destroying task relevant information.

\underline{\smash{Experimental Setup:}} We use the same backbone GIN (\cite{Hu19_HowPowerfulAreGNN}) as InfoGraph (\cite{Sun20_InfoGraph}) and GraphCL (\cite{You20_GraphContrastiveLearning}) when training all dataset but GOSSIPCOP/DEEZER. We use PNA for these datasets as Infograph's loss becomes unstable with GIN. The following training configuration is used: Number of Layers = 3, Learning Rate = 0.01, Number of Epochs = 30, Batch-Size = 32, Optimizer = Adam. Models are trained on a Nvidia Tesla K80 GPU. A batch-norm layer is included between the output of the backbone and cross entropy layer. For augmentations, we follow \cite{You20_GraphContrastiveLearning} and stochastically apply node dropping at 20\% of graph size and subgraph dropping at 20\% of graph size. For GOSSIPCOP, the encoder is based off the implementation in PyTorch Geometric \cite{Fey19_PyG}: 1 GCN Layer, 1 Linear Layer, embedding dimension = 128, Optimizer = Adam, lr = 0.001, Number of Epochs = 25, batch size = 128.
