# Supplementary material for: Augmentations in Graph Contrastive Learning: Current Methodological Flaws & Towards Better Practices
Source: arXiv:2111.03220 source file (2022-03-11)
Supplement: Supplementary file 4 [file Obs2.tex]

In Sec.~\ref{sec:l2}, we show that domain agnostic graph augmentations can lead to weakly discriminative representations, where intra-class and inter-class representational similarity is high.

\underline{\smash{Experimental Setup:}} The following training configuration is used in this experiment, including the additional results below: 3-layer GIN model with hidden dimension, learning rate, and epochs trained of (32, NA, NA) for RAND (Random Initialization), (512,0.001,20) for InfoGraph (\cite{Sun20_InfoGraph}), and (32,0.01,20)  for GraphCL (\cite{You20_GraphContrastiveLearning}). The Adam optimizer (\cite{Kingma14_Adam}) is used to train all models. A Nvidia Tesla K80 GPU is used to train all models. Results for MVGRL (\cite{Hassani20_MVGRL}) are not included as we consistently witnessed Out-Of-Memory errors during training (we use a 12-GB GPU). Results are reported over 3 seeds. Note, for the Deezer and Github datasets, we used PNA convolutional layers instead of GIN as training was unstable with GIN.

\underline{\smash{Additional Results:}} Fig.~\ref{fig:app_rand_proteins} includes additional results for PROTEINS, NCI1 and DD datasets. Given that the cosine similarity between positive samples is directly maximized by the contrastive loss, the low representational similarity indicates the model has not learned well.

\begin{figure}[h!]
\centering
        \begin{subfigure}[b]{0.3\columnwidth}
                \centering
             \includegraphics[width=\columnwidth]{APPENDIX/heatmaps/RAND_PROTEINS.pdf}
                \caption{RAND: PROT. \\ $(73.678 \pm 6.91)$}
                \label{fig:app_rand_proteins}
        \end{subfigure}%
        \hfill
        \begin{subfigure}[b]{0.3\columnwidth}
                \centering \includegraphics[width=\columnwidth]{APPENDIX/heatmaps/RAND_NCI1.pdf}
                \caption{RAND: NCI1 \\ $(70.65 \pm 1.99)$}
                \label{fig:app_rand_nci1}
        \end{subfigure}%
        \hfill
        \begin{subfigure}[b]{0.3\columnwidth}
                \centering \includegraphics[width=\columnwidth]{APPENDIX/heatmaps/RAND_DD.pdf}
                \caption{RAND: DD \\ $(74.52 \pm 9.12)$}
                \label{fig:app_rand_dd}
        \end{subfigure}
        \label{fig:modecollapse_rand}
\centering
        \begin{subfigure}[b]{0.3\columnwidth}
                \centering
             \includegraphics[width=\columnwidth]{APPENDIX/heatmaps/GRAPHCL_PROTEINS.pdf}
                \caption{GraphCL: PROT. \\ ($73.49\pm0.33$)}
                \label{fig:app_graphcl_proteins}
        \end{subfigure}%
        \hfill
        \begin{subfigure}[b]{0.3\columnwidth}
                \centering \includegraphics[width=\columnwidth]{APPENDIX/heatmaps/GRAPHCL_NCI1.pdf}
                \caption{GraphCL: NCI1\\ ($78.16 \pm 0.51$)}
                \label{fig:app_graphcl_nci1}
        \end{subfigure}%
        \hfill
        \begin{subfigure}[b]{0.3\columnwidth}
                \centering \includegraphics[width=\columnwidth]{APPENDIX/heatmaps/GRAPHCL_DD.pdf}
                \caption{GraphCL: DD \\ $(79.54\pm 0.698)$}
                \label{fig:app_graphcl_dd}
        \end{subfigure}
        \label{fig:modecollapse_graphcl}
\centering
        \begin{subfigure}[b]{0.3\columnwidth}
                \centering
             \includegraphics[width=\columnwidth]{APPENDIX/heatmaps/INFOGRAPH_PROTEINS.pdf}
                \caption{InfoGr: PROT. \\ $(73.225 \pm 0.36)$}
                \label{fig:app_infograph_proteins}
        \end{subfigure}%
        \hfill
        \begin{subfigure}[b]{0.3\columnwidth}
                \centering \includegraphics[width=\columnwidth]{APPENDIX/heatmaps/INFOGRAPH_NCI1.pdf}
                \caption{InfoGraph: NCI1 \\ $(73.58 \pm 0.16)$}
                \label{fig:app_infograph_nci1}
        \end{subfigure}%
        \hfill
        \begin{subfigure}[b]{0.3\columnwidth}
                \centering \includegraphics[width=\columnwidth]{APPENDIX/heatmaps/INFOGRAPH_DD.pdf}
                \caption{InfoGraph: DD \\ $(69.41 \pm  0.58)$}
                \label{fig:app_infograph_dd}
        \end{subfigure}
        \label{fig:modecollapse_infograph}
    \caption{\textbf{Representational Similarity: } In addition to MUTAG (\autoref{fig:modecollapse}), we provide results on PROTEINS, NCI1 and DD. Random inductive bias is most noticeable on MUTAG and PROTEINS. Note that the intra-class similarity can be low for GraphCL and InfoGraph.}
\end{figure}
